# Supplementary material for: Extending numerical simulations in SIMPSON: Electron paramagnetic resonance, dynamic nuclear polarisation, propagator splitting, pulse transients, and quadrupolar cross terms
Source: arXiv:2602.15793 ancillary file (2026-02-17)
Supplement: Supplementary file 1 [file Simpson6_SI.pdf]

# Supplementary material:
# Extending numerical simulations in SIMPSON: Electron paramagnetic resonance, dynamic nuclear polarisation, propagator splitting, pulse transients, and quadrupolar cross terms

David L. Goodwin *[1], José P. Carvalho[1], Anders B. Nielsen[1], Nino Wili[1], Thomas Vosegaard †[1], Zdeněk Tošner ‡[2], and Niels Chr. Nielsen §[1]

[1]Interdisciplinary Nanoscience Center (iNANO) and Department of Chemistry, Aarhus University, Gustav Wieds Vej 14, DK-8000 Aarhus C, Denmark
[2]Department of Chemistry, Faculty of Science, Charles University in Prague, Hlavova 8, CZ-128 43, Czech Republic

February 2026

## Contents

**1 ESEEM example** **2**

**2 Pulsed DNP examples** **4**

**3 Gradient-free optimisation** **8**

**4 Optimisation of SORDOR pulse** **11**

**5 High accuracy splittings** **20**

**6 Optimal control with pulse transients** **36**

**7 Quadrupolar second-order cross-terms** **81**

**8 Calculation of tm-SPICE pulses** **83**

*ORCID: 0000-0001-9423-1106, email: david.goodwin@inano.au.dk
†ORCID: 0000-0001-5414-4550, email: tv@chem.au.dk
‡ORCID: 0000-0003-2741-9154, email: zdenek.tosner@natur.cuni.cz
§ORCID: 0000-0003-2978-4366, email: ncn@chem.au.dk

# 1 ESEEM example

Two-pulse ESEEM (main text figure 2B)

```
# ==================================================================
# SIMPSON 2p ESEEM example, for a single crystal and ideal pi-pulse
# ==================================================================

spinsys {
    channels    e
    nuclei      e 1H
    gtensor     1 0 0 0 0 0 0
    hyperfine   1 2 0 1e6 0 45 0
}

par {
    proton_frequency    14.8e6
    start_operator      I1x
    detect_operator     I1x
    method              DNPframe
    np                  256
    sw                  250
}

proc pulseq {} {
    global par

    # set delay incr., max. delay, then loop over par(np)
    set dt 0.004
    set T [expr $par(np)*$dt]
    for {set tau 0} {$tau<$T} {set tau [expr $tau+$dt]} {
        reset
        delay   $tau
        pulseid 0.005 100e6 x
        delay   $tau
        acq
    }
}

proc main {} { fsave [fsimpson] eseem_2pulse.fid }
```

Three-pulse ESEEM (main text Figure 2C)

```
# ==================================================================
# SIMPSON 3p ESEEM example, powder, offset averaging, ideal pulses
# ==================================================================

spinsys {
    channels    e
    nuclei      e 1H
    gtensor     1 1 0 0 0 0 0
    hyperfine   1 2 0 1e6 0 45 0
}

par {
    proton_frequency    14.8e6
    start_operator      I1x
    detect_operator     I1x
    method              DNPframe
    np                  256
    sw                  250
    crystal_file        rep144
    averaging_file      gtensor_1_iso_30MHz.ave
}

proc pulseq {} {
    global par

    matrix set 1 coherence {{0 1} {0 -1} {0 0}}

    # set delay incr., max. delay, then loop over par(np)
    set dt 0.004
    set T [expr $par(np)*$dt]
    for {set tau 0} {$tau<$T} {set tau [expr $tau+$dt]} {
```

```
        reset
        delay   0.104
        pulseid 0.0025 100e6 x
        filter  1
        delay   $tau
        pulseid 0.0025 100e6 x
        delay   0.104
        acq
    }
}

proc main {} { fsave [fsimpson] eseem_3pulse.fid }
```

For realistic, non-ideal pulses, the `pulseid` should be changed for `pulse`. The range of offsets is defined in the averaging file `gtensor_1_iso_30MHz.ave`

```
gtensor_1_iso   weight
15000000.00     0.01639344
14500000.00     0.01639344
14000000.00     0.01639344
13500000.00     0.01639344
13000000.00     0.01639344
12500000.00     0.01639344
12000000.00     0.01639344
11500000.00     0.01639344
11000000.00     0.01639344
10500000.00     0.01639344
10000000.00     0.01639344
9500000.00      0.01639344
9000000.00      0.01639344
8500000.00      0.01639344
8000000.00      0.01639344
7500000.00      0.01639344
7000000.00      0.01639344
6500000.00      0.01639344
6000000.00      0.01639344
5500000.00      0.01639344
5000000.00      0.01639344
4500000.00      0.01639344
4000000.00      0.01639344
3500000.00      0.01639344
3000000.00      0.01639344
2500000.00      0.01639344
2000000.00      0.01639344
1500000.00      0.01639344
1000000.00      0.01639344
500000.00       0.01639344
0.00            0.01639344
-500000.00      0.01639344
-1000000.00     0.01639344
-1500000.00     0.01639344
-2000000.00     0.01639344
-2500000.00     0.01639344
-3000000.00     0.01639344
-3500000.00     0.01639344
-4000000.00     0.01639344
-4500000.00     0.01639344
-5000000.00     0.01639344
-5500000.00     0.01639344
-6000000.00     0.01639344
-6500000.00     0.01639344
-7000000.00     0.01639344
-7500000.00     0.01639344
-8000000.00     0.01639344
-8500000.00     0.01639344
-9000000.00     0.01639344
-9500000.00     0.01639344
-10000000.00    0.01639344
-10500000.00    0.01639344
-11000000.00    0.01639344
-11500000.00    0.01639344
-12000000.00    0.01639344
-12500000.00    0.01639344
-13000000.00    0.01639344
```

```
-13500000.00    0.01639344
-14000000.00    0.01639344
-14500000.00    0.01639344
-15000000.00    0.01639344
```

# 2 Pulsed DNP examples

In all calculations within this chapter, the same spin system is used, defined in the `DNP_sys_1.spinsys` containing:

```
spinsys {
    channels    e
    nuclei      e 1H
    gtensor     1 0 0 0 0 0 0
    hyperfine   1 2 0 1.0e+6 0 45 0
}
```

Examining bandwidth of NOVEL (main text Figure 3B, blue curve)

```
# spinsys defined in an external file
source DNP_sys_1.spinsys

par {
    proton_frequency    14.8e+6
    crystal_file        rep2000
    start_operator      I1x
    detect_operator     -I2z
    method              DNPframe
    sw                  1e9
    np                  1
    conjugate_fid       false
}

proc pulseq {} {
    reset
    pulse   0.8 14.8e+6 180
    acq
}

proc main {} {
    set fid [open novel_bandwidth.dat w]
    # loop over offsets
    for {set g -60e6} {$g<=60e6} {set g [expr $g+1e5]} {
        set f [fsimpson [list [list gtensor_1_iso $g]]]
        puts "[format "%.0f" $g] [findex $f 1 -re]"
        puts $fid "[format "%.0f" $g] [findex $f 1 -re]"
        funload $f
    }
    close $fid
}
```

Examining bandwidth of BEAM (main text Figure 3B, red curve)

```
# spinsys defined in an external file
source DNP_sys_1.spinsys

par {
    proton_frequency    14.8e+6
    crystal_file        rep2000
    start_operator      I1x
    detect_operator     -I2z
    method              DNPframe
    sw                  1e9
    np                  1
    conjugate_fid       false
}

proc pulseq {} {
    reset
    pulse   28.0e-3 32e+6   0
    pulse   31.6e-3 32e+6 180
```

```
    store   1
    reset
    prop    1 31
    acq
}

proc main {} {
    set fid [open beam_bandwidth.dat w]
    # loop over offsets
    for {set g -60e6} {$g<=60e6} {set g [expr $g+1e5]} {
        set f [fsimpson [list [list gtensor_1_iso $g]]]
        puts "[format "%.0f" $g] [findex $f 1 -re]"
        puts $fid "[format "%.0f" $g] [findex $f 1 -re]"
        funload $f
    }
    close $fid
}
```

Examining bandwidth of PLATO (main text Figure 3B, green curve)

```
# spinsys defined in an external file
source DNP_sys_1.spinsys

par {
    proton_frequency    14.8e+6
    crystal_file        rep2000
    start_operator      I1x
    detect_operator     -I2z
    method              DNPframe
    sw                  1e9
    np                  1
    conjugate_fid       false
}


proc pulseq {} {
    global duration shp Nrep
    reset
    pulse_shaped  $duration $shp
    store         1
    reset
    prop          1 $Nrep
    acq
}

proc main {} {
    global duration shp Nrep
    # load appropriate pulse shape (5ns discretisation)
    set shp             [load_shape plato.shp]
    set duration        [expr 0.005*[shape_len $shp]]
    set Nrep            15

    set fid [open plato_bandwidth.dat w]
    # loop over offsets
    for {set g -60e6} {$g<=60e6} {set g [expr $g+1e5]} {
        set f [fsimpson [list [list gtensor_1_iso $g]]]
        puts "[format "%.0f" $g] [findex $f 1 -re]"
        puts $fid "[format "%.0f" $g] [findex $f 1 -re]"
        funload $f
    }
    close $fid
}
```

The PLATO block is defined using a shaped pulse stored as a text file `plato.shp`

```
9310000     0
20360000    0
32000000    0
9290000     180
32000000    180
32000000    180
32000000    180
```

```
7860000     180
32000000    0
32000000    0
32000000    180
32000000    180
32000000    180
28040000    180
32000000    180
32000000    180
8600000     0
32000000    0
32000000    0
32000000    0
32000000    180
6940000     180
32000000    0
32000000    0
```

Examining bandwidth of cRW-OPT1 (main text Figure 3B, purple curve)

```
# spinsys defined in an external file
source DNP_sys_1.spinsys

par {
    proton_frequency    14.8e+6
    crystal_file        rep2000
    start_operator      I1x
    detect_operator     -I2z
    method              DNPframe
    sw                  1e9
    np                  1
    conjugate_fid       false
}

proc pulseq {} {
    global duration shp Nrep
    reset
    pulse_shaped  $duration $shp
    store         1
    reset
    prop          1 $Nrep
    acq
}

proc main {} {
    global duration shp Nrep
    # load appropriate pulse shape (5ns discretisation)
    set shp             [load_shape cRW.shp]
    set duration        [expr 0.005*[shape_len $shp]]
    set Nrep            13

    set fid [open cRW-OPT_bandwidth.dat w]
    # loop over offsets
    for {set g -60e6} {$g<=60e6} {set g [expr $g+1e5]} {
        set f [fsimpson [list [list gtensor_1_iso $g]]]
        puts "[format "%.0f" $g] [findex $f 1 -re]"
        puts $fid "[format "%.0f" $g] [findex $f 1 -re]"
        funload $f
    }
    close $fid
}
```

The cRW-OPT1 block is defined using a shaped pulse stored as a text file `cRW.shp`

```
23271500    0
31999700    180
31999700    0
31999800    0
27118800    180
31981000    180
28153700    180
24655300    180
```

```
30551100    0
31996600    180
31999900    180
7908330     180
31998400    0
31999900    0
31929500    0
31155000    0
20661300    0
29851800    180
24224600    180
31998500    0
32000000    0
31999700    0
18769000    0
31936100    180
23104800    0
31988900    0
513988      0
32000000    180
31988300    180
26226500    180
```

Examining the build-up of nuclear magnetization for NOVEL (main text Figure 3C, blue curve)

```
# spinsys defined in an external file
source DNP_sys_1.spinsys

par {
    proton_frequency    14.8e+6
    crystal_file        rep2000
    start_operator      I1x
    detect_operator     -I2z
    method              DNPframe
    sw                  1e9
    np                  5000
    conjugate_fid       false
}

proc pulseq {} {
    acq_block {
        pulse 0.8 14.8e+6 180
    }
}

proc main {} { fsave [fsimpson] novel_buildup.fid }
```

Examining the build-up of nuclear magnetization for BEAM (main text Figure 3C, red curve)

```
# spinsys defined in an external file
source DNP_sys_1.spinsys

par {
    proton_frequency    14.8e+6
    crystal_file        rep2000
    start_operator      I1x
    detect_operator     -I2z
    method              DNPframe
    sw                  1e9
    np                  5000
    conjugate_fid       false
}

proc pulseq {} {
    acq_block {
        pulse 28.0e-3 32e+6   0
        pulse 31.6e-3 32e+6 180
    }
}

proc main {} { fsave [fsimpson] beam_buildup.fid }
```

Examining the build-up of nuclear magnetization for PLATO (main text Figure 3C, green curve)

```
# spinsys defined in an external file
source DNP_sys_1.spinsys

par {
    proton_frequency    14.8e+6
    crystal_file        rep2000
    start_operator      I1x
    detect_operator     -I2z
    method              DNPframe
    sw                  1e9
    np                  5000
    conjugate_fid       false
}

proc pulseq {} {
    global shp duration
    acq_block {
        pulse_shaped $duration $shp
    }
}

proc main {} {
    global shp duration
    # load appropriate pulse shape (5ns discretisation)
    set shp [load_shape plato.shp]
    set duration [expr 0.005*[shape_len $shp]]

    fsave [fsimpson] plato_buildup.fid
}
```

Examining the build-up of nuclear magnetization for cRW-OPT1 (main text Figure 3C, purple curve)

```
# spinsys defined in an external file
source DNP_sys_1.spinsys

par {
    proton_frequency    14.8e+6
    crystal_file        rep2000
    start_operator      I1x
    detect_operator     -I2z
    method              DNPframe
    sw                  1e9
    np                  5000
    conjugate_fid       false
}

proc pulseq {} {
    global shp duration
    acq_block {
        pulse_shaped $duration $shp
    }
}

proc main {} {
    global shp duration
    # load appropriate pulse shape (5ns discretisation)
    set shp [load_shape cRW.shp]
    set duration [expr 0.005*[shape_len $shp]]

    fsave [fsimpson] cRW-OPT_buildup.fid
}
```

## 3 Gradient-free optimisation

Composite inversion pulse in an environment with high RF inhomogeneity, optimised using simplex method (main text Figure 4)

```
spinsys {
    channels    1H
    nuclei      1H
```

```
    }

    par {
        start_operator      I1z
        detect_operator     -I1z
        rfprof_file         solenoid.rf
        method              prop_split
        split_order         0

        # Parameters for optimisation
        conjugate_fid       false
        oc_optm_method      SIMPLEX
        oc_max_iter         150
    }

    proc pulseq {} {
        global par shp
        reset
        pulse_shaped $par(dur) $shp
        oc_acq_hermit
    }

    proc target_function {} {
        global par
        set f [fsimpson]
        set Res [findex $f 1 -re]
        funload $f
        return [format "%.20f" $Res]
    }

    proc main {} {
        global par shp

        # initial pulse sequence
        set shp [shape_create 5 -ampl 5000]
        set par(dur) 125.0

        # optimisation
        for {set i 0} {$i < 10} {incr i} {
          set tfopt [oc_optimize $shp -max 20000]
        }
        # save final result
        save_shape $shp shape_final.dat
        # free memory
        free_all_shapes
    }
```

The RF inhomogeneity is defined in the `solenoid.rf` file, where the weight factors (second column) reflect the reduced detection sensitivity when the $B_1$ field is lower (reciprocity theorem). The scaling factors (first column) were calculated along the coil axis starting from the coil centre towards the coil ending, equidistant increments, and using the Biot-Savart law. At the same time, the profile is assumed to be symmetric around the coil centre; extending for the second half of the profile increases weight factors.

```
16          1
1.00000000  0.03983506
0.99861765  0.07955939
0.99439095  0.07922088
0.98706668  0.07863448
0.97619214  0.07776426
0.96109426  0.07655679
0.94085187  0.07493893
0.91426222  0.07281523
0.87986022  0.07006939
0.83607182  0.06657652
0.78157119  0.06223156
0.71590492  0.05699882
0.64031322  0.05097734
0.55828061  0.04444456
0.47510649  0.03782214
0.39637999  0.03155464
```

The result of this optimisation is stored in the `simplex_shape_final.dat` file:

```
16078.7643468405    56.6830682863372
12451.5949730633    16.1104948466894
19038.6455968441    -73.2176646216678
8556.22442341501    38.3186389872424
20000               53.6518511869591
```

The inversion profiles of the shaped pulse and the rectangular pulse (main text Figure 4C) are calculated using the script

```
spinsys {
    channels    1H
    nuclei      1H
}

par {
    crystal_file    alpha0beta0
    gamma_angles    1
    sw              1e6
    start_operator  I1z
    detect_operator I1z
    np              1
    conjugate_fid   false
}

proc pulseq {} {
    global par shp
    reset
    pulse_shaped $par(dur) $shp
    oc_acq_hermit
}

proc main {} {
    global par shp

    # initial pulse sequence
    set shp0 [load_shape shape_final.dat]
    set par(dur) 125.0

    # create set of rf factors
    set rfac {}
    for {set x 0.1} {$x <= 1.21} {set x [expr {$x+0.025}]} {
      lappend rfac $x
    }
    set NN [llength $rfac]

    set fout [open $par(name)\_results.txt w]
    for {set k 0} {$k < $NN} {incr k} {
      set rfscl [lindex $rfac $k]
      set shp [shape_dup $shp0 0 $rfscl ]
      set f [fsimpson]
      set Res [findex $f 1 -re]
      puts $fout "[format "%12.8f" $rfscl] [format "%12.8f" $Res]"
      funload $f
      free_shape $shp
    }
    close $fout
    free_all_shapes

    # calculating performance of hard pulse
    set rfmax 20000.0
    set shp0 [shape_create 5 -ampl $rfmax]
    set par(dur) [expr 1.0e6/2.0/$rfmax]
    set fout [open $par(name)\_HP_results.txt w]
    for {set k 0} {$k < $NN} {incr k} {
      set rfscl [lindex $rfac $k]
      set shp [shape_dup $shp0 0 $rfscl ]
      set f [fsimpson]
      set Res [findex $f 1 -re]
      puts $fout "[format "%12.8f" $rfscl] [format "%12.8f" $Res]"
      funload $f
      free_shape $shp
    }
    close $fout
```

```
    free_all_shapes
}
```

# 4 Optimisation of SORDOR pulse

SORDOR pulses (main text Figure 5) are calculated using a morphic optimal control approach using the input file

```
spinsys {
    channels    13C
    nuclei      13C
    shift       1 1 0 0 0 0 0
}

par {
    averaging_file      shift_1_iso_40kHz.ave
    oc_max_iter         500
    method              prop_split
    split_order         1
    oc_grad_level       2
    oc_cg_min_step      1e-4
    conjugate_fid       false
}

proc pulseq {} {
    global shp Omega duration Q

    set ak [get_dsp $Omega $duration $Q]
    set cosak [expr {cos($ak)}]
    set sinak [expr {sin($ak)}]
    reset

    avgham_static 0.25e6 $cosak*(I1x)+$sinak*(I1y)
    store 10
    reset
    pulse_shaped $duration $shp
    oc_acq_prop 10
}

proc target_function {} {
    global par

    # we acquire a single number
    set par(np) 1
    set f [fsimpson]
    set Res [findex $f 1 -re]
    funload $f
    return [format "%.20f" [expr {$Res/4.0}]]
}

proc gradient {} {
    global par NOC

    set par(np) $NOC
    set g [fsimpson]
    return $g
}

proc get_dsp {Omega duration Q} {
    set pi 3.14159265358979323846
    set b [expr {$duration/25.0}]
    set H [matrix get hamiltonian]
    set h11 [expr round([lindex $H 0 0]/($pi))]
    set ak [expr {$pi*$b*$Q*(1-(($h11/$Omega)**2))}]
    return $ak
}

proc main {} {
    global par shp NOC Omega Q duration

    # load the BURBOP shape
    set shp [load_shape burbop090_0300us.dat]
    set NOC [shape_len $shp]
    set duration [expr {$NOC/2.0}]
    set Omega 40e3
```

```
    set tfbest 0.0
    set shpbest $shp
    set Q 0.0

    for {set Q 0.0} {$Q<=1.00} {set Q [expr {$Q+0.01}]} {
        set Q [format "%.2f" $Q]
        puts "Optimising for Q = $Q"
        set tfopt [oc_optimize_phase $shp]
        if {$tfopt>$tfbest} {
            set tfbest $tfopt
            puts "Optimum at Q = $Q"
            save_shape $shp sordor090_optim_0300us.dat
        }
        set fid [open sordor_fidelities_300.dat a]
        puts $fid "  $Q [format "%12.4e" [expr {1-$tfopt}]] "
        close $fid
    }
    free_all_shapes
}
```

It uses a range of offsets defined as averaging file `shift_1_iso_40kHz.ave` :

```
shift_1_iso    weight
      20000    0.0243902439
      19000    0.0243902439
      18000    0.0243902439
      17000    0.0243902439
      16000    0.0243902439
      15000    0.0243902439
      14000    0.0243902439
      13000    0.0243902439
      12000    0.0243902439
      11000    0.0243902439
      10000    0.0243902439
      9000     0.0243902439
      8000     0.0243902439
      7000     0.0243902439
      6000     0.0243902439
      5000     0.0243902439
      4000     0.0243902439
      3000     0.0243902439
      2000     0.0243902439
      1000     0.0243902439
      0        0.0243902439
      -1000    0.0243902439
      -2000    0.0243902439
      -3000    0.0243902439
      -4000    0.0243902439
      -5000    0.0243902439
      -6000    0.0243902439
      -7000    0.0243902439
      -8000    0.0243902439
      -9000    0.0243902439
      -10000   0.0243902439
      -11000   0.0243902439
      -12000   0.0243902439
      -13000   0.0243902439
      -14000   0.0243902439
      -15000   0.0243902439
      -16000   0.0243902439
      -17000   0.0243902439
      -18000   0.0243902439
      -19000   0.0243902439
      -20000   0.0243902439
```

The initial shape to start the optimisation is a BURBOP pulse (corresponding to $Q = 0$ condition) defined in the `burbop090_0300us.dat` file:

```
1.000000E04  9.740638E01
1.000000E04  1.083172E02
1.000000E04  1.162941E02
```

| | |
|---|---|
| 1.000000E04 | 1.219304E02 |
| 1.000000E04 | 1.258817E02 |
| 1.000000E04 | 1.286445E02 |
| 1.000000E04 | 1.305473E02 |
| 1.000000E04 | 1.318025E02 |
| 1.000000E04 | 1.325508E02 |
| 1.000000E04 | 1.328879E02 |
| 1.000000E04 | 1.328803E02 |
| 1.000000E04 | 1.325730E02 |
| 1.000000E04 | 1.319954E02 |
| 1.000000E04 | 1.311655E02 |
| 1.000000E04 | 1.300919E02 |
| 1.000000E04 | 1.287761E02 |
| 1.000000E04 | 1.272142E02 |
| 1.000000E04 | 1.253991E02 |
| 1.000000E04 | 1.233193E02 |
| 1.000000E04 | 1.209607E02 |
| 1.000000E04 | 1.183132E02 |
| 1.000000E04 | 1.153653E02 |
| 1.000000E04 | 1.121137E02 |
| 1.000000E04 | 1.085632E02 |
| 1.000000E04 | 1.047057E02 |
| 1.000000E04 | 1.006067E02 |
| 1.000000E04 | 9.632960E01 |
| 1.000000E04 | 9.195716E01 |
| 1.000000E04 | 8.760477E01 |
| 1.000000E04 | 8.337922E01 |
| 1.000000E04 | 7.938837E01 |
| 1.000000E04 | 7.574348E01 |
| 1.000000E04 | 7.247845E01 |
| 1.000000E04 | 6.979491E01 |
| 1.000000E04 | 6.774123E01 |
| 1.000000E04 | 6.637603E01 |
| 1.000000E04 | 6.575203E01 |
| 1.000000E04 | 6.588546E01 |
| 1.000000E04 | 6.685413E01 |
| 1.000000E04 | 6.870881E01 |
| 1.000000E04 | 7.146463E01 |
| 1.000000E04 | 7.509546E01 |
| 1.000000E04 | 7.965415E01 |
| 1.000000E04 | 8.498437E01 |
| 1.000000E04 | 9.086799E01 |
| 1.000000E04 | 9.698064E01 |
| 1.000000E04 | 1.030444E02 |
| 1.000000E04 | 1.088370E02 |
| 1.000000E04 | 1.142106E02 |
| 1.000000E04 | 1.190944E02 |
| 1.000000E04 | 1.234660E02 |
| 1.000000E04 | 1.273270E02 |
| 1.000000E04 | 1.307062E02 |
| 1.000000E04 | 1.336843E02 |
| 1.000000E04 | 1.363479E02 |
| 1.000000E04 | 1.387478E02 |
| 1.000000E04 | 1.409014E02 |
| 1.000000E04 | 1.428409E02 |
| 1.000000E04 | 1.446177E02 |
| 1.000000E04 | 1.462649E02 |
| 1.000000E04 | 1.477793E02 |
| 1.000000E04 | 1.491777E02 |
| 1.000000E04 | 1.504890E02 |
| 1.000000E04 | 1.517337E02 |
| 1.000000E04 | 1.529192E02 |
| 1.000000E04 | 1.540514E02 |
| 1.000000E04 | 1.551344E02 |
| 1.000000E04 | 1.561767E02 |
| 1.000000E04 | 1.571891E02 |
| 1.000000E04 | 1.581811E02 |
| 1.000000E04 | 1.591594E02 |
| 1.000000E04 | 1.601289E02 |
| 1.000000E04 | 1.610934E02 |
| 1.000000E04 | 1.620563E02 |
| 1.000000E04 | 1.630217E02 |
| 1.000000E04 | 1.639943E02 |
| 1.000000E04 | 1.649795E02 |
| 1.000000E04 | 1.659826E02 |
| 1.000000E04 | 1.670095E02 |

| | |
|---|---|
| 1.000000E04 | 1.680659E02 |
| 1.000000E04 | 1.691586E02 |
| 1.000000E04 | 1.702946E02 |
| 1.000000E04 | 1.714818E02 |
| 1.000000E04 | 1.727289E02 |
| 1.000000E04 | 1.740462E02 |
| 1.000000E04 | 1.754452E02 |
| 1.000000E04 | 1.769394E02 |
| 1.000000E04 | 1.785450E02 |
| 1.000000E04 | 1.802806E02 |
| 1.000000E04 | 1.821687E02 |
| 1.000000E04 | 1.842360E02 |
| 1.000000E04 | 1.865146E02 |
| 1.000000E04 | 1.890433E02 |
| 1.000000E04 | 1.918685E02 |
| 1.000000E04 | 1.950458E02 |
| 1.000000E04 | 1.986402E02 |
| 1.000000E04 | 2.027251E02 |
| 1.000000E04 | 2.073780E02 |
| 1.000000E04 | 2.126780E02 |
| 1.000000E04 | 2.186903E02 |
| 1.000000E04 | 2.254373E02 |
| 1.000000E04 | 2.328703E02 |
| 1.000000E04 | 2.408580E02 |
| 1.000000E04 | 2.491604E02 |
| 1.000000E04 | 2.574603E02 |
| 1.000000E04 | 2.654627E02 |
| 1.000000E04 | 2.729322E02 |
| 1.000000E04 | 2.797286E02 |
| 1.000000E04 | 2.858021E02 |
| 1.000000E04 | 2.911743E02 |
| 1.000000E04 | 2.959125E02 |
| 1.000000E04 | 3.000985E02 |
| 1.000000E04 | 3.038119E02 |
| 1.000000E04 | 3.071247E02 |
| 1.000000E04 | 3.101006E02 |
| 1.000000E04 | 3.127952E02 |
| 1.000000E04 | 3.152575E02 |
| 1.000000E04 | 3.175289E02 |
| 1.000000E04 | 3.196435E02 |
| 1.000000E04 | 3.216293E02 |
| 1.000000E04 | 3.235095E02 |
| 1.000000E04 | 3.253046E02 |
| 1.000000E04 | 3.270325E02 |
| 1.000000E04 | 3.287096E02 |
| 1.000000E04 | 3.303509E02 |
| 1.000000E04 | 3.319701E02 |
| 1.000000E04 | 3.335800E02 |
| 1.000000E04 | 3.351928E02 |
| 1.000000E04 | 3.368204E02 |
| 1.000000E04 | 3.384746E02 |
| 1.000000E04 | 3.401670E02 |
| 1.000000E04 | 3.419097E02 |
| 1.000000E04 | 3.437151E02 |
| 1.000000E04 | 3.455962E02 |
| 1.000000E04 | 3.475662E02 |
| 1.000000E04 | 3.496393E02 |
| 1.000000E04 | 3.518299E02 |
| 1.000000E04 | 3.541528E02 |
| 1.000000E04 | 3.566227E02 |
| 1.000000E04 | 3.592537E02 |
| 1.000000E04 | 2.058679E00 |
| 1.000000E04 | 5.048316E00 |
| 1.000000E04 | 8.229927E00 |
| 1.000000E04 | 1.160602E01 |
| 1.000000E04 | 1.517264E01 |
| 1.000000E04 | 1.891773E01 |
| 1.000000E04 | 2.281979E01 |
| 1.000000E04 | 2.684732E01 |
| 1.000000E04 | 3.095934E01 |
| 1.000000E04 | 3.510716E01 |
| 1.000000E04 | 3.923733E01 |
| 1.000000E04 | 4.329539E01 |
| 1.000000E04 | 4.722974E01 |
| 1.000000E04 | 5.099519E01 |
| 1.000000E04 | 5.455534E01 |

| | |
|---|---|
| 1.000000E04 | 5.788358E01 |
| 1.000000E04 | 6.096280E01 |
| 1.000000E04 | 6.378420E01 |
| 1.000000E04 | 6.634578E01 |
| 1.000000E04 | 6.865102E01 |
| 1.000000E04 | 7.070776E01 |
| 1.000000E04 | 7.252719E01 |
| 1.000000E04 | 7.412249E01 |
| 1.000000E04 | 7.550737E01 |
| 1.000000E04 | 7.669501E01 |
| 1.000000E04 | 7.769769E01 |
| 1.000000E04 | 7.852697E01 |
| 1.000000E04 | 7.919388E01 |
| 1.000000E04 | 7.970914E01 |
| 1.000000E04 | 8.008300E01 |
| 1.000000E04 | 8.032513E01 |
| 1.000000E04 | 8.044443E01 |
| 1.000000E04 | 8.044906E01 |
| 1.000000E04 | 8.034652E01 |
| 1.000000E04 | 8.014378E01 |
| 1.000000E04 | 7.984747E01 |
| 1.000000E04 | 7.946398E01 |
| 1.000000E04 | 7.899960E01 |
| 1.000000E04 | 7.846054E01 |
| 1.000000E04 | 7.785300E01 |
| 1.000000E04 | 7.718320E01 |
| 1.000000E04 | 7.645740E01 |
| 1.000000E04 | 7.568192E01 |
| 1.000000E04 | 7.486316E01 |
| 1.000000E04 | 7.400759E01 |
| 1.000000E04 | 7.312178E01 |
| 1.000000E04 | 7.221241E01 |
| 1.000000E04 | 7.128619E01 |
| 1.000000E04 | 7.034994E01 |
| 1.000000E04 | 6.941051E01 |
| 1.000000E04 | 6.847479E01 |
| 1.000000E04 | 6.754967E01 |
| 1.000000E04 | 6.664202E01 |
| 1.000000E04 | 6.575870E01 |
| 1.000000E04 | 6.490650E01 |
| 1.000000E04 | 6.409218E01 |
| 1.000000E04 | 6.332242E01 |
| 1.000000E04 | 6.260385E01 |
| 1.000000E04 | 6.194307E01 |
| 1.000000E04 | 6.134663E01 |
| 1.000000E04 | 6.082110E01 |
| 1.000000E04 | 6.037305E01 |
| 1.000000E04 | 6.000913E01 |
| 1.000000E04 | 5.973607E01 |
| 1.000000E04 | 5.956072E01 |
| 1.000000E04 | 5.949007E01 |
| 1.000000E04 | 5.953130E01 |
| 1.000000E04 | 5.969171E01 |
| 1.000000E04 | 5.997876E01 |
| 1.000000E04 | 6.039995E01 |
| 1.000000E04 | 6.096279E01 |
| 1.000000E04 | 6.167458E01 |
| 1.000000E04 | 6.254226E01 |
| 1.000000E04 | 6.357210E01 |
| 1.000000E04 | 6.476937E01 |
| 1.000000E04 | 6.613778E01 |
| 1.000000E04 | 6.767899E01 |
| 1.000000E04 | 6.939192E01 |
| 1.000000E04 | 7.127207E01 |
| 1.000000E04 | 7.331086E01 |
| 1.000000E04 | 7.549517E01 |
| 1.000000E04 | 7.780703E01 |
| 1.000000E04 | 8.022374E01 |
| 1.000000E04 | 8.271829E01 |
| 1.000000E04 | 8.526031E01 |
| 1.000000E04 | 8.781726E01 |
| 1.000000E04 | 9.035598E01 |
| 1.000000E04 | 9.284423E01 |
| 1.000000E04 | 9.525211E01 |
| 1.000000E04 | 9.755327E01 |
| 1.000000E04 | 9.972572E01 |

| | |
|---|---|
| 1.000000E04 | 1.017523E02 |
| 1.000000E04 | 1.036208E02 |
| 1.000000E04 | 1.053237E02 |
| 1.000000E04 | 1.068570E02 |
| 1.000000E04 | 1.082197E02 |
| 1.000000E04 | 1.094123E02 |
| 1.000000E04 | 1.104369E02 |
| 1.000000E04 | 1.112972E02 |
| 1.000000E04 | 1.119989E02 |
| 1.000000E04 | 1.125488E02 |
| 1.000000E04 | 1.129541E02 |
| 1.000000E04 | 1.132211E02 |
| 1.000000E04 | 1.133552E02 |
| 1.000000E04 | 1.133605E02 |
| 1.000000E04 | 1.132413E02 |
| 1.000000E04 | 1.130015E02 |
| 1.000000E04 | 1.126455E02 |
| 1.000000E04 | 1.121771E02 |
| 1.000000E04 | 1.116001E02 |
| 1.000000E04 | 1.109175E02 |
| 1.000000E04 | 1.101318E02 |
| 1.000000E04 | 1.092452E02 |
| 1.000000E04 | 1.082597E02 |
| 1.000000E04 | 1.071771E02 |
| 1.000000E04 | 1.059989E02 |
| 1.000000E04 | 1.047269E02 |
| 1.000000E04 | 1.033629E02 |
| 1.000000E04 | 1.019085E02 |
| 1.000000E04 | 1.003658E02 |
| 1.000000E04 | 9.873682E01 |
| 1.000000E04 | 9.702386E01 |
| 1.000000E04 | 9.522952E01 |
| 1.000000E04 | 9.335674E01 |
| 1.000000E04 | 9.140880E01 |
| 1.000000E04 | 8.938936E01 |
| 1.000000E04 | 8.730250E01 |
| 1.000000E04 | 8.515269E01 |
| 1.000000E04 | 8.294481E01 |
| 1.000000E04 | 8.068407E01 |
| 1.000000E04 | 7.837598E01 |
| 1.000000E04 | 7.602631E01 |
| 1.000000E04 | 7.364097E01 |
| 1.000000E04 | 7.122594E01 |
| 1.000000E04 | 6.878717E01 |
| 1.000000E04 | 6.633045E01 |
| 1.000000E04 | 6.386136E01 |
| 1.000000E04 | 6.138514E01 |
| 1.000000E04 | 5.890659E01 |
| 1.000000E04 | 5.643004E01 |
| 1.000000E04 | 5.395922E01 |
| 1.000000E04 | 5.149729E01 |
| 1.000000E04 | 4.904674E01 |
| 1.000000E04 | 4.660940E01 |
| 1.000000E04 | 4.418644E01 |
| 1.000000E04 | 4.177836E01 |
| 1.000000E04 | 3.938502E01 |
| 1.000000E04 | 3.700566E01 |
| 1.000000E04 | 3.463891E01 |
| 1.000000E04 | 3.228282E01 |
| 1.000000E04 | 2.993493E01 |
| 1.000000E04 | 2.759224E01 |
| 1.000000E04 | 2.525129E01 |
| 1.000000E04 | 2.290816E01 |
| 1.000000E04 | 2.055850E01 |
| 1.000000E04 | 1.819756E01 |
| 1.000000E04 | 1.582022E01 |
| 1.000000E04 | 1.342103E01 |
| 1.000000E04 | 1.099422E01 |
| 1.000000E04 | 8.533742E00 |
| 1.000000E04 | 6.033362E00 |
| 1.000000E04 | 3.486674E00 |
| 1.000000E04 | 8.872050E-01 |
| 1.000000E04 | 3.582285E02 |
| 1.000000E04 | 3.555043E02 |
| 1.000000E04 | 3.527086E02 |
| 1.000000E04 | 3.498359E02 |

| | |
|---|---|
| 1.000000E04 | 3.468815E02 |
| 1.000000E04 | 3.438414E02 |
| 1.000000E04 | 3.407133E02 |
| 1.000000E04 | 3.374960E02 |
| 1.000000E04 | 3.341905E02 |
| 1.000000E04 | 3.308001E02 |
| 1.000000E04 | 3.273307E02 |
| 1.000000E04 | 3.237912E02 |
| 1.000000E04 | 3.201933E02 |
| 1.000000E04 | 3.165514E02 |
| 1.000000E04 | 3.128827E02 |
| 1.000000E04 | 3.092060E02 |
| 1.000000E04 | 3.055415E02 |
| 1.000000E04 | 3.019102E02 |
| 1.000000E04 | 2.983329E02 |
| 1.000000E04 | 2.948292E02 |
| 1.000000E04 | 2.914175E02 |
| 1.000000E04 | 2.881139E02 |
| 1.000000E04 | 2.849318E02 |
| 1.000000E04 | 2.818820E02 |
| 1.000000E04 | 2.789725E02 |
| 1.000000E04 | 2.762086E02 |
| 1.000000E04 | 2.735935E02 |
| 1.000000E04 | 2.711282E02 |
| 1.000000E04 | 2.688123E02 |
| 1.000000E04 | 2.666442E02 |
| 1.000000E04 | 2.646211E02 |
| 1.000000E04 | 2.627399E02 |
| 1.000000E04 | 2.609967E02 |
| 1.000000E04 | 2.593877E02 |
| 1.000000E04 | 2.579089E02 |
| 1.000000E04 | 2.565565E02 |
| 1.000000E04 | 2.553270E02 |
| 1.000000E04 | 2.542172E02 |
| 1.000000E04 | 2.532243E02 |
| 1.000000E04 | 2.523460E02 |
| 1.000000E04 | 2.515808E02 |
| 1.000000E04 | 2.509275E02 |
| 1.000000E04 | 2.503858E02 |
| 1.000000E04 | 2.499561E02 |
| 1.000000E04 | 2.496396E02 |
| 1.000000E04 | 2.494383E02 |
| 1.000000E04 | 2.493550E02 |
| 1.000000E04 | 2.493934E02 |
| 1.000000E04 | 2.495587E02 |
| 1.000000E04 | 2.498577E02 |
| 1.000000E04 | 2.503000E02 |
| 1.000000E04 | 2.508974E02 |
| 1.000000E04 | 2.516629E02 |
| 1.000000E04 | 2.526101E02 |
| 1.000000E04 | 2.537549E02 |
| 1.000000E04 | 2.551183E02 |
| 1.000000E04 | 2.567279E02 |
| 1.000000E04 | 2.586145E02 |
| 1.000000E04 | 2.608114E02 |
| 1.000000E04 | 2.633574E02 |
| 1.000000E04 | 2.662962E02 |
| 1.000000E04 | 2.696706E02 |
| 1.000000E04 | 2.735214E02 |
| 1.000000E04 | 2.778877E02 |
| 1.000000E04 | 2.827958E02 |
| 1.000000E04 | 2.882394E02 |
| 1.000000E04 | 2.941691E02 |
| 1.000000E04 | 3.004894E02 |
| 1.000000E04 | 3.070611E02 |
| 1.000000E04 | 3.137124E02 |
| 1.000000E04 | 3.202630E02 |
| 1.000000E04 | 3.265522E02 |
| 1.000000E04 | 3.324605E02 |
| 1.000000E04 | 3.379177E02 |
| 1.000000E04 | 3.428967E02 |
| 1.000000E04 | 3.474114E02 |
| 1.000000E04 | 3.514932E02 |
| 1.000000E04 | 3.551827E02 |
| 1.000000E04 | 3.585255E02 |
| 1.000000E04 | 1.568730E00 |

| | |
|---|---|
| 1.000000E04 | 4.357343E00 |
| 1.000000E04 | 6.932601E00 |
| 1.000000E04 | 9.330927E00 |
| 1.000000E04 | 1.158426E01 |
| 1.000000E04 | 1.372089E01 |
| 1.000000E04 | 1.576622E01 |
| 1.000000E04 | 1.774340E01 |
| 1.000000E04 | 1.967373E01 |
| 1.000000E04 | 2.157711E01 |
| 1.000000E04 | 2.347245E01 |
| 1.000000E04 | 2.537813E01 |
| 1.000000E04 | 2.731242E01 |
| 1.000000E04 | 2.929392E01 |
| 1.000000E04 | 3.134202E01 |
| 1.000000E04 | 3.347726E01 |
| 1.000000E04 | 3.572168E01 |
| 1.000000E04 | 3.809916E01 |
| 1.000000E04 | 4.063562E01 |
| 1.000000E04 | 4.335941E01 |
| 1.000000E04 | 4.630169E01 |
| 1.000000E04 | 4.949664E01 |
| 1.000000E04 | 5.298071E01 |
| 1.000000E04 | 5.679061E01 |
| 1.000000E04 | 6.096000E01 |
| 1.000000E04 | 6.551561E01 |
| 1.000000E04 | 7.047248E01 |
| 1.000000E04 | 7.582757E01 |
| 1.000000E04 | 8.155207E01 |
| 1.000000E04 | 8.758510E01 |
| 1.000000E04 | 9.383258E01 |
| 1.000000E04 | 1.001737E02 |
| 1.000000E04 | 1.064747E02 |
| 1.000000E04 | 1.126062E02 |
| 1.000000E04 | 1.184593E02 |
| 1.000000E04 | 1.239553E02 |
| 1.000000E04 | 1.290479E02 |
| 1.000000E04 | 1.337202E02 |
| 1.000000E04 | 1.379788E02 |
| 1.000000E04 | 1.418460E02 |
| 1.000000E04 | 1.453527E02 |
| 1.000000E04 | 1.485324E02 |
| 1.000000E04 | 1.514185E02 |
| 1.000000E04 | 1.540436E02 |
| 1.000000E04 | 1.564391E02 |
| 1.000000E04 | 1.586333E02 |
| 1.000000E04 | 1.606503E02 |
| 1.000000E04 | 1.625114E02 |
| 1.000000E04 | 1.642350E02 |
| 1.000000E04 | 1.658378E02 |
| 1.000000E04 | 1.673344E02 |
| 1.000000E04 | 1.687381E02 |
| 1.000000E04 | 1.700602E02 |
| 1.000000E04 | 1.713106E02 |
| 1.000000E04 | 1.724979E02 |
| 1.000000E04 | 1.736299E02 |
| 1.000000E04 | 1.747135E02 |
| 1.000000E04 | 1.757549E02 |
| 1.000000E04 | 1.767599E02 |
| 1.000000E04 | 1.777336E02 |
| 1.000000E04 | 1.786808E02 |
| 1.000000E04 | 1.796061E02 |
| 1.000000E04 | 1.805135E02 |
| 1.000000E04 | 1.814070E02 |
| 1.000000E04 | 1.822903E02 |
| 1.000000E04 | 1.831669E02 |
| 1.000000E04 | 1.840403E02 |
| 1.000000E04 | 1.849138E02 |
| 1.000000E04 | 1.857906E02 |
| 1.000000E04 | 1.866739E02 |
| 1.000000E04 | 1.875664E02 |
| 1.000000E04 | 1.884710E02 |
| 1.000000E04 | 1.893905E02 |
| 1.000000E04 | 1.903272E02 |
| 1.000000E04 | 1.912838E02 |
| 1.000000E04 | 1.922625E02 |
| 1.000000E04 | 1.932654E02 |

| | |
|---|---|
| 1.000000E04 | 1.942943E02 |
| 1.000000E04 | 1.953504E02 |
| 1.000000E04 | 1.964345E02 |
| 1.000000E04 | 1.975470E02 |
| 1.000000E04 | 1.986878E02 |
| 1.000000E04 | 1.998560E02 |
| 1.000000E04 | 2.010500E02 |
| 1.000000E04 | 2.022673E02 |
| 1.000000E04 | 2.035040E02 |
| 1.000000E04 | 2.047550E02 |
| 1.000000E04 | 2.060143E02 |
| 1.000000E04 | 2.072749E02 |
| 1.000000E04 | 2.085289E02 |
| 1.000000E04 | 2.097680E02 |
| 1.000000E04 | 2.109830E02 |
| 1.000000E04 | 2.121647E02 |
| 1.000000E04 | 2.133037E02 |
| 1.000000E04 | 2.143906E02 |
| 1.000000E04 | 2.154168E02 |
| 1.000000E04 | 2.163746E02 |
| 1.000000E04 | 2.172573E02 |
| 1.000000E04 | 2.180597E02 |
| 1.000000E04 | 2.187780E02 |
| 1.000000E04 | 2.194100E02 |
| 1.000000E04 | 2.199550E02 |
| 1.000000E04 | 2.204138E02 |
| 1.000000E04 | 2.207885E02 |
| 1.000000E04 | 2.210822E02 |
| 1.000000E04 | 2.212994E02 |
| 1.000000E04 | 2.214449E02 |
| 1.000000E04 | 2.215244E02 |
| 1.000000E04 | 2.215438E02 |
| 1.000000E04 | 2.215092E02 |
| 1.000000E04 | 2.214270E02 |
| 1.000000E04 | 2.213034E02 |
| 1.000000E04 | 2.211443E02 |
| 1.000000E04 | 2.209555E02 |
| 1.000000E04 | 2.207424E02 |
| 1.000000E04 | 2.205101E02 |
| 1.000000E04 | 2.202632E02 |
| 1.000000E04 | 2.200059E02 |
| 1.000000E04 | 2.197420E02 |
| 1.000000E04 | 2.194748E02 |
| 1.000000E04 | 2.192073E02 |
| 1.000000E04 | 2.189421E02 |
| 1.000000E04 | 2.186815E02 |
| 1.000000E04 | 2.184273E02 |
| 1.000000E04 | 2.181815E02 |
| 1.000000E04 | 2.179453E02 |
| 1.000000E04 | 2.177201E02 |
| 1.000000E04 | 2.175069E02 |
| 1.000000E04 | 2.173067E02 |
| 1.000000E04 | 2.171202E02 |
| 1.000000E04 | 2.169482E02 |
| 1.000000E04 | 2.167912E02 |
| 1.000000E04 | 2.166497E02 |
| 1.000000E04 | 2.165242E02 |
| 1.000000E04 | 2.164151E02 |
| 1.000000E04 | 2.163227E02 |
| 1.000000E04 | 2.162475E02 |
| 1.000000E04 | 2.161898E02 |
| 1.000000E04 | 2.161502E02 |
| 1.000000E04 | 2.161293E02 |
| 1.000000E04 | 2.161279E02 |
| 1.000000E04 | 2.161468E02 |
| 1.000000E04 | 2.161867E02 |
| 1.000000E04 | 2.162480E02 |
| 1.000000E04 | 2.163308E02 |
| 1.000000E04 | 2.164353E02 |
| 1.000000E04 | 2.165618E02 |
| 1.000000E04 | 2.167119E02 |
| 1.000000E04 | 2.168890E02 |
| 1.000000E04 | 2.170971E02 |
| 1.000000E04 | 2.173398E02 |
| 1.000000E04 | 2.176180E02 |
| 1.000000E04 | 2.179298E02 |

```
1.000000E04  2.182741E02
1.000000E04  2.186543E02
1.000000E04  2.190807E02
1.000000E04  2.195654E02
1.000000E04  2.201157E02
1.000000E04  2.207319E02
1.000000E04  2.214155E02
1.000000E04  2.221763E02
1.000000E04  2.230320E02
1.000000E04  2.240030E02
1.000000E04  2.251113E02
1.000000E04  2.263848E02
1.000000E04  2.278654E02
1.000000E04  2.295712E02
1.000000E04  2.315475E02
1.000000E04  2.338909E02
1.000000E04  2.367187E02
1.000000E04  2.401825E02
1.000000E04  2.443868E02
1.000000E04  2.494838E02
1.000000E04  2.557114E02
1.000000E04  2.630338E02
1.000000E04  2.711385E02
1.000000E04  2.794327E02
1.000000E04  2.865552E02
1.000000E04  2.917355E02
1.000000E04  2.948907E02
1.000000E04  2.959960E02
1.000000E04  2.952046E02
1.000000E04  2.928185E02
1.000000E04  2.891452E02
1.000000E04  2.845015E02
1.000000E04  2.792582E02
1.000000E04  2.737757E02
1.000000E04  2.683114E02
1.000000E04  2.630340E02
1.000000E04  2.580765E02
1.000000E04  2.535315E02
1.000000E04  2.494351E02
1.000000E04  2.457763E02
1.000000E04  2.425320E02
1.000000E04  2.396817E02
1.000000E04  2.371832E02
1.000000E04  2.349846E02
1.000000E04  2.330597E02
1.000000E04  2.313844E02
1.000000E04  2.299350E02
1.000000E04  2.286930E02
1.000000E04  2.276417E02
1.000000E04  2.267688E02
1.000000E04  2.260703E02
1.000000E04  2.255485E02
1.000000E04  2.252115E02
1.000000E04  2.250741E02
1.000000E04  2.251594E02
1.000000E04  2.255008E02
1.000000E04  2.261477E02
1.000000E04  2.271702E02
1.000000E04  2.286686E02
1.000000E04  2.307883E02
1.000000E04  2.337444E02
1.000000E04  2.378659E02
1.000000E04  2.436404E02
1.000000E04  2.517026E02
1.000000E04  2.626324E02
```

# 5 High accuracy splittings

A number of propagator splittings are presented in the main text. The comparative timings of these splitting methods for the PLATO pulse sequence produce results of varying accuracy. A course examination of the bandwidth of PLATO:

```
# spinsys defined in an external file
source DNP_sys_1.spinsys
```

```
par {
    proton_frequency    14.8e+6
    crystal_file        rep2000
    start_operator      I1x
    detect_operator     -I2z
    method              DNPframe prop_split
    split_order         2
    sw                  1e9
    np                  1
    conjugate_fid       false
}

proc pulseq {} {
    global duration shp Nrep
    reset
    maxdt           0.00125
    pulse_shaped    $duration $shp
    store           1
    reset
    prop            1 $Nrep
    acq
}

proc main {} {
    global duration shp Nrep par
    # load appropriate pulse shape (5ns discretisation)
    set shp             [load_shape plato.shp]
    set duration        [expr 0.005*[shape_len $shp]]
    set Nrep            15

    set ttot 0.0
    set fid [open plato_BW_split2_4.dat w]
    # loop over offsets
    for {set g -60e6} {$g<=60e6} {set g [expr $g+1e6]} {
        set f [fsimpson [list [list gtensor_1_iso $g]]]
        puts $fid "[findex $f 1 -re]"
        funload $f
        set ttot_new $par(tcalc)
        set ttot "[expr $ttot_new+$ttot]"
    }
    puts "split 2 -- [expr $ttot/1e6]"
    close $fid
}
```

The results for the `diag` method, considered exact, are used to compare accuracy and are:

```
-60000000 0.0417472740600197
-59000000 0.0166423114643862
-58000000 0.0325412400417753
-57000000 0.0355058297412118
-56000000 -0.0163836355166877
-55000000 -0.00697713696211222
-54000000 -0.00791713795866192
-53000000 -0.0042035557173171
-52000000 -0.0160692053852944
-51000000 -0.0176049424579165
-50000000 -0.0151430059626725
-49000000 -0.00245142795557383
-48000000 -0.0137647721030929
-47000000 -0.00897761118593071
-46000000 -0.0947180167537862
-45000000 -0.202600389695923
-44000000 -0.0138951599419611
-43000000 0.00181843804508597
-42000000 -0.000905009089993106
-41000000 0.0010559115452434
-40000000 0.000885209187733222
-39000000 0.0501105245860158
-38000000 0.036037755832034
-37000000 0.0333287677056355
-36000000 0.340232426919156
-35000000 0.618732758295098
-34000000 0.670006255832269
-33000000 0.619839473027953
-32000000 0.581735118907059
```

-31000000 0.585939523883373
-30000000 0.621893839658754
-29000000 0.666536340765288
-28000000 0.70041871205179
-27000000 0.717266193896518
-26000000 0.721664529710484
-25000000 0.719375341300608
-24000000 0.711540985185652
-23000000 0.696523399317914
-22000000 0.674631115415118
-21000000 0.649927411412759
-20000000 0.627890112631833
-19000000 0.611960532206852
-18000000 0.602017976432553
-17000000 0.595429203544927
-16000000 0.589568839565744
-15000000 0.584023933485011
-14000000 0.580980375332753
-13000000 0.583661867961361
-12000000 0.594100301043622
-11000000 0.611695735553524
-10000000 0.633262062926762
-9000000 0.654435760663369
-8000000 0.671645462482144
-7000000 0.683467079735016
-6000000 0.690614456767585
-5000000 0.694849189724957
-4000000 0.697758990442779
-3000000 0.700143895349428
-2000000 0.702096678926348
-1000000 0.703402631541109
0 0.703861447875253
1000000 0.703402631541111
2000000 0.702096678926348
3000000 0.700143895349425
4000000 0.697758990442779
5000000 0.694849189724954
6000000 0.690614456767583
7000000 0.683467079735013
8000000 0.671645462482141
9000000 0.654435760663368
10000000 0.63326206292676
11000000 0.611695735553521
12000000 0.59410030104362
13000000 0.583661867961358
14000000 0.580980375332751
15000000 0.58402393348501
16000000 0.589568839565743
17000000 0.595429203544925
18000000 0.602017976432552
19000000 0.611960532206852
20000000 0.627890112631834
21000000 0.64992741141276
22000000 0.674631115415119
23000000 0.696523399317913
24000000 0.711540985185649
25000000 0.719375341300607
26000000 0.721664529710484
27000000 0.717266193896517
28000000 0.700418712051793
29000000 0.666536340765291
30000000 0.621893839658757
31000000 0.585939523883377
32000000 0.581735118907063
33000000 0.619839473027958
34000000 0.670006255832271
35000000 0.618732758295096
36000000 0.340232426919152
37000000 0.0333287677056355
38000000 0.0360377558320373
39000000 0.050110524586017
40000000 0.000885209187735223
41000000 0.00105591154524385
42000000 -0.000905009089993357
43000000 0.00181843804508622
44000000 -0.01389515994196

```
45000000 -0.202600389695923
46000000 -0.0947180167537905
47000000 -0.00897761118593062
48000000 -0.0137647721030947
49000000 -0.00245142795557465
50000000 -0.015143005962673 7
51000000 -0.0176049424579175
52000000 -0.0160692053852948
53000000 -0.0042035557173172
54000000 -0.00791713795866242
55000000 -0.0069771369621121
56000000 -0.0163836355166882
57000000 0.0355058297412121
58000000 0.0325412400417743
59000000 0.0166423114643853
60000000 0.0417472740600186
```

For `split_order 2`:

```
-60000000 -0.000706256001157649
-59000000 0.00185062387309362
-58000000 0.0236225823558671
-57000000 -0.0353451569896902
-56000000 -0.0820417701911169
-55000000 -0.0146374313877988
-54000000 -0.00408622632524436
-53000000 -0.0193695245917116
-52000000 -0.021847291110301
-51000000 -0.00878363925090498
-50000000 -0.00669180369176731
-49000000 -0.123764351647047
-48000000 -0.2940978225191
-47000000 -0.176473376004274
-46000000 -0.0131683976751845
-45000000 0.000350165617764421
-44000000 -0.00215517072233149
-43000000 -0.0018110162973362
-42000000 -0.00139366539581829
-41000000 0.00605480193170054
-40000000 0.0450137137304624
-39000000 0.0539604653527066
-38000000 0.00428967684788039
-37000000 0.041615123330665
-36000000 0.199175014071561
-35000000 0.37046383664434
-34000000 0.487164159710203
-33000000 0.548091028523548
-32000000 0.57249756825357
-31000000 0.575959840098145
-30000000 0.569274984896288
-29000000 0.561619692933515
-28000000 0.560455427742318
-27000000 0.569272505165646
-26000000 0.586188290411734
-25000000 0.604985953613861
-24000000 0.618450453126821
-23000000 0.622184549452149
-22000000 0.616329291879795
-21000000 0.604255417789488
-20000000 0.589847302472949
-19000000 0.575626413444452
-18000000 0.562608594277852
-17000000 0.551332470560802
-16000000 0.542935737838311
-15000000 0.539423673523348
-14000000 0.542993845985238
-13000000 0.554918608733608
-12000000 0.574653004050463
-11000000 0.599639262651624
-10000000 0.625984346996674
-9000000 0.649798726024349
-8000000 0.668547808622032
-7000000 0.681669733839738
-6000000 0.690197129612722
-5000000 0.695789258046706
```

```
-4000000 0.699839325729588
-3000000 0.703067865741947
-2000000 0.705596877405071
-1000000 0.707250208702072
0 0.707827791165303
1000000 0.707250208702074
2000000 0.705596877405071
3000000 0.703067865741947
4000000 0.699839325729589
5000000 0.695789258046707
6000000 0.690197129612725
7000000 0.68166973383974
8000000 0.668547808622032
9000000 0.649798726024351
10000000 0.625984346996677
11000000 0.599639262651628
12000000 0.574653004050462
13000000 0.554918608733609
14000000 0.542993845985241
15000000 0.539423673523352
16000000 0.542935737838312
17000000 0.551332470560803
18000000 0.562608594277855
19000000 0.575626413444457
20000000 0.589847302472951
21000000 0.604255417789492
22000000 0.616329291879798
23000000 0.622184549452151
24000000 0.618450453126823
25000000 0.604985953613864
26000000 0.586188290411737
27000000 0.569272505165648
28000000 0.56045542774232
29000000 0.561619692933519
30000000 0.569274984896288
31000000 0.575959840098147
32000000 0.572497568253573
33000000 0.548091028523552
34000000 0.487164159710206
35000000 0.370463836644343
36000000 0.199175014071562
37000000 0.0416151233306655
38000000 0.00428967684787989
39000000 0.0539604653527066
40000000 0.0450137137304626
41000000 0.00605480193170057
42000000 -0.0013936653958183
43000000 -0.00181101629733629
44000000 -0.00215517072233157
45000000 0.000350165617764443
46000000 -0.0131683976751849
47000000 -0.176473376004275
48000000 -0.2940978225191
49000000 -0.123764351647046
50000000 -0.00669180369176618
51000000 -0.00878363925090411
52000000 -0.0218472911103002
53000000 -0.0193695245917105
54000000 -0.00408622632524374
55000000 -0.0146374313877976
56000000 -0.0820417701911164
57000000 -0.0353451569896902
58000000 0.0236225823558673
59000000 0.00185062387309372
60000000 -0.000706256001157743
```

For `split_order 3`:

```
-60000000 0.00699760366476518
-59000000 0.0085361663957035
-58000000 0.0398945884921854
-57000000 -0.0140645493492339
-56000000 -0.0017342146735783
-55000000 -0.00784444546650254
-54000000 -0.00618289329615022
```

-53000000 -0.0134501950880445
-52000000 -0.00752447475283041
-51000000 -0.00795590558411629
-50000000 -0.0135262768333751
-49000000 -0.00516899478665233
-48000000 -0.0104714395705434
-47000000 -0.0035691361486714
-46000000 -0.117658491635913
-45000000 -0.139962946159543
-44000000 -0.00136908208463075
-43000000 0.00267919169736106
-42000000 -3.96424893113342e-05
-41000000 -0.000507976120957025
-40000000 0.0189070264682524
-39000000 0.0606287231920644
-38000000 0.000249439525354438
-37000000 0.185047596610623
-36000000 0.538736679204008
-35000000 0.657585486054389
-34000000 0.592248923690434
-33000000 0.514133504136086
-32000000 0.48889222127871
-31000000 0.517079516795907
-30000000 0.57762342711142
-29000000 0.642414308498741
-28000000 0.689303380508347
-27000000 0.712637962009187
-26000000 0.719622817848674
-25000000 0.718219058135902
-24000000 0.710560798126534
-23000000 0.695364493672489
-22000000 0.673227323375442
-21000000 0.648488111195498
-20000000 0.626714239547487
-19000000 0.61121465135191
-18000000 0.601645880332769
-17000000 0.595220884076134
-16000000 0.589312272255043
-15000000 0.583625648460123
-14000000 0.580479108994844
-13000000 0.583154526411505
-12000000 0.593659980845251
-11000000 0.611340106865056
-10000000 0.632974914591004
-9000000 0.654207416948808
-8000000 0.671493123137568
-7000000 0.683421122768876
-6000000 0.690689936778134
-5000000 0.695031233649947
-4000000 0.69801181124524
-3000000 0.700430958994194
-2000000 0.702394588350416
-1000000 0.703702040492127
0 0.704160696160135
1000000 0.703702040492128
2000000 0.702394588350413
3000000 0.700430958994192
4000000 0.698011811245241
5000000 0.695031233649947
6000000 0.69068993677813
7000000 0.683421122768877
8000000 0.671493123137561
9000000 0.654207416948804
10000000 0.632974914591001
11000000 0.611340106865055
12000000 0.593659980845253
13000000 0.5831545264115
14000000 0.580479108994844
15000000 0.583625648460123
16000000 0.589312272255042
17000000 0.595220884076133
18000000 0.601645880332769
19000000 0.611214651351908
20000000 0.626714239547482
21000000 0.648488111195497
22000000 0.673227323375436

```
23000000 0.695364493672483
24000000 0.710560798126536
25000000 0.7182190581359
26000000 0.719622817848672
27000000 0.712637962009186
28000000 0.689303380508343
29000000 0.642414308498739
30000000 0.577623427111412
31000000 0.517079516795905
32000000 0.488892221278708
33000000 0.514133504136083
34000000 0.592248923690433
35000000 0.657585486054392
36000000 0.53873667920401
37000000 0.185047596610622
38000000 0.000249439525353273
39000000 0.0606287231920628
40000000 0.0189070264682507
41000000 -0.000507976120957247
42000000 -3.9642489311556e-05
43000000 0.00267919169735944
44000000 -0.00136908208463106
45000000 -0.139962946159544
46000000 -0.117658491635915
47000000 -0.00356913614867241
48000000 -0.010471439570546
49000000 -0.005168994786654
50000000 -0.0135262768333746
51000000 -0.00795590558411606
52000000 -0.00752447475282962
53000000 -0.0134501950880436
54000000 -0.00618289329614949
55000000 -0.00784444546650132
56000000 -0.00173421467357771
57000000 -0.014064549349234
58000000 0.0398945884921855
59000000 0.0085361663957035
60000000 0.00699760366476613
```

For `split_order 4`:

```
-60000000 0.041822843545657
-59000000 0.0166615541523858
-58000000 0.0325578451520113
-57000000 0.0355285573451099
-56000000 -0.0164551398024361
-55000000 -0.00692836157904716
-54000000 -0.00801548024092936
-53000000 -0.00411959470796778
-52000000 -0.0160224962723219
-51000000 -0.0176112968139514
-50000000 -0.0150719843382416
-49000000 -0.00236456973937914
-48000000 -0.0139570128141827
-47000000 -0.00879824166864507
-46000000 -0.0955731235655738
-45000000 -0.202340222598282
-44000000 -0.0137424193879685
-43000000 0.00180378899769295
-42000000 -0.000906518954564221
-41000000 0.00105180161985448
-40000000 0.00089804933017397
-39000000 0.0501485477975539
-38000000 0.0360078929738678
-37000000 0.0333257008178276
-36000000 0.340066829663192
-35000000 0.618573813041803
-34000000 0.670081360123459
-33000000 0.620117458156088
-32000000 0.582102728371439
-31000000 0.58630620429965
-30000000 0.622195085201592
-29000000 0.666735302212594
-28000000 0.700515982566903
-27000000 0.717292240094268
```

```
-26000000 0.721655969751974
-25000000 0.719357443503745
-24000000 0.711525322937695
-23000000 0.696513354796851
-22000000 0.674626871825957
-21000000 0.649927785918237
-20000000 0.627892696908335
-19000000 0.611962048380333
-18000000 0.602015369179838
-17000000 0.595420948254939
-16000000 0.589555638681555
-15000000 0.584008263766975
-14000000 0.580965166737312
-13000000 0.583649231368403
-12000000 0.594091001784574
-11000000 0.611689429329299
-10000000 0.63325790933919
-9000000 0.6544330083941
-8000000 0.67164373774839
-7000000 0.683466330962737
-6000000 0.690614729091889
-5000000 0.694850452878654
-4000000 0.697761109609433
-3000000 0.700146686897544
-2000000 0.702099957389875
-1000000 0.703406212096697
0 0.703865132214863
1000000 0.703406212096698
2000000 0.70209995738988
3000000 0.700146686897545
4000000 0.697761109609436
5000000 0.694850452878659
6000000 0.690614729091894
7000000 0.683466330962739
8000000 0.671643737748393
9000000 0.654433008394105
10000000 0.633257909339193
11000000 0.611689429329303
12000000 0.594091001784578
13000000 0.583649231368407
14000000 0.580965166737314
15000000 0.584008263766978
16000000 0.589555638681559
17000000 0.59542094825494
18000000 0.60201536917984
19000000 0.611962048380336
20000000 0.62789269690834
21000000 0.649927785918238
22000000 0.674626871825962
23000000 0.696513354796851
24000000 0.711525322937702
25000000 0.719357443503748
26000000 0.72165596975198
27000000 0.717292240094268
28000000 0.700515982566906
29000000 0.666735302212596
30000000 0.622195085201588
31000000 0.586306204299649
32000000 0.58210272837144
33000000 0.620117458156085
34000000 0.670081360123458
35000000 0.618573813041801
36000000 0.340066829663192
37000000 0.0333257008178258
38000000 0.0360078929738661
39000000 0.0501485477975535
40000000 0.000898049330172662
41000000 0.00105180161985375
42000000 -0.000906518954565055
43000000 0.00180378899769266
44000000 -0.0137424193879704
45000000 -0.202340222598285
46000000 -0.0955731235655748
47000000 -0.00879824166864697
48000000 -0.0139570128141829
49000000 -0.00236456973937882
```

```
50000000 -0.0150719843382415
51000000 -0.0176112968139514
52000000 -0.0160224962723213
53000000 -0.00411959470796738
54000000 -0.00801548024092911
55000000 -0.00692836157904678
56000000 -0.0164551398024357
57000000 0.0355285573451098
58000000 0.032557845152012
59000000 0.0166615541523862
60000000 0.0418228435456585
```

For `split_order 5`:

```
-60000000 0.0371092229913348
-59000000 0.0146248439524267
-58000000 0.0334777488766596
-57000000 0.030132923600272
-56000000 -0.0143093893346153
-55000000 -0.0092647179524208
-54000000 -0.0054994843373599
-53000000 -0.00611531683422001
-52000000 -0.0166530734628857
-51000000 -0.0173297046039788
-50000000 -0.0154252907075169
-49000000 -0.00273301442325934
-48000000 -0.0133986215891951
-47000000 -0.00833958056116862
-46000000 -0.0976146551915587
-45000000 -0.196097229969455
-44000000 -0.0119371162896389
-43000000 0.00185648371650128
-42000000 -0.000795633328606441
-41000000 0.000774042117265227
-40000000 0.00185689729038056
-39000000 0.0531217272644116
-38000000 0.0308512702178929
-37000000 0.0436467472177524
-36000000 0.36332391259381
-35000000 0.628515790426714
-34000000 0.665565462593777
-33000000 0.610460782668032
-32000000 0.57282108737182
-31000000 0.579230291822018
-30000000 0.617607241694532
-29000000 0.664231633818773
-28000000 0.699372896797054
-27000000 0.716834139942018
-26000000 0.721469217569325
-25000000 0.719256830031601
-24000000 0.711433400106836
-23000000 0.696393539096085
-22000000 0.674474909686998
-21000000 0.649769167243341
-20000000 0.627762075668107
-19000000 0.61187896186224
-18000000 0.60197428844279
-17000000 0.595398840441842
-16000000 0.589528812776878
-15000000 0.583965983794781
-14000000 0.580911486169936
-13000000 0.583594918066868
-12000000 0.594044330029998
-11000000 0.611652458619143
-10000000 0.633228741604385
-9000000 0.654410301324348
-8000000 0.671629108376369
-7000000 0.683462977365115
-6000000 0.690624312758814
-5000000 0.694871432723964
-4000000 0.697789668041526
-3000000 0.7001789107621
-2000000 0.702133348221949
-1000000 0.703439777555787
0 0.703898688444742
```

```
1000000 0.70343977755579
2000000 0.702133348221954
3000000 0.700178910762099
4000000 0.697789668041524
5000000 0.69487143272396
6000000 0.69062431275882
7000000 0.683462977365109
8000000 0.671629108376372
9000000 0.654410301324355
10000000 0.633228741604382
11000000 0.611652458619137
12000000 0.594044330030006
13000000 0.583594918066863
14000000 0.58091148616994
15000000 0.583965983794779
16000000 0.589528812776882
17000000 0.595398840441851
18000000 0.601974288442799
19000000 0.611878961862252
20000000 0.627762075668116
21000000 0.649769167243338
22000000 0.674474909687003
23000000 0.696393539096091
24000000 0.711433400106837
25000000 0.7192568300316
26000000 0.721469217569319
27000000 0.71683413994202
28000000 0.699372896797055
29000000 0.664231633818769
30000000 0.617607241694527
31000000 0.579230291822008
32000000 0.572821087371821
33000000 0.610460782668037
34000000 0.665565462593778
35000000 0.62851579042672
36000000 0.363323912593819
37000000 0.0436467472177556
38000000 0.0308512702178945
39000000 0.0531217272644128
40000000 0.00185689729038131
41000000 0.000774042117265991
42000000 -0.000795633328606029
43000000 0.0018564837165037
44000000 -0.0119371162896358
45000000 -0.196097229969451
46000000 -0.0976146551915555
47000000 -0.00833958056116531
48000000 -0.0133986215891882
49000000 -0.00273301442325577
50000000 -0.0154252907075158
51000000 -0.017329704603979
52000000 -0.0166530734628871
53000000 -0.0061153168342211
54000000 -0.0054994843373618
55000000 -0.00926471795242184
56000000 -0.0143093893346154
57000000 0.0301329236002715
58000000 0.03347774887666
59000000 0.0146248439524266
60000000 0.0371092229913339
```

For `split_order 6`:

```
-60000000 0.0417162135496055
-59000000 0.0166294631571311
-58000000 0.0325444494968081
-57000000 0.0354801357391893
-56000000 -0.0163761296167724
-55000000 -0.00698616329063621
-54000000 -0.00790809556934238
-53000000 -0.00420931781717247
-52000000 -0.0160710277514141
-51000000 -0.0176039933756728
-50000000 -0.0151428895229539
-49000000 -0.00245134449239175
```

```
-48000000 -0.0137650352497445
-47000000 -0.0089741336512546
-46000000 -0.0947292772893488
-45000000 -0.202578997601279
-44000000 -0.0138895406759798
-43000000 0.00181838331336405
-42000000 -0.000904785723860458
-41000000 0.00105550194118456
-40000000 0.000886454419953375
-39000000 0.0501142606372391
-38000000 0.0360308140146462
-37000000 0.0333395516612939
-36000000 0.340254681389911
-35000000 0.618740212804732
-34000000 0.670001361546073
-33000000 0.619831808496602
-32000000 0.58172887231417
-31000000 0.585935404364763
-30000000 0.621891471224142
-29000000 0.666535106206008
-28000000 0.700418057849658
-27000000 0.717265782086573
-26000000 0.721664226860378
-25000000 0.719375115154844
-24000000 0.711540824920385
-23000000 0.696523290975894
-22000000 0.674631044443423
-21000000 0.64992736573499
-20000000 0.627890080812452
-19000000 0.611960501916098
-18000000 0.602017936321419
-17000000 0.595429147112872
-16000000 0.589568767763656
-15000000 0.584023853701101
-14000000 0.580980297295518
-13000000 0.583661799454227
-12000000 0.594100245822857
-11000000 0.611695693680394
-10000000 0.6332620323865
-9000000 0.654435739091443
-8000000 0.671645448223624
-7000000 0.683467071995696
-6000000 0.690614455182816
-5000000 0.694849193902439
-4000000 0.697758999781392
-3000000 0.70014390905716
-2000000 0.702096696034205
-1000000 0.703402650851906
0 0.703861467955302
1000000 0.703402650851905
2000000 0.702096696034207
3000000 0.700143909057165
4000000 0.697758999781399
5000000 0.694849193902442
6000000 0.690614455182823
7000000 0.683467071995702
8000000 0.67164544822363
9000000 0.654435739091441
10000000 0.633262032386506
11000000 0.611695693680402
12000000 0.594100245822861
13000000 0.583661799454232
14000000 0.580980297295524
15000000 0.584023853701107
16000000 0.589568767763665
17000000 0.595429147112877
18000000 0.602017936321425
19000000 0.611960501916104
20000000 0.627890080812458
21000000 0.649927365735003
22000000 0.674631044443427
23000000 0.696523290975899
24000000 0.711540824920386
25000000 0.719375115154851
26000000 0.721664226860383
27000000 0.717265782086577
```

```
28000000 0.700418057849662
29000000 0.666535106206012
30000000 0.621891471224146
31000000 0.585935404364759
32000000 0.581728872314168
33000000 0.6198318084966
34000000 0.670001361546075
35000000 0.618740212804734
36000000 0.340254681389909
37000000 0.0333395516612922
38000000 0.0360308140146436
39000000 0.0501142606372374
40000000 0.000886454419952069
41000000 0.00105550194118398
42000000 -0.000904785723861385
43000000 0.00181838331336391
44000000 -0.0138895406759815
45000000 -0.202578997601283
46000000 -0.0947292772893503
47000000 -0.00897413365125533
48000000 -0.0137650352497463
49000000 -0.00245134449239242
50000000 -0.0151428895229551
51000000 -0.0176039933756733
52000000 -0.016071027751414
53000000 -0.00420931781717235
54000000 -0.00790809556934239
55000000 -0.00698616329063643
56000000 -0.0163761296167717
57000000 0.0354801357391885
58000000 0.0325444494968089
59000000 0.0166294631571308
60000000 0.0417162135496072
```

SIMPSON-v6.0 uses `maxdt` as an effective Trotterisation, and for `maxdt 0.025`, this sets a Trotter number to 2. The results for this, using `split_order 2` are:

```
-60000000 0.0285108954928163
-59000000 0.0122169373994906
-58000000 0.0365807105747476
-57000000 0.0195562125345055
-56000000 -0.0203343988722802
-55000000 -0.00696826299014099
-54000000 -0.0155023513929918
-53000000 -0.000475065914849324
-52000000 -0.00547009965175795
-51000000 -0.00638644954308901
-50000000 -0.000869902834683253
-49000000 -0.0126659915407817
-48000000 -0.0227580213575549
-47000000 -0.0198219492389438
-46000000 -0.233332860343463
-45000000 -0.102934784893922
-44000000 0.00271857780952274
-43000000 -0.000351285767226073
-42000000 -0.000752489303695089
-41000000 -0.000260749777626698
-40000000 0.00779384193123189
-39000000 0.060462305682606
-38000000 0.0230696179023575
-37000000 0.0435636025003289
-36000000 0.320925219515719
-35000000 0.581095650447795
-34000000 0.672464038836409
-33000000 0.671570570821386
-32000000 0.661361813841166
-31000000 0.668922381835065
-30000000 0.688344938607169
-29000000 0.70543294491438
-28000000 0.712484704395918
-27000000 0.711661659461444
-26000000 0.708742275820326
-25000000 0.705922672491102
-24000000 0.700445634394333
```

-23000000 0.688524792332562
-22000000 0.66969742522849
-21000000 0.647549355667399
-20000000 0.626925686028614
-19000000 0.610763373300237
-18000000 0.599002325926585
-17000000 0.589775466019881
-16000000 0.581621811346799
-15000000 0.575082209631748
-14000000 0.572606850237592
-13000000 0.576990232191917
-12000000 0.589517865387879
-11000000 0.608941707463336
-10000000 0.631762202206186
-9000000 0.653655109271078
-8000000 0.671286878608322
-7000000 0.683460105510676
-6000000 0.69098246578979
-5000000 0.695593891624535
-4000000 0.698830192715906
-3000000 0.701467197983655
-2000000 0.703600747667584
-1000000 0.705019976940483
0 0.705518265527258
1000000 0.705019976940488
2000000 0.703600747667585
3000000 0.701467197983656
4000000 0.698830192715907
5000000 0.695593891624535
6000000 0.690982465789797
7000000 0.68346010551068
8000000 0.671286878608322
9000000 0.65365510927108
10000000 0.631762202206189
11000000 0.608941707463341
12000000 0.589517865387876
13000000 0.576990232191917
14000000 0.572606850237595
15000000 0.575082209631753
16000000 0.581621811346799
17000000 0.589775466019883
18000000 0.599002325926588
19000000 0.610763373300242
20000000 0.626925686028615
21000000 0.647549355667402
22000000 0.66969742522849
23000000 0.688524792332563
24000000 0.700445634394334
25000000 0.705922672491101
26000000 0.708742275820327
27000000 0.711661659461445
28000000 0.712484704395921
29000000 0.705432944914386
30000000 0.688344938607169
31000000 0.668922381835065
32000000 0.661361813841169
33000000 0.67157057082139
34000000 0.672464038836411
35000000 0.581095650447801
36000000 0.320925219515722
37000000 0.0435636025003296
38000000 0.0230696179023576
39000000 0.0604623056826069
40000000 0.00779384193123234
41000000 -0.000260749777626455
42000000 -0.000752489303695439
43000000 -0.000351285767225859
44000000 0.00271857780952143
45000000 -0.102934784893922
46000000 -0.233332860343464
47000000 -0.0198219492389433
48000000 -0.0227580213575546
49000000 -0.0126659915407806
50000000 -0.000869902834683668
51000000 -0.00638644954308914
52000000 -0.00547009965175769

```
53000000 -0.000475065914849476
54000000 -0.0155023513929925
55000000 -0.00696826299014083
56000000 -0.0203343988722803
57000000 0.0195562125345056
58000000 0.0365807105747486
59000000 0.0122169373994907
60000000 0.0285108954928166
```

For `split_order 3`:

```
-60000000 0.0314487553256498
-59000000 0.0125754897034225
-58000000 0.0348359561184864
-57000000 0.0229058160637517
-56000000 -0.011109182469947
-55000000 -0.0118239546220906
-54000000 -0.00295134856184118
-53000000 -0.00859159922940466
-52000000 -0.0168125990926805
-51000000 -0.0166783354227772
-50000000 -0.0156108756625939
-49000000 -0.00306086827725625
-48000000 -0.0130107711124561
-47000000 -0.00751946468540392
-46000000 -0.101331938396023
-45000000 -0.187882521500123
-44000000 -0.00972324514246131
-43000000 0.00191836540364189
-42000000 -0.000668356557478449
-41000000 0.00044115004881477
-40000000 0.00338566073980368
-39000000 0.0563821845251223
-38000000 0.0244697701994355
-37000000 0.0584642791089041
-36000000 0.39168446032625
-35000000 0.638855064912306
-34000000 0.658748418244102
-33000000 0.59820246151982
-32000000 0.561476550428608
-31000000 0.570748842585508
-30000000 0.612189807603154
-29000000 0.661312311173107
-28000000 0.698042880955238
-27000000 0.716282105727297
-26000000 0.721219958691702
-25000000 0.719108020744807
-24000000 0.711301411352827
-23000000 0.696235931265338
-22000000 0.674285411401895
-21000000 0.649576837662878
-20000000 0.627606406413544
-19000000 0.611780458727079
-18000000 0.601923247862258
-17000000 0.595365729672385
-16000000 0.589485396925626
-15000000 0.58390142420057
-14000000 0.580833301303807
-13000000 0.583517989480921
-12000000 0.593979282644517
-11000000 0.61160143567263
-10000000 0.633188760049499
-9000000 0.654379251242088
-8000000 0.671608850784429
-7000000 0.683457521494208
-6000000 0.690635773961629
-5000000 0.694897867122376
-4000000 0.697826222284875
-3000000 0.70022057314402
-2000000 0.702176857125233
-1000000 0.703483743183657
0 0.703942723189202
1000000 0.703483743183657
2000000 0.702176857125227
3000000 0.700220573144015
```

```
4000000 0.697826222284874
5000000 0.694897867122377
6000000 0.690635773961623
7000000 0.683457521494209
8000000 0.671608850784418
9000000 0.654379251242081
10000000 0.633188760049492
11000000 0.611601435672627
12000000 0.59397928264452
13000000 0.583517989480912
14000000 0.580833301303809
15000000 0.583901424200569
16000000 0.589485396925623
17000000 0.595365729672384
18000000 0.601923247862257
19000000 0.611780458727074
20000000 0.627606406413536
21000000 0.649576837662875
22000000 0.674285411401886
23000000 0.696235931265329
24000000 0.711301411352836
25000000 0.719108020744805
26000000 0.721219958691697
27000000 0.716282105727296
28000000 0.698042880955228
29000000 0.661312311173103
30000000 0.612189807603142
31000000 0.570748842585506
32000000 0.561476550428607
33000000 0.598202461519818
34000000 0.6587484182441
35000000 0.638855064912319
36000000 0.391684460326252
37000000 0.0584642791089014
38000000 0.0244697701994331
39000000 0.0563821845251188
40000000 0.00338566073980062
41000000 0.000441150048813594
42000000 -0.000668356557479274
43000000 0.00191836540363896
44000000 -0.0097232451424621
45000000 -0.187882521500123
46000000 -0.101331938396028
47000000 -0.00751946468540506
48000000 -0.0130107711124597
49000000 -0.00306086827725912
50000000 -0.0156108756625938
51000000 -0.016678335422777
52000000 -0.016812599092679
53000000 -0.00859159922940288
54000000 -0.00295134856183982
55000000 -0.0118239546220886
56000000 -0.011109182469946
57000000 0.0229058160637516
58000000 0.0348359561184856
59000000 0.0125754897034229
60000000 0.0314487553256521
```

For `maxdt 0.0125`, Trotter number 4, the `split_order 2` results are:

```
-60000000 0.0389421762547165
-59000000 0.015439590591148
-58000000 0.0337975520854827
-57000000 0.031894749591263
-56000000 -0.0172011277942974
-55000000 -0.0072042641221427
-54000000 -0.00940095609704309
-53000000 -0.00274583191454884
-52000000 -0.0145341771263412
-51000000 -0.0168798911687281
-50000000 -0.0118386883735368
-49000000 -0.00036222598806419
-48000000 -0.0208662246442558
-47000000 -0.00182162116247076
-46000000 -0.134377884329402
```

-45000000 -0.182372428631621
-44000000 -0.00668098260471749
-43000000 0.0011709961590283
-42000000 -0.000885934022906147
-41000000 0.000761071893050916
-40000000 0.00207805943229202
-39000000 0.05333833777041
-38000000 0.0325572507782282
-37000000 0.0362553730873388
-36000000 0.336595586768905
-35000000 0.610845502463777
-34000000 0.673388849857859
-33000000 0.636524847910476
-32000000 0.606001135964716
-31000000 0.611623859597472
-30000000 0.643806120721432
-29000000 0.681269247655648
-28000000 0.707484465359298
-27000000 0.718738742268529
-26000000 0.720349987190344
-25000000 0.717317728264545
-24000000 0.709730356461123
-23000000 0.695298179560024
-22000000 0.674064019986173
-21000000 0.649937403816065
-20000000 0.628216407266543
-19000000 0.612193630351108
-18000000 0.601741781810661
-17000000 0.594408464895766
-16000000 0.587867849737528
-15000000 0.581968525417277
-14000000 0.578984519709827
-13000000 0.582040982206316
-12000000 0.592978752689616
-11000000 0.611025515168772
-10000000 0.632906992324527
-9000000 0.654263332390634
-8000000 0.671580502355633
-7000000 0.6834914472694
-6000000 0.690734290139185
-5000000 0.69506545904239
-4000000 0.698059472183107
-3000000 0.70051002064147
-2000000 0.702510358485196
-1000000 0.703846346438042
0 0.704315668780402
1000000 0.703846346438051
2000000 0.702510358485199
3000000 0.700510020641471
4000000 0.698059472183107
5000000 0.695065459042392
6000000 0.6907342901392
7000000 0.683491447269409
8000000 0.671580502355632
9000000 0.654263332390639
10000000 0.632906992324534
11000000 0.611025515168781
12000000 0.592978752689611
13000000 0.582040982206316
14000000 0.578984519709833
15000000 0.581968525417288
16000000 0.58786784973753
17000000 0.594408464895768
18000000 0.601741781810666
19000000 0.612193630351117
20000000 0.628216407266546
21000000 0.649937403816069
22000000 0.674064019986174
23000000 0.695298179560027
24000000 0.709730356461126
25000000 0.717317728264545
26000000 0.720349987190346
27000000 0.718738742268527
28000000 0.7074844653593
29000000 0.68126924765565
30000000 0.643806120721425

```
31000000 0.611623859597469
32000000 0.606001135964715
33000000 0.636524847910477
34000000 0.673388849857857
35000000 0.610845502463784
36000000 0.336595586768907
37000000 0.0362553730873377
38000000 0.0325572507782259
39000000 0.0533383377704089
40000000 0.00207805943229139
41000000 0.000761071893050386
42000000 -0.000885934022907383
43000000 0.00117099615902924
44000000 -0.00668098260472151
45000000 -0.18237242863162
46000000 -0.134377884329404
47000000 -0.0018216211624705
48000000 -0.0208662246442544
49000000 -0.000362225988062662
50000000 -0.0118386883735383
51000000 -0.0168798911687282
52000000 -0.0145341771263411
53000000 -0.00274583191454877
54000000 -0.00940095609704461
55000000 -0.00720426412214223
56000000 -0.0172011277942974
57000000 0.0318947495912627
58000000 0.0337975520854836
59000000 0.015439590591148
60000000 0.0389421762547169
```

# 6 Optimal control with pulse transients

Optimal control calculation presented in the main text Figure 7 takes into account a model of pulse transients and it is conducted using the input file

```
spinsys {
    channels     e
    nuclei       e 1H
    gtensor      1 1e6 0 0 0 0 0
    hyperfine    1 2 0 0.8676e6  0 60 0
}

par {
    proton_frequency    14.8e+6
    crystal_file        alpha0beta0
    gamma_angles        1
    averaging_file      gtensor_1_iso_120MHz.ave
    sw                  1e9
    start_operator      I1x
    detect_operator     -I2z
    method              DNPframe prop_split
    split_order 2

    # Parameters for optimisation
    conjugate_fid       false
    oc_grad_level       2
    oc_max_iter         500
    oc_tol_cg           1e-9
}

proc pulseq {} {
    global shpdist duration
    reset
    pulse_shaped $duration $shpdist
    oc_acq_hermit
}

proc gradient {} {
    global par shp dop shpdist

    # create distorted shape, prepare gradient
    distort_shape $dop $shp $shpdist
    # we optimize non-distorted shp but calculate grard wrt distorted shpdist
```

```
    oc_grad_shapes $shpdist
    set par(np) [shape_len $shpdist]
    set g [fsimpson]

    # reconstruct grads w.r.t. original shape shp
    set gg [fcreate -np [shape_len $shp] -sw $par(sw)]
    reconstruct_gradient $g $gg $dop
    funload $g

    return $gg
}

proc target_function {} {
    global par shp dop shpdist

    # create distorted shape
    distort_shape $dop $shp $shpdist
    set par(np) 1

    # calculate target
    set f [fsimpson]
    set Resn [expr [findex $f 1 -re] ]
    funload $f

    return [format "%.20f" $Resn]
}

proc main {} {
    global shp dop shpdist duration

    # time resolution of non-distorted shape is 1 ns (each element is 1 ns)
    set t 0.001
    set shp [load_shape shape_oc_initial.dat]
    set Nshp [shape_len $shp]
    set duration [expr $Nshp*$t]

    # discretised distortion operator with time resolution of 0.5ns
    set dt [expr $t/2.0]
    # discretized distortion operators
    set dop [create_distortion_operator Rsp.dat $dt $Nshp $t]
    # allocate distorted shape with Nshpdist elements
    set Nshpdist [expr int($Nshp*$t/$dt)]
    set shpdist [shape_create $Nshpdist]

    # optimisation
    set tfopt [oc_optimize $shp -max 32e6]

    free_distortion_operator $dop
    free_all_shapes
}
```

The offset range is defined as the `averaging_file` `gtensor_1_iso_120MHz.ave`:

```
gtensor_1_iso           weight
    +60000000   0.016393442623
    +58000000   0.016393442623
    +56000000   0.016393442623
    +54000000   0.016393442623
    +52000000   0.016393442623
    +50000000   0.016393442623
    +48000000   0.016393442623
    +46000000   0.016393442623
    +44000000   0.016393442623
    +42000000   0.016393442623
    +40000000   0.016393442623
    +38000000   0.016393442623
    +36000000   0.016393442623
    +34000000   0.016393442623
    +32000000   0.016393442623
    +30000000   0.016393442623
    +28000000   0.016393442623
    +26000000   0.016393442623
    +24000000   0.016393442623
    +22000000   0.016393442623
    +20000000   0.016393442623
```

```
+18000000   0.016393442623
+16000000   0.016393442623
+14000000   0.016393442623
+12000000   0.016393442623
+10000000   0.016393442623
 +8000000   0.016393442623
 +6000000   0.016393442623
 +4000000   0.016393442623
 +2000000   0.016393442623
       +0   0.016393442623
 -2000000   0.016393442623
 -4000000   0.016393442623
 -6000000   0.016393442623
 -8000000   0.016393442623
-10000000   0.016393442623
-12000000   0.016393442623
-14000000   0.016393442623
-16000000   0.016393442623
-18000000   0.016393442623
-20000000   0.016393442623
-22000000   0.016393442623
-24000000   0.016393442623
-26000000   0.016393442623
-28000000   0.016393442623
-30000000   0.016393442623
-32000000   0.016393442623
-34000000   0.016393442623
-36000000   0.016393442623
-38000000   0.016393442623
-40000000   0.016393442623
-42000000   0.016393442623
-44000000   0.016393442623
-46000000   0.016393442623
-48000000   0.016393442623
-50000000   0.016393442623
-52000000   0.016393442623
-54000000   0.016393442623
-56000000   0.016393442623
-58000000   0.016393442623
-60000000   0.016393442623
```

The initial shape for optimisation was obtained in a separate calculation that ignored pulse transients and it is stored in the `shape_oc_initial.dat` file:

```
31957442.4894379    -4.27404861262645
32000000            -6.78202890632305
31998606.0148436    -7.93075603444182
31877919.7978521    -8.44664854666366
31682287.5675026    -8.32759890502926
31463603.7927394    -7.2404510199456
31311114.0234222    -3.33130991404044
20222564.9607153    -3.53520923602843
7685802.17460973    -3.26885030852931
789588.386625434    54.5142557499533
3302471.62672317    139.717044362743
25068510.3373082    172.209871109119
27481493.9630469    172.657054380511
25250134.2188636    170.728235722178
23214513.2212744    168.252589546998
21485674.9647708    165.215653527394
17341807.7344187    157.632952830186
15181321.7670882    146.107684135064
18990827.9242687    144.21118237783
28464805.8425915    150.415550980035
31999016.3814229    150.561620162025
31999000.033698     151.397397900264
31999232.2489808    153.169391188157
31999645.043832     154.459776498776
32000000            155.838627015234
32000000            157.642478258701
32000000            160.100103034134
32000000            163.845082915392
31999968.5568881    170.448092532534
19627008.5057139    -175.110704015905
```

| | |
|---|---|
| 31242938.2928043 | 2.24958498723615 |
| 32000000 | 12.3579083624253 |
| 32000000 | 15.0113522277716 |
| 32000000 | 14.4290747577455 |
| 32000000 | 12.6393694692078 |
| 32000000 | 10.6799786187225 |
| 32000000 | 9.07462160583345 |
| 32000000 | 8.04671994950632 |
| 32000000 | 7.65749463152889 |
| 32000000 | 7.91824872039565 |
| 32000000 | 8.88368736635583 |
| 32000000 | 10.7178707802784 |
| 32000000 | 13.6996647125217 |
| 32000000 | 18.1021119846857 |
| 32000000 | 23.9326503214578 |
| 31979691.1179763 | 30.8644290393789 |
| 29832831.2424209 | 38.0119386773113 |
| 27716712.2150648 | 43.5455848848903 |
| 26438937.0565863 | 46.4181334085167 |
| 21012627.5270785 | 114.718953038512 |
| 31999782.5823298 | 153.94070612562 |
| 31999443.1604661 | 158.97515697282 |
| 28854809.5138532 | 158.04225512325 |
| 8845246.03971577 | 92.7906608481789 |
| 21008318.7900676 | 23.5191028306642 |
| 21091486.7892378 | 24.4301758035109 |
| 21439628.5395426 | 26.325494217638 |
| 22252946.4674471 | 29.1454363748432 |
| 23671898.1530862 | 32.3871013399652 |
| 25684889.9939528 | 35.3371419028559 |
| 28080408.502097 | 37.3294599817844 |
| 30268289.6098436 | 37.4782006887073 |
| 31625439.2340527 | 35.6889869521162 |
| 31767919.0915348 | 32.6153921152107 |
| 28232572.2989687 | 29.7590484737226 |
| 18583399.6043395 | 30.8816172936417 |
| 5771488.5294041 | 63.2183291052822 |
| 16342128.6429513 | 172.591724249823 |
| 32000000 | 178.962587957147 |
| 32000000 | 177.226802784233 |
| 32000000 | 175.939914179235 |
| 32000000 | 174.612794211925 |
| 32000000 | 172.245679330283 |
| 32000000 | 167.410348964432 |
| 32000000 | 157.394766892905 |
| 30135191.1805209 | 75.3358691210855 |
| 31885871.6188293 | 27.3989456979128 |
| 31999288.0329428 | 11.0992649009367 |
| 32000000 | 3.52435719659932 |
| 32000000 | 0.406224730324011 |
| 32000000 | -0.725214980187703 |
| 32000000 | -0.992714867421246 |
| 32000000 | -0.852238083854566 |
| 32000000 | -0.445100888345061 |
| 32000000 | 0.210051800839661 |
| 32000000 | 0.972040046423212 |
| 31999287.0989906 | 1.04548758077611 |
| 31459587.8501836 | -1.86878984634049 |
| 29767853.1863454 | -11.5562807319055 |
| 18440788.0258556 | -42.0639683432386 |
| 18287389.0575552 | -134.95183890859 |
| 14518477.6021321 | -134.840086934318 |
| 20729366.0962864 | -29.0451190939773 |
| 32000000 | -16.7037542615424 |
| 32000000 | -19.5226601656638 |
| 32000000 | -20.7443369468937 |
| 32000000 | -21.7499128479686 |
| 32000000 | -23.0481571800216 |
| 32000000 | -24.724630491526 |
| 32000000 | -26.7077324375045 |
| 32000000 | -28.8401036195003 |
| 31999697.1783212 | -30.9051433076846 |
| 31999053.4602398 | -32.8429641312664 |
| 31998446.8746337 | -40.6454314933364 |
| 19759459.2047097 | -83.2747563359851 |
| 15788951.1333689 | -105.180773043308 |

| | |
|---|---|
| 12316882.5756992 | -79.5216673843129 |
| 14497920.3476068 | -42.5387522169162 |
| 26633533.0594344 | -16.688484328578 |
| 30983982.0519159 | -9.29113901772093 |
| 32000000 | -3.19114024671547 |
| 32000000 | 1.73948309625579 |
| 32000000 | 5.64085543438136 |
| 32000000 | 8.99786539793897 |
| 32000000 | 12.3709564152375 |
| 30821400.9133371 | 18.108930278893 |
| 31888415.2264492 | 164.280543489216 |
| 31998915.7942523 | 166.542873007747 |
| 31999804.7453885 | 168.472989271858 |
| 31999954.1918431 | 169.413686294733 |
| 31999981.5257794 | 169.125600164137 |
| 31999883.4189582 | 167.464457354465 |
| 31999693.2596178 | 164.282910439626 |
| 31998388.3209589 | 159.621335224271 |
| 31908899.8529551 | 154.117725716754 |
| 31833256.4564186 | 149.10521604665 |
| 23868552.6581055 | 136.236414965286 |
| 16369280.4199661 | 69.0013319069026 |
| 25556252.7948469 | 36.398887103685 |
| 31368040.7948804 | 28.9884340986957 |
| 30492899.0939627 | 27.7151916058586 |
| 30100283.5499058 | 27.9274639254075 |
| 24745322.0955097 | 30.3325801958529 |
| 16342272.7436155 | 35.5299267833016 |
| 6514936.21147373 | 60.274641013103 |
| 13106803.1188765 | 8.76507287473372 |
| 14530136.5685228 | -2.88953344248662 |
| 18513173.6535576 | -8.31149972007076 |
| 21400868.7880301 | -9.98887835322542 |
| 28739273.8166579 | -5.90827953663798 |
| 30235090.3061992 | -1.73019862631132 |
| 32000000 | 2.82368544868418 |
| 32000000 | 7.09223939876161 |
| 32000000 | 10.7032714359722 |
| 32000000 | 13.5693577794695 |
| 32000000 | 15.8381374839809 |
| 32000000 | 17.7892841136186 |
| 32000000 | 19.716380098894 |
| 32000000 | 21.8868608519847 |
| 32000000 | 24.6304008043799 |
| 32000000 | 28.6380094764873 |
| 32000000 | 35.8152470449062 |
| 22951654.4289804 | 56.2290068481708 |
| 31999447.1145721 | 158.172178056895 |
| 31999776.703335 | 164.360140320128 |
| 32000000 | 168.580404359186 |
| 32000000 | 171.400261711375 |
| 32000000 | 172.800467699498 |
| 32000000 | 172.765726071267 |
| 32000000 | 171.171616881305 |
| 32000000 | 165.005134114418 |
| 18607630.969687 | 111.527856748571 |
| 23283888.1252057 | 59.2838858839613 |
| 31999073.5759317 | 36.5231376512378 |
| 31999103.7452788 | 28.4081074388993 |
| 31999157.7434212 | 23.6021366856199 |
| 31999143.2286678 | 20.572069149916 |
| 31986928.9834642 | 18.9294173690929 |
| 31943636.9505651 | 18.366616771748 |
| 31822613.2313435 | 18.5369898093872 |
| 31671721.0728303 | 18.8864833257058 |
| 31524183.3145153 | 18.6052147394216 |
| 30602663.3105234 | 16.3624465746368 |
| 22826858.0418555 | 15.2146400907211 |
| 3285459.42461435 | 72.7913165026686 |
| 16463868.561109 | 173.568857205803 |
| 29200839.3014696 | 177.023388289692 |
| 31825001.6427928 | 177.504235858955 |
| 31648884.8356012 | 177.612557977418 |
| 27020989.1793323 | 178.278834637825 |
| 14638049.9010417 | -175.583422282191 |
| 9816648.30296307 | -160.622557703874 |

| | |
|---|---|
| 4720615.13229782 | -102.100287323905 |
| 12949385.2688362 | -26.4676466073889 |
| 25153903.1849089 | -16.6912876138545 |
| 25535830.9888872 | -18.847628745481 |
| 24492165.8026844 | -17.8529336402998 |
| 23099517.9649472 | -14.3027867639728 |
| 22193894.9032403 | -9.39368791842029 |
| 22429986.6053139 | -5.18775102813041 |
| 24091104.8425903 | -3.73115176070914 |
| 27257432.6761518 | -5.58295184898992 |
| 31890037.0954885 | -9.71202537147888 |
| 31997500.2733469 | -15.2150728823755 |
| 31997670.3619449 | -20.9749862892156 |
| 31997960.7382352 | -26.1993272491403 |
| 31998327.7510571 | -31.3994629569386 |
| 31998784.6697377 | -38.3475888674671 |
| 31999503.4582707 | -53.6006467744692 |
| 24934626.3769246 | -76.3169618514754 |
| 22540826.5470444 | -111.316184261966 |
| 27886984.097775 | -142.070549773776 |
| 32000000 | -158.734923640728 |
| 32000000 | -166.799257746166 |
| 32000000 | -170.135967763604 |
| 32000000 | -170.702081263629 |
| 32000000 | -167.643243382985 |
| 22751507.7544012 | -155.806122229269 |
| 15759603.8304244 | -133.559323085965 |
| 12820081.8727937 | -98.6838451435153 |
| 17294883.605147 | -47.8673042643138 |
| 25417404.961258 | -27.7710344852443 |
| 30498632.2012365 | -17.8916790001551 |
| 27765117.719457 | -11.6315713694731 |
| 25310710.2658984 | -3.08347119780311 |
| 24114115.3170127 | 6.27799343143285 |
| 24331789.6641062 | 12.8880003863145 |
| 25585193.9474424 | 14.4444207302042 |
| 27456233.2709074 | 11.2047433048776 |
| 29598634.3396341 | 4.92901510568243 |
| 31886239.5732093 | -2.52677910822513 |
| 32000000 | -9.88887083892731 |
| 32000000 | -16.9430470137154 |
| 24510726.0558635 | -42.3095590114395 |
| 21268275.0780393 | -133.587325033443 |
| 27977450.0148005 | -154.820355907206 |
| 30679182.9591766 | -166.533065344746 |
| 31196423.7139659 | -174.56864801355 |
| 31793454.5028301 | 179.051015679962 |
| 18723645.9126869 | 172.3455208484 |
| 3429330.2826906 | -8.1710445390554 |
| 15912453.6269167 | -25.0029194207833 |
| 17825678.22144 | -51.2814894472178 |
| 20394406.3853696 | -105.086252392973 |
| 31841611.4274177 | -142.365613537128 |
| 31494279.4178381 | -145.919242314829 |
| 31235940.2794158 | -146.732146228876 |
| 28732566.1539252 | -147.399886810864 |
| 18903693.7723975 | -144.580762779675 |
| 6649550.63456721 | -93.2246005964339 |
| 31999784.7648855 | -9.19579577618486 |
| 31999895.3867788 | -12.1152960154951 |
| 32000000 | -13.4753222464455 |
| 32000000 | -12.4062270258165 |
| 32000000 | -10.2951646768232 |
| 32000000 | -8.33445301264572 |
| 32000000 | -7.13420044234823 |
| 32000000 | -6.78614249673998 |
| 32000000 | -7.13782169175037 |
| 32000000 | -8.0183027934513 |
| 32000000 | -9.34034339167734 |
| 32000000 | -11.1317583156612 |
| 32000000 | -13.5673293746185 |
| 32000000 | -17.054308807669 |
| 32000000 | -22.3632795838436 |
| 24230924.7425455 | -46.632828029675 |
| 31907927.1132102 | -151.686513482862 |
| 31999383.0430013 | -161.080898299032 |

| | |
|---|---|
| 31999975.8874248 | -164.485992201579 |
| 32000000 | -166.000493075226 |
| 32000000 | -165.968760255881 |
| 32000000 | -164.081570959182 |
| 19347187.8824101 | -153.740141151362 |
| 7379208.29081556 | -99.4085173891792 |
| 12761981.7209873 | -29.2076346333218 |
| 20389575.2857476 | -14.9093937769584 |
| 26282824.8127898 | -9.27813187557942 |
| 30372107.8514319 | -5.990905935628 |
| 26654370.6929972 | -4.09623949257189 |
| 21498790.690009 | -1.090837281388 |
| 13274488.4854642 | 5.28773120561838 |
| 14761284.1912935 | 10.0955701355189 |
| 13631957.1826036 | 13.9925756820122 |
| 8690818.90114153 | 22.7944184653804 |
| 3582152.05100727 | 124.797190025224 |
| 15093836.4599395 | 171.748249623254 |
| 28020843.7443975 | 177.7835062713 |
| 32000000 | -179.749913736052 |
| 32000000 | -177.772634941426 |
| 32000000 | -175.651710055193 |
| 32000000 | -174.157800158606 |
| 32000000 | -173.6260347287 |
| 32000000 | -174.863618569666 |
| 15620348.1585964 | -176.843907637294 |
| 28891339.9545676 | 0.512123319328685 |
| 32000000 | -2.58713047020602 |
| 32000000 | -3.97483777744738 |
| 32000000 | -4.41128224117629 |
| 32000000 | -4.40375104766078 |
| 32000000 | -4.25804539327705 |
| 32000000 | -4.18405938839655 |
| 32000000 | -4.33630811698985 |
| 32000000 | -4.81568938673711 |
| 31082304.1543191 | -5.62883291046764 |
| 29912279.2377754 | -6.5895632739895 |
| 28711176.2476448 | -7.40694246012102 |
| 27553621.7082241 | -8.32715985226888 |
| 6054709.25037279 | -124.658735731719 |
| 29929682.9200143 | -171.70313174706 |
| 27234443.9164301 | -172.109638318007 |
| 3812804.27692383 | -74.0260616378095 |
| 16127952.4133596 | -15.2458246489901 |
| 31652264.5837479 | -9.31124663414687 |
| 32000000 | -8.82947882226689 |
| 32000000 | -9.43818530041747 |
| 32000000 | -10.5873131381545 |
| 31946074.3311905 | -11.8375589079865 |
| 31423634.224179 | -12.8303356321624 |
| 31001667.4315663 | -13.2804960254495 |
| 30459189.7684033 | -13.1599953545314 |
| 10584449.7649273 | -34.5439486487525 |
| 19853197.4325606 | -162.425048840483 |
| 27958888.6401879 | -165.82226857859 |
| 8193844.7054204 | -115.877185074573 |
| 26680601.511749 | -13.6171043066508 |
| 27602957.4166143 | -8.78100632333384 |
| 29584153.4447972 | -5.05956128222477 |
| 31893858.5800096 | -3.01437897180811 |
| 31999626.3874395 | -2.30433629582574 |
| 31999757.2838566 | -2.38669451313433 |
| 31999846.5517265 | -2.77248009676996 |
| 31999911.121278 | -3.15108403559639 |
| 31999942.5796258 | -3.45068036434467 |
| 30507037.0612448 | -175.343386569228 |
| 31999931.0808196 | -173.747397608852 |
| 32000000 | -174.105181980083 |
| 32000000 | -175.044249494877 |
| 32000000 | -175.884778467336 |
| 32000000 | -176.40030080629 |
| 32000000 | -176.474750490677 |
| 31999794.0949083 | -175.848820988907 |
| 31999225.3330521 | -173.951435870174 |
| 31998185.7535902 | -167.149533856544 |
| 26492500.817595 | -17.3894277412849 |

| | |
|---|---|
| 31013486.5416958 | -8.2699418569938 |
| 32000000 | -4.86079612121855 |
| 32000000 | -3.77253033119292 |
| 32000000 | -4.06632220364322 |
| 32000000 | -7.11241598101281 |
| 32000000 | -13.6358604679437 |
| 28218153.4556327 | -21.3525960548494 |
| 32000000 | -21.7246392610922 |
| 32000000 | -17.2321901249671 |
| 32000000 | -17.6652290204811 |
| 31999964.8555282 | -16.8874522461536 |
| 32000000 | -14.8297843137999 |
| 32000000 | -11.9757347697438 |
| 32000000 | -8.7293553131929 |
| 32000000 | -5.35682046521555 |
| 32000000 | -2.05639496729099 |
| 32000000 | 0.949491845580325 |
| 32000000 | 3.43612582198743 |
| 32000000 | 5.012644521944 |
| 30555476.0070766 | 5.3593937140893 |
| 29189620.2739576 | 4.33708105517366 |
| 22607376.6825037 | 2.84529329763632 |
| 12692348.6537048 | -0.918952955244852 |
| 6587597.5314747 | -10.5821319845033 |
| 3742155.50227469 | -153.628745175817 |
| 31998844.2427744 | -173.886070863226 |
| 31999083.1554883 | -170.144175902887 |
| 31349406.7587865 | -168.900898381602 |
| 30436836.5066987 | -169.91027325092 |
| 28099529.9948146 | -172.360210817329 |
| 21996884.5410341 | -175.555086395316 |
| 18787989.8613289 | 179.868969999481 |
| 13080013.059916 | 175.053399224677 |
| 14038676.6863235 | 9.78601305643068 |
| 30285262.4274133 | 8.36758236578499 |
| 26666321.6978481 | 13.0457186277745 |
| 25548504.3596171 | 14.9028474168995 |
| 26502715.1904064 | 14.0659224569092 |
| 25580021.5704453 | 13.1944305090621 |
| 28493585.5543701 | 10.1627311352695 |
| 32000000 | 7.47869125075599 |
| 31999709.2746917 | 5.65878051139225 |
| 31999289.6532153 | 4.85708521413431 |
| 31998868.1621275 | 4.39756036102639 |
| 30019889.7580606 | 4.3341592817984 |
| 27188184.2427514 | 4.83907187762003 |
| 24072885.9860861 | 6.09415620768304 |
| 21193382.8838768 | 8.15045968121768 |
| 10179179.6424697 | 25.862860731566 |
| 32000000 | 171.488765129884 |
| 32000000 | 173.864303892318 |
| 32000000 | 174.161932716014 |
| 32000000 | 173.88610559077 |
| 32000000 | 173.226701766593 |
| 32000000 | 171.723586640847 |
| 20829030.925042 | 159.161235827442 |
| 11313750.9776837 | 45.5005638858513 |
| 31629467.1887284 | 15.4081708249052 |
| 31998550.5660681 | 10.8233231164586 |
| 31999190.5825228 | 7.63499813855431 |
| 31999758.9966989 | 5.17736876640556 |
| 32000000 | 3.35852419007294 |
| 32000000 | 2.1898660475459 |
| 31999896.4173925 | 1.71448333418654 |
| 31999523.2841133 | 2.0034736689385 |
| 31999073.376558 | 3.18916695734014 |
| 31993235.8485203 | 5.26755467209016 |
| 27823151.2236764 | 10.2181680025319 |
| 16821953.4885419 | 21.8924936833361 |
| 11856310.6500188 | 39.154137879429 |
| 9503201.79713572 | 61.4458707094446 |
| 10762180.4038732 | 53.5804879196207 |
| 12783717.1348006 | 39.9850728646206 |
| 10089598.7785666 | 45.0201506703027 |
| 5839584.53492229 | 93.1799866507062 |
| 13162513.5894213 | 159.372754224814 |

| | |
|---|---|
| 20259848.5553505 | 169.444281820463 |
| 24994205.8417924 | 173.307005656729 |
| 31246243.1528849 | 175.845204034193 |
| 28651117.2554431 | 175.532624168961 |
| 2562360.74782347 | 49.7800111833115 |
| 8285786.06435535 | 9.99808774889642 |
| 16792150.5997305 | 4.39234650655819 |
| 30258259.174407 | 2.64601391442639 |
| 31477651.539381 | 2.52434576834783 |
| 31878456.5547913 | 2.15927454284529 |
| 31999748.7738183 | 1.52191443486828 |
| 32000000 | 0.700625749807758 |
| 32000000 | -0.294306319453602 |
| 32000000 | -1.5089955757389 |
| 32000000 | -3.02874990003327 |
| 32000000 | -4.94613249359475 |
| 32000000 | -7.51229680581079 |
| 32000000 | -11.412246510592 |
| 6745777.23872038 | -102.993497600125 |
| 24296306.8898055 | -167.928321304315 |
| 28710142.9218595 | -174.263164912487 |
| 28390748.5118811 | -178.430477072023 |
| 27410439.0487555 | 178.436580836205 |
| 25388973.4598995 | 174.810547112471 |
| 12234737.5210619 | 163.587403435629 |
| 6594446.44166556 | 39.0674034585993 |
| 24445425.5492654 | 10.558707965279 |
| 29771174.2839234 | 9.05436209633459 |
| 30061956.2284513 | 9.73639660353853 |
| 30149851.8595286 | 10.8203529709725 |
| 29597498.595171 | 11.974434926996 |
| 28714771.5787727 | 12.5127116542237 |
| 25868003.6490041 | 12.7761474208516 |
| 18785663.0199754 | 13.8276063570314 |
| 11111198.5065791 | 161.929716894521 |
| 31999828.0725867 | 174.288596271612 |
| 32000000 | 172.876221333706 |
| 32000000 | 173.025199978392 |
| 32000000 | 173.678471207513 |
| 32000000 | 174.369510471872 |
| 32000000 | 174.776585384059 |
| 31976678.2070018 | 174.639118239159 |
| 31839891.2826717 | 173.776615624083 |
| 31703065.0332244 | 172.157805626899 |
| 16395997.1636417 | 156.894720489649 |
| 26364900.7270761 | 14.986126965361 |
| 31713784.4315731 | 10.31910455759 |
| 31731080.2476575 | 8.8306184816447 |
| 31610230.6522739 | 7.44050248386883 |
| 31405278.6942926 | 6.07300999762847 |
| 31185986.3474862 | 4.64009239127225 |
| 31017566.469929 | 3.08971376392418 |
| 30959802.7342364 | 1.46282904566249 |
| 31061877.8293338 | -0.374940231581672 |
| 31315009.7727207 | -2.28251269542139 |
| 22444049.9798358 | -5.6132581143947 |
| 15920493.9069013 | -9.44679079077808 |
| 15368729.1721326 | -10.0282472491535 |
| 16005530.7357222 | -8.89224498212997 |
| 21410123.5742758 | -5.47548768669257 |
| 30581261.1082378 | -2.80922109410896 |
| 31997482.7365018 | -1.45034735181432 |
| 31997235.0180448 | 0.0419817268045984 |
| 31996783.362976 | 1.91496970758504 |
| 31862620.4645042 | 4.28141046604518 |
| 31749829.4741596 | 6.96837488752932 |
| 31701148.7600792 | 9.78959698458717 |
| 31673710.2184726 | 12.4724155514707 |
| 20360391.4669392 | 22.8749214890112 |
| 15067052.08186 | 34.1021739366864 |
| 9871502.34441054 | 60.0770007738456 |
| 9638444.0672649 | 117.937928382952 |
| 18618935.9776186 | 152.115664683892 |
| 30253222.6837727 | 161.924460649494 |
| 29339282.007007 | 159.881977064431 |
| 27598011.9599671 | 158.094412543808 |

| | |
|---|---|
| 26823080.7317138 | 157.797563776475 |
| 26882439.5742776 | 158.768408385661 |
| 28058937.4176769 | 161.020363878602 |
| 26437702.7059327 | 162.45560572015 |
| 24131463.2188853 | 162.33489347575 |
| 17825039.442585 | 19.7131885468972 |
| 26797991.8537946 | 9.48702291859215 |
| 31999742.9885786 | 4.36984585222307 |
| 31999765.7600675 | 0.910561649764946 |
| 31999823.6376928 | -1.39917520445491 |
| 31999896.0953743 | -3.00588693587619 |
| 31999965.1902464 | -3.96286417329605 |
| 32000000 | -4.30087767348702 |
| 32000000 | -4.08019864201649 |
| 32000000 | -3.34427954055567 |
| 32000000 | -2.058702822284 |
| 32000000 | -0.0361823399875018 |
| 32000000 | 3.17379390095874 |
| 32000000 | 8.32139556009934 |
| 31904771.3628261 | 15.5239258347054 |
| 31999688.3967582 | 162.607609076107 |
| 31999867.8885994 | 163.648154004561 |
| 31999954.7025925 | 164.862236587966 |
| 31999938.7262848 | 165.23434754225 |
| 31999814.875663 | 164.994462467325 |
| 31999600.7507046 | 164.367950011013 |
| 31999351.7700987 | 162.916792854335 |
| 20915926.4231882 | 64.1470331782827 |
| 29573537.7919939 | 33.9057425244854 |
| 32000000 | 23.1785966651143 |
| 32000000 | 16.2610340964095 |
| 32000000 | 11.0894002853046 |
| 32000000 | 7.3146803380468 |
| 32000000 | 4.7152847087293 |
| 32000000 | 3.08688163717685 |
| 32000000 | 2.21756019939449 |
| 32000000 | 1.88224865431765 |
| 32000000 | 1.9646031981841 |
| 30410582.6229922 | 2.73484609917257 |
| 28936525.1649801 | 4.0242905397303 |
| 28659904.7334466 | 5.1974729252573 |
| 29389595.5313026 | 5.93771868210694 |
| 31072412.839794 | 5.88000561956635 |
| 29838658.6017505 | 5.93964817871825 |
| 29852116.2109771 | 4.38152650766863 |
| 7268244.65030958 | 13.4678124075575 |
| 16582229.6540184 | 171.956621169503 |
| 12273728.5022209 | 164.08034379763 |
| 10728758.4080351 | 157.522647710772 |
| 12637143.3245544 | 156.982035716362 |
| 17662250.7537984 | 159.194460530284 |
| 13863160.4967726 | 32.1924901129961 |
| 29154371.5593085 | 15.2551751507959 |
| 28530529.336543 | 16.3843315378045 |
| 30162413.2281242 | 17.3528009035521 |
| 31999785.1984564 | 17.5377301780061 |
| 31999757.714915 | 16.9959100858761 |
| 31999675.7905124 | 15.4317311548291 |
| 31999498.7052383 | 12.0984543692147 |
| 31999176.1603902 | 6.27345670636641 |
| 960610.550039661 | 155.363117090989 |
| 19687576.6534355 | -176.308856984615 |
| 31355214.2662916 | -173.875440148447 |
| 32000000 | -170.507161962889 |
| 32000000 | -167.739880959837 |
| 32000000 | -166.542245864481 |
| 32000000 | -167.207230384459 |
| 31999863.6530128 | -170.627013968498 |
| 11327461.7616171 | -166.061910333809 |
| 30281706.1793952 | -4.67079636943676 |
| 32000000 | -3.64858259159638 |
| 32000000 | -4.44463862180298 |
| 32000000 | -5.39319197337118 |
| 32000000 | -6.65369716052647 |
| 32000000 | -8.37423440762908 |
| 32000000 | -10.6240786133068 |

| | |
|---|---|
| 32000000 | -13.4997578458472 |
| 32000000 | -17.1456531324466 |
| 32000000 | -21.7762661155 |
| 31863517.3447128 | -27.76410000343 |
| 31708390.7177173 | -36.8252651716575 |
| 31592838.2632886 | -52.0131346034226 |
| 27524395.4250541 | -66.7274169290496 |
| 23488786.6478962 | -79.9126749499588 |
| 20338483.5069939 | -88.4674771881896 |
| 17782133.1099273 | -74.0988369758182 |
| 19136157.2274085 | -44.5797232861626 |
| 26196064.764261 | -20.6016108979051 |
| 26997891.805722 | -9.60642771051634 |
| 27754392.5399744 | -0.993567539751838 |
| 28223262.645691 | 6.23688595143081 |
| 25884739.6024425 | 12.6211797894704 |
| 22299443.3269235 | 18.2073784933626 |
| 20151561.4039596 | 20.1747018921479 |
| 18657897.0597297 | 17.750452389409 |
| 16958715.1884321 | 11.3107445856305 |
| 18910245.3244301 | 0.699732797377462 |
| 23759424.1444965 | -7.5577437821729 |
| 16180891.6125175 | -23.3378644124275 |
| 9647604.97543384 | -84.4471018055796 |
| 22910696.7906672 | -146.679805127354 |
| 26102655.4428413 | -145.871482642427 |
| 28981152.5515052 | -148.246109120311 |
| 32000000 | -153.930417446668 |
| 32000000 | -159.20467073059 |
| 32000000 | -163.849265133127 |
| 32000000 | -167.955088055966 |
| 28213105.6982739 | -171.092494607266 |
| 14102646.7100414 | -172.934293540948 |
| 5602571.77407516 | 4.19237544098176 |
| 31998959.0536638 | -0.991308790253091 |
| 31999927.1185039 | -2.31104055597394 |
| 32000000 | -2.69579518011207 |
| 32000000 | -2.3409359545627 |
| 32000000 | -1.50916248811042 |
| 32000000 | -0.47916631583489 |
| 32000000 | 0.500639032905895 |
| 32000000 | 1.2237131600523 |
| 32000000 | 1.51088147102057 |
| 32000000 | 1.18516447695592 |
| 32000000 | 0.0493189383132673 |
| 32000000 | -2.11536827489392 |
| 32000000 | -5.49998691736603 |
| 31948272.0030167 | -10.1289767101126 |
| 31724729.2067818 | -15.7922139549787 |
| 24486316.4183026 | -26.4395371323798 |
| 9518485.32418901 | -100.46714335446 |
| 15279629.7573694 | -149.621343630129 |
| 16037876.5912222 | -156.589494923999 |
| 14803178.1579384 | -158.594221770578 |
| 8462468.49983287 | -145.32256438941 |
| 6958646.63303748 | -40.5958444830387 |
| 23037320.2188196 | -10.8863709564377 |
| 29234779.5167436 | -8.75393287941728 |
| 31021896.6551397 | -7.98850386964751 |
| 31836443.9429228 | -6.30325454661967 |
| 31916407.0283274 | -4.34183010948428 |
| 32000000 | -2.1366189397357 |
| 32000000 | 0.263801520593768 |
| 32000000 | 2.75787814499712 |
| 32000000 | 5.16855676250274 |
| 32000000 | 7.24729429026142 |
| 32000000 | 8.68996826729886 |
| 32000000 | 9.15468799480638 |
| 32000000 | 8.28269971091516 |
| 32000000 | 5.73821071448644 |
| 32000000 | 1.29445467305705 |
| 31996661.0028887 | -5.01182460052834 |
| 31930868.998031 | -12.6727704140532 |
| 31691395.58781 | -21.9620076718485 |
| 15377547.1823813 | -115.30464081335 |
| 31998777.304703 | -157.662275848541 |

| | |
|---|---|
| 31998920.3746775 | -160.879750474162 |
| 31999298.3058463 | -165.418266391261 |
| 31999816.4434928 | -170.461344256879 |
| 31985051.3679673 | -175.372388813176 |
| 24051532.8459189 | 178.329732367008 |
| 16666995.0349147 | 166.75148345604 |
| 28368575.9549808 | 12.6546692281074 |
| 31997036.7177778 | 9.49043576504303 |
| 31997382.846871 | 9.46049009699936 |
| 31997771.9089474 | 9.84255145966861 |
| 31998149.6978272 | 10.7672398450445 |
| 31998554.7606556 | 12.1431997958272 |
| 31998886.0933721 | 13.8309384223551 |
| 11730878.2283938 | 92.3244528903192 |
| 30975648.215806 | 155.574664883063 |
| 32000000 | 164.313898746935 |
| 31999862.9396274 | 170.645153236816 |
| 31999692.3129822 | 175.683272512051 |
| 31999568.5807425 | 179.702081027349 |
| 31999500.8388858 | -176.955570381802 |
| 31999503.0022039 | -174.278312205739 |
| 24815952.0062132 | -168.355394868661 |
| 11591336.0466063 | -41.2096293004537 |
| 31999909.9965794 | -14.0904493848273 |
| 31999857.0987314 | -10.7841633190144 |
| 31999811.8424831 | -8.36009505294878 |
| 31999802.4543968 | -6.95488690346093 |
| 31999874.7703602 | -6.31122068837209 |
| 32000000 | -6.30141688396914 |
| 32000000 | -6.88291601660575 |
| 32000000 | -8.02302426342117 |
| 32000000 | -9.6687657657858 |
| 32000000 | -11.7558628427334 |
| 32000000 | -14.2414346590404 |
| 32000000 | -17.1202812736263 |
| 32000000 | -20.3300983993599 |
| 31921299.8182978 | -23.45501316789 |
| 31564051.0472463 | -25.2758003409185 |
| 31172493.8053374 | -23.9032415263999 |
| 29571210.8164001 | -23.1422502873896 |
| 16192378.5361653 | -26.1155431849448 |
| 10383569.405831 | -21.5937427694641 |
| 10438761.4932066 | -7.04920174229305 |
| 14595530.3797308 | 3.44568808365826 |
| 20759528.1223762 | 8.16118378318932 |
| 27488326.56188 | 10.7736195598051 |
| 31998627.6344309 | 13.4643710929119 |
| 23288699.1234115 | 24.0499093760444 |
| 14705662.6316325 | 44.6485794968176 |
| 14085805.546001 | 50.885332286546 |
| 12412526.4613677 | 74.0426302903917 |
| 14399708.8868714 | 113.384742947987 |
| 23326832.9146555 | 141.392466163985 |
| 31735136.9852548 | 151.239697355031 |
| 29831747.0242129 | 146.770782385554 |
| 27431300.8123099 | 140.557435085293 |
| 26416734.2001436 | 136.055505915291 |
| 26198200.1975349 | 135.088054951391 |
| 25320036.0926202 | 136.248401689301 |
| 22958791.7907468 | 138.069203695852 |
| 13830980.5246541 | 90.1071301704919 |
| 31951062.0823022 | 25.3906667470557 |
| 31896964.3966068 | 30.0135828651572 |
| 31847803.7558439 | 28.4598940556982 |
| 31818202.068897 | 23.6711514146997 |
| 31844877.6749136 | 18.3778751714322 |
| 31938463.1805876 | 13.9114475747005 |
| 31999850.6962686 | 10.606603362638 |
| 31999990.6638284 | 8.50035465438918 |
| 32000000 | 7.63337042405902 |
| 32000000 | 8.13557958514342 |
| 32000000 | 10.2968527613569 |
| 32000000 | 14.6883837504446 |
| 31999448.5805279 | 22.3620331158335 |
| 31591916.1401612 | 34.9895645172227 |
| 27965108.0872792 | 56.3451305521601 |

| | |
|---|---|
| 26705391.257637 | 124.398554045246 |
| 32000000 | 163.601593348982 |
| 32000000 | 165.902476978575 |
| 32000000 | 165.96156453431 |
| 32000000 | 161.792693643585 |
| 24294305.9912094 | 119.958542416662 |
| 21362376.2506957 | 50.8380786984385 |
| 25408478.5068778 | 23.8931285667589 |
| 29954969.1521677 | 9.56163172791194 |
| 32000000 | 2.24952635647851 |
| 32000000 | -1.51271292197645 |
| 32000000 | -3.33343306627693 |
| 32000000 | -4.10392432335028 |
| 32000000 | -4.34762332559477 |
| 31998551.2154876 | -4.38634698287282 |
| 31209252.7519754 | -4.25371085518017 |
| 30681677.9305902 | -3.73591281522809 |
| 30380248.7208031 | -2.73138882383001 |
| 30234948.8854961 | -1.50895315263057 |
| 30100011.4339834 | -0.577381873063422 |
| 29846740.7637789 | -0.43812139151045 |
| 29419252.5954468 | -1.55397238966687 |
| 28851240.5556108 | -4.48794705293548 |
| 28274957.6550226 | -9.93852643454061 |
| 26131972.6050342 | -18.1310678874543 |
| 23199901.966293 | -28.7216685249434 |
| 21152670.8851241 | -142.105572730985 |
| 32000000 | -163.414543095552 |
| 32000000 | -168.455661603281 |
| 31919570.6649088 | -169.457017947319 |
| 31571070.8598199 | -168.6845602344 |
| 28531326.534709 | -166.339670658807 |
| 20407756.1782232 | -161.954584202489 |
| 31739534.2928036 | -15.7184293050755 |
| 32000000 | -16.8294644847727 |
| 32000000 | -21.338133265939 |
| 32000000 | -25.113531754972 |
| 32000000 | -29.7566365929495 |
| 31992092.0600485 | -36.6382695835347 |
| 31939577.0792605 | -47.3116744780882 |
| 25598036.6229135 | -75.1383413851447 |
| 32000000 | -149.768039052365 |
| 32000000 | -164.815174657271 |
| 32000000 | -168.334868117165 |
| 32000000 | -170.781466736349 |
| 32000000 | -172.379798624695 |
| 32000000 | -173.142959049232 |
| 32000000 | -172.899075604818 |
| 32000000 | -170.343191410776 |
| 22131768.6478043 | -139.803026794936 |
| 30282587.0563101 | -31.099813833621 |
| 31999920.1287784 | -19.1993214667128 |
| 32000000 | -14.9377591887374 |
| 32000000 | -13.2340947046547 |
| 32000000 | -12.3237478221987 |
| 32000000 | -11.4951425217941 |
| 32000000 | -10.4458307040427 |
| 32000000 | -9.09601046977683 |
| 32000000 | -7.56026100255037 |
| 32000000 | -6.06229227585823 |
| 31999887.3111638 | -4.4627502358449 |
| 29898329.3902433 | -1.6058730904481 |
| 25237011.991464 | 3.54897063514916 |
| 19993411.3685076 | 12.3873692208843 |
| 20722733.3501214 | 18.145292567683 |
| 16909615.0883039 | 26.878721813002 |
| 11327531.9138815 | 38.9275280942718 |
| 12011301.4984072 | 25.2189198399135 |
| 20491040.0252758 | 7.28771456095086 |
| 31597575.0354034 | 0.656976827763182 |
| 31652374.165241 | -3.69242771336814 |
| 31740528.9458507 | -6.62516174950053 |
| 31845100.2508441 | -8.90576952264965 |
| 31939102.2741328 | -9.86959024104444 |
| 31981526.4398985 | -8.64524730288719 |
| 31997717.5517753 | -4.48033487492863 |

| | |
|---|---|
| 32000000 | 3.15768730643044 |
| 28391159.6300654 | 18.967493340336 |
| 16270567.8765249 | 124.549600154806 |
| 29207628.3094197 | 154.9611302268 |
| 31119089.2269389 | 155.878194226693 |
| 31762163.2464116 | 154.888159734863 |
| 31984763.6292176 | 153.344779551399 |
| 31999705.2888651 | 152.26486710246 |
| 31999866.6388201 | 152.190544378961 |
| 31999814.685499 | 153.424349266208 |
| 31999543.8183302 | 156.335221204996 |
| 31999091.1571382 | 161.744357756712 |
| 31998582.0728261 | 171.632092217662 |
| 1138844.04447617 | -147.561621093042 |
| 31623005.2825014 | 2.11506809561048 |
| 31907555.4779533 | 6.38399317766634 |
| 31909200.5585841 | 6.60035299779 |
| 31911829.9741111 | 5.29222130994917 |
| 31907182.0184194 | 3.61071557241935 |
| 31892664.6771234 | 2.08042889847203 |
| 31864992.0138629 | 0.966510018494246 |
| 31816780.9532982 | 0.447400035927744 |
| 31764843.3370092 | 0.696199223971822 |
| 31722796.3298918 | 1.90942137324205 |
| 31704820.1655337 | 4.29030926333613 |
| 31709573.1724346 | 7.97683078141438 |
| 31527103.8749744 | 12.8983691144029 |
| 31572938.7862608 | 18.5783979789711 |
| 31893002.0594891 | 25.8166282142475 |
| 28598752.7761425 | 33.8503610627193 |
| 27488667.2818657 | 36.0282066948094 |
| 28884286.2492374 | 35.3135665942994 |
| 30421529.6346548 | 35.3504100337555 |
| 30454138.3500648 | 37.4462433571763 |
| 28243610.4339344 | 41.8788133471044 |
| 23847263.1710438 | 49.1685136795204 |
| 19510933.0814409 | 55.1876755269119 |
| 16033257.3001184 | 52.91583857466 |
| 8752249.58448096 | 74.658141466416 |
| 9995300.11863008 | 20.7563577061626 |
| 27586117.4996007 | -1.88971426533728 |
| 30289207.2433608 | -0.938671653600731 |
| 31614534.2950229 | 0.55203473129548 |
| 31998921.5327008 | 1.12858807514701 |
| 31999323.5629289 | 1.195130721533 |
| 31999737.111943 | 0.88500747512081 |
| 32000000 | 0.403448032055098 |
| 32000000 | -0.0997073646735038 |
| 32000000 | -0.524625750004976 |
| 32000000 | -0.803492374940021 |
| 32000000 | -0.871158048624018 |
| 32000000 | -0.417279403471254 |
| 32000000 | 2.35387307348223 |
| 18691352.491426 | 20.056119218346 |
| 30364692.9175786 | 166.331666260705 |
| 30986775.6113968 | 165.91030748793 |
| 30749127.8738679 | 163.930181301877 |
| 28911718.1388991 | 160.026178797085 |
| 25483133.9746468 | 153.293674080514 |
| 13431048.0678062 | 125.085212429739 |
| 9855474.55983999 | 87.2751574673752 |
| 21901769.3798874 | 23.7381125614561 |
| 31999803.4723629 | 13.1475337970976 |
| 31999771.9508339 | 16.7301802669398 |
| 31975863.796259 | 19.6964958832985 |
| 12304131.4904471 | 39.221457604581 |
| 31046878.8441865 | 179.131889576891 |
| 31856160.8463329 | -166.25485284321 |
| 31975721.9415639 | -158.63698426458 |
| 31996545.6164383 | -155.945321981123 |
| 31996940.9361649 | -155.769254153626 |
| 31970239.4509945 | -156.889353009917 |
| 31926690.1793201 | -158.894718509542 |
| 31880197.8348799 | -161.767173866942 |
| 31797467.2113403 | -165.647687397154 |
| 31657527.3703474 | -166.08639762789 |

| | |
|---|---|
| 8175097.29307962 | -36.8948597637906 |
| 32000000 | 0.959254134725217 |
| 32000000 | 4.61092027010005 |
| 32000000 | 4.82101729879268 |
| 32000000 | 4.75057188494262 |
| 32000000 | 5.02947773775524 |
| 32000000 | 5.71526100620627 |
| 32000000 | 6.78150745081821 |
| 32000000 | 8.19703097604981 |
| 31999971.8200092 | 9.91700628207801 |
| 31999916.3996158 | 11.8345209643644 |
| 31999890.0440389 | 13.6840311651459 |
| 31999892.9470503 | 14.9424805641514 |
| 31303690.2461733 | 14.8229241950474 |
| 29778073.5242284 | 12.4154899354121 |
| 24875972.6025403 | 10.4821760434038 |
| 23966553.2005427 | 6.08354543010462 |
| 29240943.3216569 | 0.908989196668666 |
| 30917736.3344859 | -3.18290764039221 |
| 31718155.756368 | -6.07645127145022 |
| 32000000 | -7.77056342696761 |
| 32000000 | -8.00893164895749 |
| 32000000 | -6.94796991997509 |
| 32000000 | -4.9658242282176 |
| 32000000 | -2.67964170721343 |
| 32000000 | -0.904850254915408 |
| 26714363.0427096 | -0.421018904377888 |
| 15293252.6094518 | -1.46238000348478 |
| 7416242.44599973 | -7.59419342704088 |
| 7556029.88839691 | -164.580825817431 |
| 32000000 | -177.23158048243 |
| 32000000 | -176.681570387982 |
| 32000000 | -175.16327649017 |
| 32000000 | -173.200404070751 |
| 32000000 | -171.320943248739 |
| 32000000 | -169.999055108799 |
| 32000000 | -169.615603338663 |
| 32000000 | -170.596670749948 |
| 32000000 | -173.737673661966 |
| 32000000 | 179.470406529598 |
| 8240783.73178725 | 79.0840133309014 |
| 28731076.2825042 | 25.0205710604087 |
| 32000000 | 14.9604005730441 |
| 32000000 | 11.7591971534799 |
| 32000000 | 10.385495966461 |
| 32000000 | 9.44630695588791 |
| 32000000 | 8.35262828396957 |
| 32000000 | 6.80952768497888 |
| 32000000 | 4.63197803977664 |
| 32000000 | 1.62482189550773 |
| 32000000 | -2.55795766241234 |
| 32000000 | -8.63514148645568 |
| 32000000 | -17.5144856335504 |
| 24030719.0316338 | -36.6578235329384 |
| 16107719.4640774 | -65.377473661952 |
| 12875448.7888784 | -70.110101336672 |
| 20193843.3622446 | -23.0913426761237 |
| 32000000 | -4.93088957398383 |
| 32000000 | 1.72082300113645 |
| 32000000 | 6.13850513849044 |
| 32000000 | 9.00423924556197 |
| 32000000 | 10.0728183755916 |
| 32000000 | 8.92326729457244 |
| 31948820.6131683 | 4.94973470348659 |
| 30740190.9749755 | -2.50767689517583 |
| 29338086.2550696 | -13.8489967021288 |
| 26249298.2397909 | -28.309163274709 |
| 22730738.6365357 | -46.0404072754968 |
| 23731596.3350621 | -50.9983465788566 |
| 32000000 | -34.0152743167971 |
| 32000000 | -23.0625628480702 |
| 32000000 | -17.453821685167 |
| 32000000 | -13.1010493447484 |
| 32000000 | -9.6374646685178 |
| 32000000 | -6.93384925453963 |
| 32000000 | -5.04124954919296 |

| | |
|---|---|
| 32000000 | -4.1599727088539 |
| 32000000 | -4.65261740915251 |
| 32000000 | -6.93032231030564 |
| 30965013.1202268 | -10.8508295559277 |
| 22713578.0935823 | -19.2172852545798 |
| 31998680.8880268 | -169.405506666889 |
| 31999178.4424725 | -171.015567514099 |
| 31999553.8223887 | -172.380995420058 |
| 31999652.2806822 | -174.021067480422 |
| 31999563.7041144 | -175.548222240677 |
| 14922559.9102948 | -172.999039685471 |
| 28199619.2083411 | -0.235001288779936 |
| 32000000 | 3.5417121094163 |
| 32000000 | 3.81738726606942 |
| 32000000 | 2.68101356788336 |
| 32000000 | 0.847877392375745 |
| 32000000 | -1.42843227262488 |
| 32000000 | -4.17408150776048 |
| 32000000 | -7.53023448346179 |
| 32000000 | -11.5136517418085 |
| 32000000 | -16.5498469331956 |
| 18986642.6107719 | -57.8937822732259 |
| 21357415.5656703 | -136.639122839471 |
| 28439298.2729815 | -156.268782420282 |
| 29666037.9396842 | -165.652213152073 |
| 30689348.0487221 | -172.896848081381 |
| 31765027.1844866 | -178.448756538718 |
| 31998095.7088147 | 179.895520166154 |
| 26383966.6037555 | 175.584541015787 |
| 11071808.8871018 | 164.585367405698 |
| 3135662.43046726 | 106.146952718034 |
| 12006548.6812492 | 11.7794175371036 |
| 23114502.6030504 | 3.21735078433282 |
| 24564000.3251355 | 0.716133427650086 |
| 26483298.3791079 | -0.909080633977554 |
| 28566202.1540949 | -1.55277355589006 |
| 30661072.9897625 | -1.34717049885944 |
| 31900050.1993246 | -0.528062710044382 |
| 31928761.9680004 | 0.735152890351284 |
| 31941086.2765452 | 2.35224711062861 |
| 26768146.1118484 | 4.79187407641902 |
| 17707088.9515852 | 9.5428703485531 |
| 12526114.2375912 | 16.0017351415798 |
| 12691837.6069378 | 15.8904845976352 |
| 16510742.7772633 | 9.62919550554914 |
| 15740720.1107082 | 5.67431321088947 |
| 26270485.4562897 | -0.377671811264437 |
| 32000000 | -5.91569239790962 |
| 32000000 | -9.94451840251758 |
| 32000000 | -11.7172743312567 |
| 32000000 | -12.0057097537272 |
| 32000000 | -11.2366409712627 |
| 32000000 | -9.66157983343399 |
| 32000000 | -7.33767502620867 |
| 32000000 | -4.14866606964541 |
| 32000000 | 0.187504356843989 |
| 32000000 | 6.01918727963665 |
| 22315705.0031518 | 22.5585362746161 |
| 31999944.8241921 | 159.193859886652 |
| 32000000 | 160.365246759985 |
| 32000000 | 161.07312929491 |
| 32000000 | 161.953291177798 |
| 32000000 | 162.733782849847 |
| 32000000 | 163.421973374452 |
| 32000000 | 164.312056926783 |
| 31999998.9305946 | 166.234499070733 |
| 31074729.6498945 | 170.785653946485 |
| 19277895.0878059 | -177.125770398025 |
| 18017599.3555234 | -22.4453623854226 |
| 32000000 | -9.37733605549776 |
| 32000000 | -9.73029481721563 |
| 32000000 | -10.7584689618648 |
| 32000000 | -12.2984109116081 |
| 32000000 | -14.2177375825786 |
| 32000000 | -16.2937054934121 |
| 32000000 | -18.0897490035145 |

| | |
|---|---|
| 31973360.385663 | -18.768334390711 |
| 30791130.8992146 | -17.0344512530198 |
| 23966939.1396888 | -12.6744270126158 |
| 10389631.0246364 | -5.4095833760133 |
| 2065671.73771601 | 113.868747214038 |
| 16567219.9845149 | 173.658653328712 |
| 23861674.5617199 | -175.997409069065 |
| 14366030.7047363 | -153.962061096685 |
| 18980767.2970253 | -26.2275177667806 |
| 24242459.1760776 | -15.2841400657609 |
| 27555863.0649158 | -11.3974617917525 |
| 31045644.4613244 | -9.66583143242403 |
| 31997752.1989284 | -8.99961656993467 |
| 31997994.8087071 | -8.58111703366241 |
| 31998248.4726833 | -7.62770394049995 |
| 31998472.7134035 | -4.997173746172 |
| 31998631.4856335 | 0.855209078930606 |
| 30960119.6626119 | 11.6762201302627 |
| 22175754.6197125 | 32.8511519712879 |
| 16695693.9873265 | 72.1927176857762 |
| 20086917.3802985 | 117.29356036678 |
| 20662522.3418168 | 117.720303992046 |
| 25044733.67575 | 53.542371421674 |
| 30748617.4195685 | 35.8392908605999 |
| 31611758.2390295 | 29.5809193300719 |
| 31998214.9017102 | 21.9427342358458 |
| 31998816.3665992 | 14.5937771491214 |
| 31999485.7865554 | 8.37578861312991 |
| 32000000 | 3.80796113483318 |
| 32000000 | 1.37861657369426 |
| 32000000 | 1.78761503677628 |
| 32000000 | 6.15509458984034 |
| 32000000 | 15.9213460702635 |
| 32000000 | 31.5781135405404 |
| 30717325.3248621 | 53.3133892659247 |
| 31997577.1125745 | 140.789542172542 |
| 31997132.5044517 | 143.435247659442 |
| 31996654.5137956 | 143.63792659756 |
| 31996282.9592234 | 144.451307095466 |
| 31996124.5394523 | 146.36093600399 |
| 30115372.4636835 | 121.899499073147 |
| 30066349.7296389 | 42.9016452516917 |
| 30819345.279388 | 30.476577502284 |
| 31335393.2749534 | 21.0284622758067 |
| 31693824.5208753 | 13.9215891513841 |
| 31844785.7476958 | 7.89083477469335 |
| 31793930.1916873 | 1.64674071368866 |
| 26408678.8932007 | -171.041159292362 |
| 31146684.376623 | -164.600222269005 |
| 32000000 | -160.754796371394 |
| 32000000 | -159.102336217442 |
| 32000000 | -159.710857712448 |
| 32000000 | -162.665889901736 |
| 32000000 | -168.199499682909 |
| 21714911.1991923 | -176.034791439448 |
| 10901122.0724572 | 12.3722664069035 |
| 14638092.2778527 | 22.3920268981048 |
| 18882193.0317904 | 26.4960690751596 |
| 22503547.5758899 | 27.1199449477779 |
| 25270150.7115789 | 24.6630734557077 |
| 27834576.7154057 | 18.7499833134044 |
| 31623611.1928516 | 9.79352646458875 |
| 12863321.5763344 | 6.52448397516749 |
| 980502.064965705 | -58.2180775857141 |
| 2391789.86445199 | -127.350697316466 |
| 6479629.62146933 | -23.5421723844135 |
| 22727952.762136 | -9.40137097527401 |
| 29713813.7823765 | -9.42326582512242 |
| 31788703.1688668 | -8.51766555704474 |
| 31695584.9588006 | -6.1737804429171 |
| 31616748.2468655 | -1.30226717007414 |
| 31042966.8940501 | 5.18765251971134 |
| 30138578.9784763 | 12.0104349316974 |
| 29223370.5205894 | 17.8186919016895 |
| 28221146.4674628 | 21.532266192167 |
| 27190395.7141698 | 22.3607057232578 |

| | |
|---|---|
| 26395425.2528756 | 19.8379346173959 |
| 26259784.3002568 | 14.1392874291644 |
| 27067475.3412725 | 6.40220672077898 |
| 28613343.5766071 | -1.73985118968849 |
| 30306533.4244347 | -9.12918158217844 |
| 31413370.0669713 | -15.4147080510125 |
| 31719408.2876264 | -20.661016121995 |
| 31894907.581129 | -25.2532069744865 |
| 31959872.1375404 | -30.1376491947347 |
| 31990183.3721878 | -36.8857548644913 |
| 31983297.768847 | -49.9931253671589 |
| 30659010.8716048 | -123.915028117303 |
| 29394204.2807345 | -141.602477907079 |
| 29731274.1593158 | -155.467180561749 |
| 30789875.7260553 | -164.505717263237 |
| 31669614.0324144 | -169.122172310267 |
| 31808218.3118156 | -170.152658180903 |
| 31940682.4748622 | -168.286109937642 |
| 32000000 | -163.861628262956 |
| 32000000 | -156.73472431024 |
| 29784681.2397664 | -59.6850048776601 |
| 31997404.0952152 | -52.6261941636485 |
| 31997189.4459202 | -49.177428049299 |
| 31997288.2159674 | -44.0760176781563 |
| 31997802.7882204 | -37.746383515692 |
| 31998649.3894945 | -30.8267202937343 |
| 31999518.5476177 | -24.0916260572626 |
| 32000000 | -18.367120026795 |
| 32000000 | -14.1024001028885 |
| 32000000 | -11.0197224013556 |
| 32000000 | -7.95682025148163 |
| 30435173.9827972 | -5.26825407506056 |
| 1808109.50489814 | -8.34265469926543 |
| 15391515.1691006 | 178.380697446561 |
| 24519873.5676194 | 179.494359261027 |
| 25583614.9388035 | -179.19726868512 |
| 18282088.90154 | -177.200183383664 |
| 1934865.87761732 | -147.556092841745 |
| 6939933.06214828 | -7.30859008025758 |
| 9325706.16475064 | -9.14922845632103 |
| 14912686.6043715 | -13.510064503465 |
| 23015787.3789256 | -16.9447544537985 |
| 27601432.6549075 | -20.0073430379804 |
| 27128424.7414273 | -25.7050405504958 |
| 26981721.0990491 | -30.1100158151505 |
| 26842278.4667791 | -30.4243898410654 |
| 26598315.6952323 | -25.2753972493948 |
| 26806260.2266577 | -14.4625285108783 |
| 28388506.5495065 | -0.270272952864911 |
| 30702993.2670485 | 12.9102943309542 |
| 32000000 | 22.2356217623896 |
| 32000000 | 27.0667317332014 |
| 32000000 | 28.1901469611038 |
| 32000000 | 26.4176831196237 |
| 32000000 | 22.1388279779761 |
| 31999887.8846203 | 15.4092431626829 |
| 31999502.0499054 | 6.25392556840784 |
| 31999209.5940483 | -4.80130585645844 |
| 31999088.8130406 | -16.2162712607232 |
| 31693595.6272612 | -25.5237793077744 |
| 28218279.5898254 | -32.0483996501072 |
| 17347737.1295162 | -51.7691021238026 |
| 13141367.8574885 | -120.341993505466 |
| 31999879.3490822 | -164.620477478409 |
| 31999411.8830195 | -169.345728673416 |
| 31998738.3418971 | -171.817672483056 |
| 31388429.7233417 | -174.332123371909 |
| 29252040.4049366 | -175.406226932381 |
| 27938918.2954482 | -174.209908494841 |
| 27696578.768656 | -170.434446487017 |
| 27423967.7510944 | -164.387637180116 |
| 23178440.7280773 | -154.330385349256 |
| 13692369.1569608 | -124.089912463952 |
| 11134248.5075356 | -82.6173891462061 |
| 11692930.4330819 | -52.1579723726999 |
| 11816396.9957816 | -31.2891147650618 |

| | |
|---|---|
| 10772794.6231923 | -11.5635044311781 |
| 9283429.13006528 | 13.5566799190136 |
| 11920651.5676202 | 33.1024230719298 |
| 17875880.2632113 | 36.7848091175759 |
| 26599899.785731 | 33.5626600973286 |
| 31999595.614975 | 23.1659183932591 |
| 31999918.4683862 | 25.6817761560145 |
| 32000000 | 25.0713860011614 |
| 32000000 | 23.2924401514333 |
| 32000000 | 20.7875778360146 |
| 32000000 | 17.8772294950401 |
| 32000000 | 14.755601179981 |
| 32000000 | 11.4970577457845 |
| 32000000 | 8.03543566980469 |
| 31999719.732981 | 4.05957889261614 |
| 28334889.0234386 | -1.27879483731147 |
| 23319164.3547104 | -9.97321733216132 |
| 20112266.6356397 | -23.4207608628818 |
| 18973550.611378 | -37.8502353701739 |
| 14091475.8489875 | -122.110321486335 |
| 21549933.2681809 | -151.874735030293 |
| 20674567.9108486 | -156.752022065295 |
| 16797192.1411148 | -158.168664917748 |
| 9923026.80340377 | -152.686576878607 |
| 3559592.53643193 | -117.49492135546 |
| 5934950.25101311 | -21.213407904002 |
| 15924272.3414786 | -6.62785826560448 |
| 31920171.1795124 | -4.78714013595211 |
| 31999963.8000138 | -5.13739054476595 |
| 32000000 | -6.70940581446736 |
| 32000000 | -8.38064951855529 |
| 32000000 | -10.1079915345021 |
| 32000000 | -11.7785753841657 |
| 32000000 | -13.16437665981 |
| 32000000 | -13.9892661985081 |
| 32000000 | -14.0003719395231 |
| 32000000 | -12.9991222389938 |
| 32000000 | -10.8174762605832 |
| 32000000 | -7.17785557530077 |
| 32000000 | -1.12946173389329 |
| 10239007.8793115 | 120.845812893223 |
| 28765954.2394162 | 159.702829763093 |
| 31770477.5159258 | 162.475756044028 |
| 31999129.4253391 | 165.015188525694 |
| 31998873.7988427 | 168.372439579617 |
| 31998476.6577897 | 172.197247746475 |
| 31998081.3523926 | 176.039312439653 |
| 31997801.2988439 | 179.474184386072 |
| 31997640.2881927 | -177.969203030342 |
| 31997493.4233897 | -177.476338670393 |
| 22887883.8766743 | 162.943834398312 |
| 25299247.9183666 | 24.9696569492101 |
| 32000000 | 10.6617799777564 |
| 32000000 | 9.82449251330438 |
| 32000000 | 11.167739051963 |
| 32000000 | 12.4003749493829 |
| 32000000 | 12.7910151537865 |
| 32000000 | 12.1918162948325 |
| 32000000 | 10.6839394256173 |
| 31927902.6338907 | 8.45760366659842 |
| 31792968.3628954 | 5.7691003762829 |
| 31703625.142319 | 2.94262628166483 |
| 31667906.7833687 | 0.431059578913565 |
| 31063621.5728489 | -1.16565901007182 |
| 28087946.2960008 | 0.626326491332365 |
| 6396448.46318823 | 6.49985040471514 |
| 4156590.97788274 | 36.9353870985135 |
| 11566641.897433 | 27.4405479434236 |
| 20349991.3634313 | 25.0934758460189 |
| 29124947.0675208 | 23.4254916085419 |
| 30256519.5558243 | 25.6298386966297 |
| 24291274.3377704 | 31.8427787851583 |
| 10810998.4699169 | 78.0751934576051 |
| 27516491.0319693 | 164.9279770072 |
| 32000000 | 177.383203419537 |
| 31999899.0277639 | -176.418888024741 |

| | |
|---|---|
| 31999658.4678789 | -172.083694969981 |
| 31999380.9480768 | -169.808329253621 |
| 31999161.813533 | -169.571286300384 |
| 31998841.4848684 | -172.383831340009 |
| 14940727.6564017 | -173.309440738522 |
| 25964720.2072985 | 2.44260187682384 |
| 32000000 | 4.05388339864995 |
| 32000000 | 5.43941254714251 |
| 32000000 | 6.45323550359274 |
| 32000000 | 7.34157874177808 |
| 32000000 | 8.07052405152357 |
| 32000000 | 8.40968734111078 |
| 32000000 | 7.95222687006086 |
| 32000000 | 6.11557501539324 |
| 32000000 | 2.34780666597844 |
| 32000000 | -3.79668551251832 |
| 8346346.2078439 | -39.3463696771413 |
| 11332512.7174084 | -178.631892368084 |
| 12004038.5331396 | 146.287597998586 |
| 18808766.5895422 | 41.3040015463339 |
| 31933420.3598161 | 13.2641426650797 |
| 31995887.1355588 | 9.41357176854306 |
| 31675144.3889767 | 7.91150784186708 |
| 31092961.2097376 | 7.13075253080333 |
| 30140033.2475346 | 4.86358587957258 |
| 15647262.3174598 | -5.51405659883138 |
| 31998062.804972 | 176.579415283449 |
| 31998211.6600146 | 170.644309531219 |
| 31998633.0325821 | 168.646651207189 |
| 31999205.1536654 | 168.580011319397 |
| 31999828.5228529 | 169.943638302943 |
| 32000000 | 172.767570755669 |
| 32000000 | 177.578971002458 |
| 32000000 | -174.11331169619 |
| 32000000 | -157.736356805372 |
| 31822193.5191241 | -31.5891686773252 |
| 31999025.0087972 | -22.318296675632 |
| 31999624.5874157 | -20.4079135022862 |
| 32000000 | -18.3503512008653 |
| 32000000 | -16.5353000855367 |
| 32000000 | -15.0846603393577 |
| 32000000 | -14.0193474123582 |
| 32000000 | -13.3233139674878 |
| 32000000 | -12.9637740717521 |
| 32000000 | -12.8993684415392 |
| 32000000 | -13.0920719019782 |
| 32000000 | -13.5233414496582 |
| 32000000 | -14.1869277598829 |
| 32000000 | -14.9948031546214 |
| 32000000 | -15.6506164759069 |
| 32000000 | -15.7477679401563 |
| 15289766.8605508 | -15.4441962183252 |
| 1851475.41573286 | 164.168317777117 |
| 4452102.42150904 | 103.955221753983 |
| 12857841.8081136 | 39.3465950946401 |
| 26970697.1361064 | 26.3023409803317 |
| 32000000 | 16.1277713733098 |
| 32000000 | 10.7637629445826 |
| 32000000 | 7.84135012385241 |
| 32000000 | 6.0689602005626 |
| 32000000 | 5.12686521230167 |
| 32000000 | 4.98827747462798 |
| 32000000 | 5.9030117920089 |
| 31999663.5089363 | 8.62348365762599 |
| 31999203.9471336 | 15.676141407191 |
| 31999570.324677 | 36.306816282369 |
| 29571859.4372951 | 130.56062233411 |
| 32000000 | 164.562095549551 |
| 32000000 | 166.224145364466 |
| 32000000 | 167.152730240388 |
| 32000000 | 167.540615463223 |
| 32000000 | 167.255857714731 |
| 32000000 | 165.028440224653 |
| 24676702.6778683 | 116.617762326553 |
| 29775458.2774496 | 28.7515226159578 |
| 32000000 | 9.47658019200599 |

| | |
|---|---|
| 32000000 | 1.63227422850331 |
| 32000000 | -1.97332904741914 |
| 32000000 | -4.05897129036558 |
| 32000000 | -5.63877203232781 |
| 32000000 | -7.18004054252737 |
| 32000000 | -9.01126367007176 |
| 32000000 | -11.4060711245893 |
| 31923656.6700652 | -14.3810469240821 |
| 31788961.3380553 | -17.2718295781376 |
| 26436101.0530687 | -19.2783187485218 |
| 17079858.9199621 | -23.310550505229 |
| 5327291.52746962 | -69.0793057244046 |
| 7973398.74588603 | -148.28081356721 |
| 12264570.8111325 | -17.5009391480771 |
| 32000000 | -2.99701111027834 |
| 32000000 | 1.00257670142911 |
| 32000000 | 3.91438809469333 |
| 32000000 | 6.31697241526837 |
| 32000000 | 8.34143162254529 |
| 32000000 | 10.1341564429007 |
| 32000000 | 11.9006864361959 |
| 32000000 | 13.9047185116874 |
| 32000000 | 16.4364262949492 |
| 32000000 | 19.6886476723289 |
| 32000000 | 23.479543132986 |
| 32000000 | 27.8306653812127 |
| 21096373.8684406 | 53.5849085841001 |
| 24395887.1097921 | 136.75497124607 |
| 18741887.410622 | 107.264646268141 |
| 31811698.6093734 | 24.7308189964879 |
| 31984097.5873599 | 17.6190634772948 |
| 32000000 | 14.4156083683236 |
| 32000000 | 13.6684265065045 |
| 32000000 | 13.8301924854575 |
| 32000000 | 14.0400047591507 |
| 32000000 | 13.9499717697044 |
| 32000000 | 13.4198944445973 |
| 32000000 | 12.3517966261358 |
| 32000000 | 10.6041074262135 |
| 32000000 | 7.91680216289068 |
| 32000000 | 3.79674434832595 |
| 32000000 | -2.24016754575623 |
| 7579491.97195528 | -40.3929636434212 |
| 11584385.147979 | -162.562456642819 |
| 17274963.3829978 | -176.624559172379 |
| 20394292.8486311 | 175.009238972192 |
| 22538546.5044722 | 167.668042504676 |
| 25316162.7348226 | 161.363939645422 |
| 23829266.5034638 | 152.090598067716 |
| 11787116.5324028 | 85.1092701562044 |
| 18501825.9210239 | 29.0952361363182 |
| 18775980.4802037 | 14.3062496384342 |
| 15208418.6473109 | 1.64971998396185 |
| 11175953.4398155 | -14.8828831882361 |
| 7087270.15077021 | -144.393907871479 |
| 29338296.5865951 | -176.491887706365 |
| 29377462.2880071 | 176.847694708953 |
| 29683842.0501217 | 172.731768928595 |
| 30468590.858773 | 171.369963165698 |
| 31345303.048372 | 171.418209807797 |
| 31999125.0103147 | 171.784144227906 |
| 32000000 | 171.859701930106 |
| 32000000 | 171.421092761855 |
| 32000000 | 170.476617948725 |
| 23774643.3366468 | 168.067522421609 |
| 10190709.057324 | 13.7432501429162 |
| 31925213.4580072 | -1.35102565538971 |
| 31999282.7557152 | -4.02700434637045 |
| 31999705.5696464 | -5.96542623595775 |
| 31999966.0258595 | -6.97727908758533 |
| 32000000 | -7.38721968290891 |
| 31999933.0453476 | -7.29423294126689 |
| 31999719.2026692 | -6.53949020245405 |
| 29714450.91917 | -5.9301607945374 |
| 10968668.4850368 | -2.89681582406356 |
| 3144586.93643408 | 128.979916324559 |

| | |
|---|---|
| 9225298.35599547 | 143.550638409718 |
| 9106695.77283475 | 117.357149313484 |
| 10901836.1286371 | 65.3420334758263 |
| 17902060.5312678 | 37.5840496714036 |
| 27628035.9759186 | 23.7768386676903 |
| 31983770.3451123 | 17.3632139923769 |
| 32000000 | 13.1055096610473 |
| 32000000 | 9.81656707576378 |
| 32000000 | 7.44477276303485 |
| 32000000 | 5.89119555276323 |
| 32000000 | 5.02915899089278 |
| 32000000 | 4.69201447054616 |
| 32000000 | 4.66940787821226 |
| 32000000 | 4.70673585418246 |
| 32000000 | 4.49236978914645 |
| 32000000 | 3.62098884590519 |
| 32000000 | 1.52911000073305 |
| 32000000 | -2.57893024278571 |
| 31808098.547988 | -9.74722949547116 |
| 26496327.972913 | -21.1439847934037 |
| 16756139.8200273 | -44.690154921268 |
| 13080562.7706648 | -79.911291338009 |
| 27780238.0637013 | -153.927254107086 |
| 31998829.8900628 | -168.786730534188 |
| 31998995.7574805 | -173.256611785696 |
| 31999085.5023791 | -173.10470770548 |
| 21551662.4304258 | -165.761257734869 |
| 8225991.80603351 | -70.4651646692002 |
| 23772426.7089006 | -30.702663629481 |
| 28617395.0533456 | -34.8917625994173 |
| 30570948.6692386 | -39.3615361319419 |
| 31371355.0961547 | -42.2777481102789 |
| 31195318.2530195 | -43.706497030211 |
| 29299382.3211307 | -44.089453627168 |
| 27123584.7405573 | -41.795699411638 |
| 27891551.5918581 | -32.607276403168 |
| 28847939.7455896 | -22.914596284128 |
| 28979163.4903853 | -15.4389220594314 |
| 29730874.5497741 | -9.9158265054852 |
| 30922692.6188309 | -6.13298852083771 |
| 31694335.6115148 | -3.49475965719545 |
| 31999041.7655206 | -1.35201539867077 |
| 31998811.2434859 | 0.797165382624007 |
| 31998483.0569655 | 3.40336456579078 |
| 31998129.7136018 | 6.81338496335158 |
| 31997837.6965784 | 12.0669635359137 |
| 18522278.5406355 | 38.4166493274303 |
| 14795601.3061981 | 137.564079590316 |
| 25631681.9113405 | 164.172666022121 |
| 24300787.71795 | 170.759959739305 |
| 14551721.96564 | 171.992907691708 |
| 2053191.25979647 | 74.6427779880174 |
| 12435975.5551491 | 15.5728876693352 |
| 16844969.6456273 | 17.1611761261622 |
| 23148236.4205189 | 15.9888809652746 |
| 28531320.285816 | 14.4309657985463 |
| 29831102.858748 | 13.4844032139286 |
| 31102688.725776 | 13.0310564991436 |
| 28565843.4112984 | 16.9342924014122 |
| 25421187.6093951 | 19.2967612578124 |
| 27837709.4626609 | 18.8491326617575 |
| 31879190.8074388 | 16.8909677734906 |
| 31926067.1975848 | 18.7945149284128 |
| 31996551.0196494 | 21.0934950938333 |
| 32000000 | 22.9787413064524 |
| 32000000 | 24.1595688463008 |
| 32000000 | 24.4262209559266 |
| 32000000 | 23.6161184450322 |
| 32000000 | 21.4361405120067 |
| 32000000 | 17.3451729604313 |
| 31744571.5851591 | 10.1882350340179 |
| 17607003.8940125 | 172.172804494791 |
| 30588794.5648767 | 176.229443434909 |
| 30423620.914809 | 177.09625067114 |
| 30340628.9707765 | 178.708958376679 |
| 30307235.7165855 | -179.764604337692 |

| | |
|---|---|
| 30282922.1598205 | -178.841229374117 |
| 29378273.6531035 | -178.748184480692 |
| 22728057.0192086 | -179.93944172362 |
| 16752136.8956407 | 175.182296244047 |
| 6981946.20254203 | 150.668160028864 |
| 26683595.2967924 | 10.2604952140726 |
| 31688214.4152153 | 5.4561195931892 |
| 31025594.3674203 | 4.35822885782984 |
| 29212234.5568109 | 2.92855071398221 |
| 17586477.511583 | 0.188095245234273 |
| 2037916.7082263 | -141.092510871818 |
| 17854189.7946334 | -172.366093167062 |
| 29704027.3733436 | -173.769352240464 |
| 31999172.9909698 | -173.471479844325 |
| 7083104.46589778 | -138.18152572623 |
| 14944894.3245478 | -29.5429331983203 |
| 19249364.0946046 | -29.7600739917636 |
| 24591277.431542 | -24.4912811617379 |
| 30850574.5247554 | -17.9839768262015 |
| 31784143.0233202 | -12.4187379274474 |
| 31797260.5564037 | -7.83659599623729 |
| 31818642.8718809 | -4.598630961686 |
| 31855486.4758511 | -2.66244266775085 |
| 31913559.4848515 | -1.77573002601317 |
| 31989657.8918658 | -1.70662532500701 |
| 32000000 | -2.07250261461198 |
| 32000000 | -2.52723256325109 |
| 32000000 | -3.63456848094013 |
| 32000000 | -5.59709352834493 |
| 32000000 | -8.14666943940004 |
| 7261915.85711306 | -52.3962473088624 |
| 17371012.1555638 | -158.149454132334 |
| 29445785.9446898 | -167.371008436717 |
| 31831714.1655758 | -170.206969627282 |
| 27838863.6077166 | -172.30704121573 |
| 12881739.1303948 | -172.228922998097 |
| 8519801.27666633 | 0.300873628534452 |
| 15432836.5034253 | 5.07268662697607 |
| 16701357.1019556 | 7.81659152229743 |
| 19158901.6507805 | 8.27258981809449 |
| 21757710.9750621 | 7.22167210554742 |
| 23678223.1659668 | 5.22448179959281 |
| 23913504.9497093 | 2.4628005873974 |
| 22045578.849235 | -1.43727015496187 |
| 18289750.0557549 | -7.56609445637295 |
| 13486903.6236637 | -18.6567721948316 |
| 6298651.01077242 | -104.610227514543 |
| 19694944.092447 | -157.405448774748 |
| 28085628.3682 | -162.132441780207 |
| 27066102.7439014 | -160.25996837016 |
| 17010598.8234796 | -147.888049793926 |
| 11127608.5665042 | -131.418421055984 |
| 7022941.1696819 | -93.8044729086555 |
| 6964432.72061096 | -47.3009070569767 |
| 8887260.64317961 | -18.9397433303851 |
| 12713751.8814842 | -2.61936518253686 |
| 21533223.1166454 | 4.09512197250345 |
| 31999569.4590029 | 5.05234755156309 |
| 31999203.1459131 | 5.1602677622326 |
| 31998904.4446883 | 4.01511121840419 |
| 31998756.0386948 | 1.78098652075044 |
| 31998768.8226691 | -0.942572677731993 |
| 31998955.91764 | -3.59810168579524 |
| 31999318.8105255 | -5.812873280653 |
| 31999834.4372349 | -7.43817646051955 |
| 32000000 | -8.47008987460263 |
| 32000000 | -8.93679405594916 |
| 32000000 | -8.80834854307886 |
| 32000000 | -7.92713956804671 |
| 31907793.4810855 | -5.93475326478961 |
| 31551221.970416 | -3.86222929493487 |
| 11925608.8856616 | 178.527010131508 |
| 31997587.7789605 | 175.229392573192 |
| 31997592.9094064 | 174.541848987468 |
| 31997473.1924112 | 174.409277566356 |
| 31997251.7989151 | 174.447759120088 |

| | |
|---|---|
| 31909534.8944333 | 173.51476539763 |
| 14294736.0722546 | 161.848077372596 |
| 14868763.4787237 | 18.6431179943708 |
| 32000000 | 9.82927253628736 |
| 32000000 | 9.78352003417484 |
| 32000000 | 11.7821030117904 |
| 32000000 | 14.4243773095533 |
| 31999715.9180707 | 17.1433460660055 |
| 31998682.1428162 | 19.6063947647907 |
| 31997818.6776807 | 21.3568509106326 |
| 31997254.1310679 | 21.6719274272339 |
| 31997033.162555 | 19.8148386485995 |
| 31997154.0053964 | 15.4186649445818 |
| 31997577.4114941 | 8.64012139735497 |
| 30105748.4902169 | -0.140637188683317 |
| 25826777.5280113 | -12.0231442334337 |
| 21125686.1798738 | -28.9110462459633 |
| 17317601.5165216 | -54.4939580362126 |
| 17467190.9244179 | -106.16086226072 |
| 31977389.0014149 | -150.905204834843 |
| 31941892.8652781 | -159.585504661772 |
| 31931799.4264882 | -165.299032681308 |
| 31930676.5858485 | -169.186717742452 |
| 31920109.4972677 | -172.458048888389 |
| 31885588.1861918 | -174.706526343258 |
| 31501609.955272 | -174.12702884181 |
| 17415448.6121959 | -165.144398117143 |
| 13230037.95139 | -13.9746516551257 |
| 31999221.5330987 | -3.01903631626404 |
| 31998022.0671097 | -1.41848148331361 |
| 31996804.5420918 | -1.50202690250113 |
| 31995640.0608059 | -2.35785446995734 |
| 31876337.9655993 | -4.37770820980779 |
| 4764753.11784228 | -115.245761773882 |
| 32000000 | -171.522954744387 |
| 32000000 | -170.356237489148 |
| 32000000 | -169.108820522871 |
| 32000000 | -167.895212503398 |
| 32000000 | -166.447839342217 |
| 32000000 | -164.678559491727 |
| 32000000 | -162.743358452551 |
| 32000000 | -161.0848116122 |
| 32000000 | -160.581337001746 |
| 32000000 | -162.982358267957 |
| 20308464.4175404 | -162.671367558193 |
| 29996250.3285872 | -6.06547418912504 |
| 31997520.1456752 | -5.09488313859355 |
| 31997723.6994666 | -3.27682974723751 |
| 31998110.1964358 | -1.48531606315027 |
| 31998663.4062962 | -0.26867635188265 |
| 31999335.8522271 | 0.0446988606816139 |
| 32000000 | -0.797546707075335 |
| 32000000 | -2.97955765011025 |
| 32000000 | -6.57459508199764 |
| 32000000 | -11.4630933284505 |
| 32000000 | -17.2323436583772 |
| 31632484.3054698 | -23.1186237002874 |
| 30629954.5326056 | -28.1028692799636 |
| 29945360.4465388 | -32.6772525617573 |
| 24430182.2585711 | -38.8308130415305 |
| 23027300.2716425 | -37.1333372050973 |
| 23474066.9553823 | -31.27865398116 |
| 26204620.2166742 | -23.0549308018974 |
| 28333812.8711546 | -14.6916370455612 |
| 29471021.5170968 | -8.9097226165674 |
| 30838758.3981623 | -4.85632873417608 |
| 31815838.1916817 | -2.05420762614565 |
| 30288891.5082776 | -0.42177926937694 |
| 22408182.126237 | 0.94100338636316 |
| 16107426.6398943 | 0.455713606895077 |
| 12301324.5366875 | -3.93369302166079 |
| 3819367.49583404 | -38.6734801536032 |
| 4528351.38638317 | -71.7210887711995 |
| 17934942.1355668 | -19.2376114967063 |
| 26074121.1529757 | -13.8968459173576 |
| 24880041.0026372 | -12.5718419706111 |

| | |
|---|---|
| 23792673.1659424 | -8.60109325835938 |
| 23086512.4429981 | -1.26144835608198 |
| 23382789.1814489 | 8.95278188197917 |
| 23810774.6998138 | 20.3420986588023 |
| 14119034.6461881 | 61.8627253442212 |
| 17176549.0631951 | 108.497779310901 |
| 20404232.2908693 | 99.4042898625409 |
| 29924490.8570925 | 54.3397384472046 |
| 32000000 | 28.4422564629297 |
| 32000000 | 25.8059824552177 |
| 32000000 | 24.2386441860689 |
| 32000000 | 22.9987319966663 |
| 32000000 | 22.1612123331138 |
| 32000000 | 21.9171447840162 |
| 32000000 | 22.5562243690425 |
| 32000000 | 24.3773941738097 |
| 32000000 | 27.5119269652495 |
| 31669030.1409748 | 31.5950810943634 |
| 28963695.0153809 | 36.5655645834805 |
| 20819523.2565099 | 53.7101952863028 |
| 13197762.6136442 | 87.6211459245552 |
| 9853711.07639821 | 79.6002149825878 |
| 8844284.13005691 | 37.9345699597622 |
| 13779052.946135 | 4.71701288070758 |
| 24168086.3740766 | -6.67001399874608 |
| 28870049.3594556 | -10.005726480146 |
| 31997141.8188862 | -11.2303503755875 |
| 31997197.0830548 | -11.6365069596477 |
| 31997534.3282098 | -12.2450056924024 |
| 31998101.5867474 | -13.700040701522 |
| 31998801.3385023 | -17.3681654798728 |
| 27753717.141382 | -43.2691432196711 |
| 15686406.0750002 | -113.743818834981 |
| 19241156.7322158 | -157.365001487927 |
| 16995661.8035304 | -175.437202877973 |
| 8908054.05126108 | 170.479533558 |
| 1323244.35224834 | 16.5268612600308 |
| 2999922.4561098 | -85.3488520552095 |
| 6637900.65397133 | -89.9466485677338 |
| 10655301.8782584 | -74.8611153135403 |
| 13313824.826542 | -87.7783215435572 |
| 15164647.8624996 | -100.142815190932 |
| 15399985.94536 | -92.8300940698302 |
| 17971664.8408412 | -59.8952894163349 |
| 31996585.7560663 | -30.9785770850994 |
| 31996417.9839628 | -24.5348167151422 |
| 31996925.0778499 | -25.5193860442228 |
| 31997590.1188105 | -25.1297032431393 |
| 31998363.25933 | -22.9920805984869 |
| 31318760.5951485 | -19.0584325544893 |
| 30559548.797692 | -13.5676038793339 |
| 30532948.6829417 | -7.22487150474514 |
| 15895709.463226 | -0.888012156871664 |
| 23010334.5546969 | 169.139353417176 |
| 28990036.3502416 | 163.747128547068 |
| 28566303.5312542 | 158.509050847891 |
| 28354000.9707673 | 157.023768636347 |
| 28476161.386632 | 159.280132276935 |
| 29212135.2605238 | 164.754725795827 |
| 25630738.8682256 | 171.104491535614 |
| 6162760.86693171 | -179.448477295751 |
| 3457929.84738557 | -86.0587479433201 |
| 11862630.5082747 | -149.601493382469 |
| 27710976.7028593 | -164.073665273973 |
| 31997956.3207256 | -170.824888584902 |
| 31997883.0315333 | -172.836380394411 |
| 31997760.5423067 | -174.668081062202 |
| 31997544.610259 | -175.954544942841 |
| 31997197.0426602 | -176.011662196813 |
| 31913623.7661259 | -173.753091474261 |
| 12664765.4058092 | -146.017710731018 |
| 32000000 | -13.7468803699698 |
| 32000000 | -16.233082909059 |
| 32000000 | -18.2361447054512 |
| 32000000 | -19.2299809250338 |
| 32000000 | -19.2341725115205 |

| | |
|---|---|
| 32000000 | -18.4313325583388 |
| 32000000 | -17.0195297996501 |
| 32000000 | -15.2008362112403 |
| 32000000 | -13.2156318385436 |
| 32000000 | -11.3319839212963 |
| 32000000 | -9.62929824558471 |
| 31858723.9986829 | -7.6201225504184 |
| 25589658.6371393 | -3.52173930488944 |
| 28249010.3886773 | -0.794193211508167 |
| 31999853.7945142 | -0.0299229401081557 |
| 31999801.2929685 | -0.0492010352150012 |
| 31999830.4574394 | -1.13049654014075 |
| 31999901.7779411 | -2.33835390876937 |
| 31999981.2637464 | -3.05821989643799 |
| 31783006.7493042 | -2.75282123812067 |
| 30638190.6280524 | -0.565898591594856 |
| 28944800.7966033 | 4.97466723403242 |
| 24980395.9387142 | 16.8194622120786 |
| 9865666.32373833 | 95.0743239930917 |
| 17193713.5983478 | 145.963449193625 |
| 19763665.5025348 | 154.904983172169 |
| 12297711.832685 | 147.1614727424 |
| 10575369.5384955 | 29.1798351437981 |
| 32000000 | 6.77459323260616 |
| 32000000 | 3.67461584382535 |
| 32000000 | 2.6528066532974 |
| 32000000 | 2.0488974185691 |
| 32000000 | 1.65465336631041 |
| 32000000 | 1.36655627018941 |
| 32000000 | 1.16233971924286 |
| 32000000 | 1.11368459300488 |
| 32000000 | 1.45104239172728 |
| 32000000 | 2.66984706241122 |
| 32000000 | 5.5557190618997 |
| 32000000 | 10.7869037431441 |
| 14828186.065516 | 45.799078967069 |
| 23687699.6443456 | 160.125284287112 |
| 30246965.8177077 | 171.522080758726 |
| 32000000 | 178.733819033012 |
| 16885438.622636 | -172.34478916751 |
| 25193959.9318603 | -3.74727512508817 |
| 29442308.7961319 | 0.22217389158923 |
| 32000000 | 2.15138284119074 |
| 32000000 | 3.08717038327977 |
| 32000000 | 3.57621114151822 |
| 32000000 | 3.88271611333344 |
| 32000000 | 4.13977885385636 |
| 32000000 | 4.4863901711686 |
| 32000000 | 4.91426563661267 |
| 32000000 | 5.43425998117973 |
| 32000000 | 6.05570314938164 |
| 32000000 | 6.8073815813243 |
| 32000000 | 7.78213925493854 |
| 27631745.8357161 | 11.2541477393187 |
| 8053031.44357943 | 38.747490942306 |
| 11691057.7491905 | 158.316948454427 |
| 26154102.1169211 | 172.782460174741 |
| 31999954.753748 | 176.717604052283 |
| 32000000 | 179.302740670879 |
| 30845825.2551176 | -178.083154355618 |
| 20156105.8586307 | -173.956055251489 |
| 4436998.43837359 | -145.318283046251 |
| 12355460.7807567 | -9.1275049922936 |
| 13194385.3773061 | -2.82729770808361 |
| 14098827.1631555 | 2.84764638741782 |
| 14564649.035245 | 8.24576601910595 |
| 16355503.0215254 | 12.2281285441913 |
| 19932597.0671392 | 14.0421948000028 |
| 22281077.6476005 | 14.8757523090746 |
| 24826514.2557141 | 14.7353829785118 |
| 28274222.0873344 | 13.9452616010848 |
| 30253993.0225724 | 13.006281071997 |
| 31380992.5146268 | 12.209942926474 |
| 32000000 | 11.8986150097526 |
| 31999978.0245329 | 12.2262108160269 |
| 31999833.8640518 | 13.1120624158939 |

| | |
|---|---|
| 31999686.6394383 | 14.7632483083753 |
| 23660606.4488062 | 32.076070743143 |
| 15013576.6423432 | 124.248389686332 |
| 14663164.1437443 | 122.378728020913 |
| 13504314.8114352 | 118.799744863366 |
| 11661365.995108 | 108.503187302698 |
| 10337279.5089899 | 85.2714038183933 |
| 11821468.3377837 | 55.1962934120398 |
| 15811018.7562904 | 35.8733968169285 |
| 19367341.5993356 | 27.0714756253781 |
| 19695817.9923711 | 24.3109804969227 |
| 14761488.7195439 | 28.1669037490409 |
| 5535580.25994692 | 76.909590705058 |
| 17745762.1764768 | 168.514843045399 |
| 31998057.2541166 | 177.584537055257 |
| 31998433.1848669 | 179.635748616307 |
| 31998820.5951742 | -179.628577389756 |
| 31999094.8880175 | -179.589245285133 |
| 31999156.9415829 | 179.961380507215 |
| 31998949.5726906 | 179.199877916299 |
| 31998469.7892645 | 178.071070864323 |
| 31949126.8361922 | 175.104942219829 |
| 9775563.59951388 | 144.396591805896 |
| 30107813.1417383 | 15.7586792555924 |
| 32000000 | 10.0621496523819 |
| 32000000 | 10.0190917171366 |
| 32000000 | 10.1476833270187 |
| 32000000 | 10.1269528492064 |
| 32000000 | 9.80992079803204 |
| 31999769.8994925 | 8.93513103973963 |
| 31998204.8744866 | 7.03093089070713 |
| 31754250.6259648 | 3.51468613780205 |
| 24887227.0071967 | -0.688719615407006 |
| 16335625.7684805 | -7.19159759766816 |
| 12012767.3600429 | -15.9241444583099 |
| 13924284.6546849 | -17.0901200140272 |
| 9428940.99763327 | -26.484393897535 |
| 12189614.4440401 | -15.9280112640742 |
| 22890187.1227609 | -4.67532984493559 |
| 31999980.8361973 | -0.193088296359661 |
| 32000000 | 2.23051683823042 |
| 32000000 | 3.91963258974299 |
| 32000000 | 5.65406596068351 |
| 29724745.7194654 | 7.5002129498991 |
| 22644899.3595317 | 8.85955685762105 |
| 17890776.4568139 | 7.6709597216312 |
| 12585943.8687565 | 2.57531237289769 |
| 8435840.50251906 | -172.606103585872 |
| 22069242.8586366 | -173.91658760333 |
| 26417907.4630664 | -173.05387572502 |
| 21066543.2704618 | -170.108251756521 |
| 21185886.3037877 | -170.948945897978 |
| 16668257.253497 | -170.706268239263 |
| 3027028.96677416 | -39.8687143465482 |
| 16505502.7188172 | -7.63534056069382 |
| 22688941.302851 | -8.98341957853744 |
| 18822427.6644052 | -17.6477656953819 |
| 9853960.65314668 | -57.8356857294613 |
| 16507140.8447788 | -136.575512867419 |
| 28469258.5573887 | -158.803047943288 |
| 30529963.0616332 | -158.779542408466 |
| 31979377.9608417 | -154.349786199967 |
| 31998879.8471226 | -149.713280567967 |
| 31998840.116085 | -139.350009708977 |
| 32000000 | -44.7059703853658 |
| 32000000 | -30.9077317913009 |
| 32000000 | -24.4046531921336 |
| 32000000 | -19.4289117078015 |
| 32000000 | -16.5649923024741 |
| 32000000 | -15.888212057978 |
| 32000000 | -17.456257221924 |
| 32000000 | -21.1733624905355 |
| 32000000 | -26.1165129423394 |
| 31998796.2467947 | -37.4759271289836 |
| 23196774.7861097 | -129.851048628138 |
| 25668150.9405215 | -147.036755580594 |

| | |
|---|---|
| 24953845.5176257 | -141.148731731223 |
| 18577730.4849641 | -60.1537472631961 |
| 31998442.7070245 | -17.5054792261444 |
| 31998610.6381956 | -10.2857735861057 |
| 31998799.5948691 | -6.05063403112999 |
| 31998943.4931642 | -3.83002907495341 |
| 31170572.1309767 | -2.89936788568251 |
| 30048428.2660212 | -2.91046196788644 |
| 26000137.5154017 | -4.12070841370866 |
| 21495466.6096444 | -6.52020310848811 |
| 6193963.85753308 | -47.8599090389813 |
| 7774170.69122507 | -120.78280865531 |
| 10973132.842738 | -39.9165166352311 |
| 21787794.543321 | -12.4358828989464 |
| 28815402.7896128 | -1.69728509222726 |
| 32000000 | 3.59981631041298 |
| 32000000 | 5.60604599527569 |
| 32000000 | 6.42712402841503 |
| 32000000 | 6.98638185560685 |
| 32000000 | 7.52584621824652 |
| 32000000 | 8.08629792203789 |
| 32000000 | 8.70688674317864 |
| 32000000 | 9.87838305362453 |
| 32000000 | 16.3625722740045 |
| 20555829.1037377 | 32.0488544818248 |
| 6805172.28874849 | 129.829150121178 |
| 15859270.1507652 | 177.553426140369 |
| 18058903.4257297 | -174.386308011383 |
| 12187591.2847655 | -172.416053381473 |
| 22285505.2762192 | 179.763841868172 |
| 31999588.7494583 | 176.876334348074 |
| 21455465.0706942 | 167.935568642657 |
| 13066237.6625173 | 144.369273395143 |
| 10658799.4428218 | 96.4037053892505 |
| 16097935.3209988 | 53.7273779720559 |
| 27159596.0619265 | 32.522177389554 |
| 31359465.2093522 | 26.5096008618164 |
| 31312586.023923 | 25.5694726478787 |
| 30877940.8857265 | 22.9650762592627 |
| 28596073.4047087 | 18.8285137289036 |
| 24020107.7698172 | 14.2734654150892 |
| 13185786.9410192 | 9.0097627186976 |
| 23422961.8545234 | -177.907938014992 |
| 31390438.8113802 | -176.144152712246 |
| 31551742.0517638 | -175.539495922242 |
| 31784625.3557205 | -176.507936029916 |
| 31880134.7841103 | -178.395781723717 |
| 31966138.6157885 | 179.291712772431 |
| 31988405.7341555 | 176.993277616482 |
| 31996283.513219 | 175.552491846365 |
| 18165714.3404587 | 2.76554691717302 |
| 31861525.3000742 | 4.9600737443412 |
| 32000000 | 4.49475390312103 |
| 32000000 | 1.72403878670497 |
| 32000000 | -0.587379091324117 |
| 32000000 | -1.75289325888952 |
| 32000000 | -1.94471358222357 |
| 32000000 | -1.49695002987286 |
| 32000000 | -0.726725653166229 |
| 32000000 | 0.050404460282724 |
| 31999552.9060946 | 0.461652982324389 |
| 31999151.423658 | 0.0344695924939616 |
| 31998951.6957105 | -1.76827464057275 |
| 31999002.6958641 | -5.32592445759935 |
| 31999266.2205364 | -10.3433733345834 |
| 31933096.4583612 | -15.4124411518891 |
| 27858419.9081912 | -19.772515080236 |
| 9992673.11112986 | -127.343474353819 |
| 31486290.7606517 | -170.695697846001 |
| 31837683.9647673 | -177.340881565323 |
| 31040401.1947839 | 176.034055697473 |
| 18400410.6750992 | 162.565200945914 |
| 10365361.940769 | 51.1227082561044 |
| 22699890.3616679 | 25.5071634224333 |
| 26744582.5972653 | 23.5501025219168 |
| 29833367.3593747 | 21.2856753790455 |

| | |
|---|---|
| 31173976.9890241 | 19.4169596540546 |
| 30840767.1400703 | 17.9165666276773 |
| 28999075.8682862 | 16.8268433538114 |
| 27561529.954391 | 15.0245966288177 |
| 28013288.4648831 | 11.5854746341828 |
| 24887946.5240109 | 8.97641952433762 |
| 16435695.5867461 | 7.58871149146733 |
| 10384472.7185777 | 2.54787063947789 |
| 5402644.52904787 | -14.3388171323672 |
| 3442986.76167221 | -71.0171584000211 |
| 5471606.08159772 | -104.825326885245 |
| 14853518.8424889 | -152.31579481808 |
| 28159740.7730959 | -164.381116197531 |
| 27692712.7540975 | -163.141323791917 |
| 25774868.3210648 | -162.047783899443 |
| 25012322.1247428 | -163.248397894512 |
| 25047134.5796734 | -167.056080257923 |
| 12722737.9220216 | -161.499784058176 |
| 30231334.0763237 | -9.36238013899425 |
| 32000000 | -10.7333702488259 |
| 32000000 | -12.5820898963441 |
| 32000000 | -13.0574163660416 |
| 32000000 | -12.4884667910567 |
| 32000000 | -11.3046426075898 |
| 32000000 | -9.80562987760615 |
| 32000000 | -8.13903944059568 |
| 32000000 | -6.37720591460629 |
| 32000000 | -4.58422094759369 |
| 32000000 | -2.82545074941832 |
| 31952148.4149153 | -1.09533943957072 |
| 31800110.4582954 | 1.29434896424233 |
| 22174675.6517388 | 7.50825261131056 |
| 6060903.3804756 | 31.1631794399758 |
| 4298322.97476863 | 56.0480052611505 |
| 12395231.5878522 | 18.2388115315466 |
| 29161996.6742438 | 7.0115809090413 |
| 29920197.4711057 | 4.23672483098622 |
| 30446013.3372545 | 2.00456966933171 |
| 30613113.7292464 | 0.845866802492687 |
| 30207820.1322021 | 0.7068685331163 |
| 29402249.344205 | 1.43602075681131 |
| 28403687.6006072 | 2.89871136006163 |
| 27291864.8961325 | 4.78150174182699 |
| 18716274.6637782 | 7.13045734695556 |
| 8932290.86466149 | 14.0876369930122 |
| 2875815.27022614 | 45.1825994712162 |
| 5242466.28758433 | 21.4367748095534 |
| 19589297.4296826 | 4.74996742479138 |
| 31997369.5682237 | 2.36443788119333 |
| 31997914.5146822 | 3.30710916577412 |
| 31998658.9823227 | 3.94083282367974 |
| 31999459.7771007 | 4.1565279667353 |
| 32000000 | 4.24798900090255 |
| 32000000 | 4.38212046961966 |
| 32000000 | 4.64961391501342 |
| 32000000 | 5.07087228319702 |
| 32000000 | 5.50975695991445 |
| 31998394.2284315 | 5.54728822631111 |
| 31888842.0829485 | 4.48404777527714 |
| 13211961.3268582 | 10.4957381185389 |
| 17939767.8719921 | 169.858806660777 |
| 27761190.1871673 | 170.881311703303 |
| 28515487.6995332 | 168.742708389677 |
| 28891166.6148004 | 167.380884956937 |
| 22812758.9186418 | 163.54156070288 |
| 5960423.05498488 | 122.444584467689 |
| 15511265.0156702 | 8.54935600674141 |
| 23950935.7501585 | -2.66215624559063 |
| 25764903.9946367 | -10.2862282519913 |
| 28133140.3521621 | -15.6573173416859 |
| 19988318.776163 | -30.0671175813985 |
| 12923622.1219971 | -121.677459978492 |
| 30220370.7940564 | -159.621394259832 |
| 30469227.9235174 | -163.600788753736 |
| 30630339.1158242 | -168.662514026677 |
| 30596486.4299603 | -174.225812133652 |

| | |
|---|---|
| 30707905.8387542 | -179.867097636978 |
| 30931024.5571221 | 174.011794945874 |
| 28931718.94827 | 165.228218574521 |
| 16838035.5569909 | 37.1664267343133 |
| 32000000 | 17.1266702359545 |
| 32000000 | 14.9847849553087 |
| 32000000 | 13.1366432629384 |
| 32000000 | 11.5644473474188 |
| 32000000 | 10.1208529367896 |
| 32000000 | 8.66940925741936 |
| 32000000 | 7.12722805051343 |
| 32000000 | 5.42829225232646 |
| 32000000 | 3.36384931885117 |
| 32000000 | 0.56219982491243 |
| 32000000 | -3.27727298285681 |
| 31126286.8272207 | -8.70647585639403 |
| 22198785.953821 | -19.0402389242792 |
| 16555982.2655088 | -31.19506836163 |
| 17827125.929241 | -32.5306340547578 |
| 26422201.4621476 | -23.9568416218147 |
| 30673210.2793132 | -20.8546447054709 |
| 31961201.8329441 | -18.3220431818094 |
| 32000000 | -15.9182436181285 |
| 32000000 | -13.9533715251485 |
| 32000000 | -12.5067668522026 |
| 32000000 | -11.5992977873125 |
| 32000000 | -11.2860617383763 |
| 32000000 | -11.6979309109877 |
| 32000000 | -13.0902511900463 |
| 32000000 | -15.9080696564681 |
| 31520001.2218419 | -24.0703548009942 |
| 31999442.2822874 | -164.166900104831 |
| 32000000 | -169.346502970516 |
| 32000000 | -171.546705040882 |
| 32000000 | -172.446776548332 |
| 32000000 | -172.493699668016 |
| 32000000 | -171.970196973261 |
| 32000000 | -170.985299614249 |
| 32000000 | -169.475809019329 |
| 32000000 | -167.212392978735 |
| 17776315.0567211 | -134.483144044566 |
| 30916996.2913761 | -20.1824953532293 |
| 31998127.9876116 | -13.3684364309547 |
| 31998620.5564475 | -9.19909600878588 |
| 31999045.8671975 | -6.51369143969664 |
| 31999214.1344331 | -4.78779681671164 |
| 31999302.8120279 | -3.72392610721306 |
| 31999322.4186853 | -3.04546630188122 |
| 31999270.1369894 | -2.50344998813043 |
| 31999155.4930865 | -2.20716824588235 |
| 31998981.9523176 | -1.95263152780457 |
| 27357663.9339169 | -4.75786741625491 |
| 16879704.9057923 | -13.0545060794774 |
| 10472872.8914098 | -32.2780232859552 |
| 9087238.66942226 | -54.1519646366609 |
| 9050701.78424211 | -81.6995350893972 |
| 15055343.659896 | -135.656067359041 |
| 14931350.2754046 | -125.23004528199 |
| 17630111.9009343 | -47.7865438031214 |
| 20993861.733681 | -22.8587113631308 |
| 22830442.6777212 | -14.0812876594051 |
| 25377322.3490215 | -7.01928001056709 |
| 28137776.0445787 | -1.58580072809238 |
| 30612315.4636683 | 2.67823131924352 |
| 32000000 | 6.4830199707687 |
| 32000000 | 10.5668464319776 |
| 32000000 | 15.60624450192 |
| 32000000 | 22.3809021000731 |
| 32000000 | 31.6541501986132 |
| 31999876.6815525 | 57.2972343986335 |
| 31999316.5968762 | 142.509593305426 |
| 31999915.7434972 | 150.752788745316 |
| 32000000 | 154.873086096711 |
| 32000000 | 156.736707493697 |
| 23279057.2603464 | 133.140904948291 |
| 30138715.6456459 | 29.6244184475289 |

| | |
|---|---|
| 31997548.5087262 | 20.4191194322195 |
| 31997832.0147887 | 15.3051918719323 |
| 31998051.6117358 | 11.9570254178797 |
| 31998179.3036118 | 9.78435327518819 |
| 31998204.4678589 | 8.41178920048394 |
| 31998135.713453 | 7.6773466394286 |
| 31998005.3030349 | 7.68233315956667 |
| 31997874.9900996 | 8.88642012831672 |
| 21587373.6002546 | 13.7745529669462 |
| 12115572.3082084 | 155.348389682371 |
| 32000000 | 174.138199076419 |
| 32000000 | 174.895379273186 |
| 32000000 | 175.456113253281 |
| 31999894.6520767 | 175.685210303821 |
| 22385904.7206244 | 174.558558802711 |
| 10538099.5172686 | 170.062250805359 |
| 1688434.27067799 | 82.3357146369844 |
| 8588562.42595127 | 11.599450499086 |
| 13621748.0317416 | 8.50843061149046 |
| 15262017.540131 | 9.6560768625018 |
| 13477652.8784528 | 14.3973615307804 |
| 8746719.04334696 | 29.8129044288551 |
| 5634493.97552186 | 102.056769626179 |
| 14709357.6000329 | 152.317745723218 |
| 28862761.1851537 | 163.179226706442 |
| 31370334.3443075 | 167.187817791067 |
| 31403242.7369977 | 166.127544724036 |
| 31353393.5275617 | 163.906636998515 |
| 31299943.0146001 | 162.169033716753 |
| 30668883.1724056 | 161.514464910766 |
| 29439047.0181086 | 160.010118102052 |
| 13737509.0979818 | 135.034058381062 |
| 18175256.3805612 | 29.1809771967597 |
| 32000000 | 14.2363393539312 |
| 32000000 | 11.368176072903 |
| 32000000 | 10.6150474735876 |
| 31898121.8184463 | 10.2606605234274 |
| 31629520.8499703 | 10.2496461578131 |
| 31449104.257218 | 10.6025396525259 |
| 31442327.6524622 | 11.4172992173502 |
| 31552920.5657088 | 12.8836285291855 |
| 31687165.8454819 | 15.3294886510368 |
| 31741569.6721642 | 19.2599361628184 |
| 31227782.9452545 | 25.2500106874066 |
| 28029585.6858397 | 34.0018514176283 |
| 23324809.8465376 | 45.8701441268838 |
| 17860918.0187687 | 71.2960166450227 |
| 22639319.0447542 | 136.870384225306 |
| 23926175.1450641 | 140.044470402878 |
| 14142993.5814965 | 80.7492765753413 |
| 19233509.5003266 | 32.3456931731199 |
| 30503348.3629928 | 9.81537336396885 |
| 32000000 | 1.0194716691015 |
| 32000000 | -3.45626579695283 |
| 32000000 | -5.72558987490185 |
| 32000000 | -6.93688949602217 |
| 32000000 | -7.86456073544864 |
| 32000000 | -9.38989829608122 |
| 32000000 | -13.0661318138686 |
| 30207613.1294801 | -21.9202423865604 |
| 19959428.7261086 | -144.103093296772 |
| 31999103.504 | -177.722338818557 |
| 31999606.5565649 | 175.166392288042 |
| 31999923.6054214 | 171.748774648106 |
| 31999918.7659663 | 170.74447577317 |
| 31999630.3482719 | 171.585897969594 |
| 31998958.4970593 | 175.836815708283 |
| 3077908.2984152 | -60.6214201280786 |
| 30337892.4426897 | -16.5312797604727 |
| 32000000 | -21.4998579530433 |
| 32000000 | -25.3150305406987 |
| 32000000 | -29.1817616136392 |
| 32000000 | -34.4076505748493 |
| 32000000 | -41.8633509263679 |
| 32000000 | -51.228099493891 |
| 32000000 | -61.7639077926373 |

| | |
|---|---|
| 32000000 | -73.6602808997707 |
| 32000000 | -79.4307907894908 |
| 31269951.7107682 | -68.1266325876787 |
| 30744422.0274578 | -50.4611710229603 |
| 31868238.8949414 | -30.9058206429961 |
| 31998555.7461787 | -16.3239431308114 |
| 31999052.919147 | -6.81492954621506 |
| 31999487.9816894 | -1.26599423316381 |
| 31796670.0028519 | 1.77402199810059 |
| 31011324.8799981 | 3.63417248410935 |
| 29567025.3906732 | 6.02493090995867 |
| 27132481.343087 | 12.2093645219583 |
| 23420994.5404284 | 28.6433824914308 |
| 19309288.6946589 | 114.439565977516 |
| 32000000 | 169.784146649745 |
| 32000000 | 178.631555113567 |
| 32000000 | -179.846784594434 |
| 21452309.1931355 | 165.905087785323 |
| 22343809.7753328 | 31.0408825072532 |
| 31999195.2435967 | 20.6821697027843 |
| 31999538.2420169 | 20.5909501057919 |
| 31999751.4780151 | 20.2824861231088 |
| 31999785.8886934 | 19.6123996426682 |
| 31999627.4516778 | 18.3142475467176 |
| 31999294.6628298 | 16.1398903844508 |
| 31998836.8096478 | 12.9710793186924 |
| 31998323.4936494 | 9.04369353415901 |
| 31222551.5611675 | 5.28028008096049 |
| 29975133.7813448 | 3.2548685253227 |
| 30465577.0904095 | 4.37725231149758 |
| 31730463.0699671 | 8.4730804842051 |
| 31961464.3323015 | 13.8694503548675 |
| 31998698.6447568 | 18.4184518436312 |
| 31999131.9233916 | 21.227020467688 |
| 31999484.5152379 | 22.4199565432248 |
| 31999726.2995782 | 22.4525548478813 |
| 31999843.9706153 | 21.7780310819216 |
| 31999841.5034001 | 20.8684195424853 |
| 32000000 | 44.5847579059592 |
| 24504182.2538955 | 96.3160879947946 |
| 30444017.5220469 | 128.759438890238 |
| 31453700.5475751 | 142.026139822232 |
| 31869457.7905459 | 149.089111822126 |
| 32000000 | 145.573674988206 |
| 25906665.6728894 | 121.954691190132 |
| 21663436.6159331 | 73.7761756507488 |
| 28866530.6352693 | 40.902082147868 |
| 32000000 | 26.9206865472064 |
| 32000000 | 19.6726317444615 |
| 32000000 | 15.3892251751896 |
| 25683184.4930473 | 12.753841366622 |
| 16454798.4901573 | 12.0063435073405 |
| 13636795.5657058 | 8.2709236620977 |
| 9547932.46883004 | 6.95143419691295 |
| 3276494.59072406 | 15.5442811644037 |
| 5641593.06062832 | 170.032649884805 |
| 16904447.1221331 | 175.613070359827 |
| 20456227.9452579 | 175.41375182823 |
| 21749183.7968552 | 175.286775623223 |
| 26429241.4676818 | 176.536382583396 |
| 17921684.4331745 | 176.87870552842 |
| 22454632.0854249 | -179.725215758822 |
| 20697725.8082462 | -175.464617226806 |
| 14026640.2144489 | -165.855535210717 |
| 5799367.63437582 | -114.934046785668 |
| 13843021.4236886 | -30.5023057935752 |
| 27725853.1567152 | -18.4072279619018 |
| 32000000 | -15.6013689731587 |
| 32000000 | -15.2122695984931 |
| 32000000 | -17.1842625510326 |
| 30650760.4582908 | -19.0186584200942 |
| 27348949.3061961 | -19.4764700334454 |
| 23740495.5486029 | -17.6214875409638 |
| 21794272.3980035 | -12.5543050459126 |
| 21547951.8188742 | -4.72893825733231 |
| 24038465.9243702 | 3.11032987986613 |

| | |
|---|---|
| 28907403.9304663 | 8.53984845679288 |
| 31998718.9131645 | 11.7310117044442 |
| 31999328.0919182 | 13.7847111782289 |
| 31999998.247429 | 13.8759639792788 |
| 32000000 | 12.3914909172038 |
| 32000000 | 9.8610878637406 |
| 32000000 | 7.06459662618328 |
| 32000000 | 4.39254018649603 |
| 32000000 | 1.89919643344289 |
| 32000000 | -0.24404711461363 |
| 31999986.5810847 | -2.0206973241756 |
| 28485097.8214396 | -3.00069487917982 |
| 25363366.1509894 | -2.83982267359978 |
| 22840974.806995 | -1.06892900310497 |
| 20543922.0267928 | 1.84080925314425 |
| 11800040.9617722 | 9.86021578354414 |
| 3207850.27509548 | 95.6604179729561 |
| 9939027.04763516 | 156.199813089218 |
| 12754414.1393586 | 159.674934922355 |
| 19238537.7581993 | 167.52360713547 |
| 23069444.383243 | 172.559355811257 |
| 24587915.3199139 | 177.7387246834 |
| 24385348.7352924 | -176.081921310443 |
| 23064241.516616 | -168.583130466834 |
| 20702409.9956913 | -159.253587154827 |
| 16877793.9015528 | -145.306396738607 |
| 13417510.0855546 | -123.895402402513 |
| 18922243.0064868 | -37.4995129748155 |
| 22730944.4205126 | -28.3160674903694 |
| 29369209.7014108 | -16.6184281970924 |
| 29699246.5304701 | -8.89028182917177 |
| 30508479.9658287 | -4.06991277678978 |
| 31410503.6578826 | -0.22446493884369 |
| 31999452.1495029 | 2.52527500020483 |
| 31999366.3147696 | 4.08393081799916 |
| 31999432.2742287 | 4.4200339359761 |
| 31910186.3251472 | 3.37974689218621 |
| 29487478.1068551 | 0.510323927469123 |
| 27702126.1959989 | -3.99453912686907 |
| 27112410.2153484 | -9.09940862525908 |
| 28715351.4366726 | -12.7102066162664 |
| 31159467.6030216 | -14.0672047993304 |
| 28299635.7667323 | -16.2453086877947 |
| 27709963.0104281 | -16.1703911493393 |
| 32000000 | -10.6006231560478 |
| 32000000 | -4.65481457844341 |
| 32000000 | -1.07122188651307 |
| 32000000 | 1.84181103469607 |
| 31831001.8559037 | 3.82200375222091 |
| 31079348.9468941 | 4.68517627679821 |
| 30452217.9826873 | 4.36260982333243 |
| 30302940.7542851 | 2.94976052155931 |
| 30736159.8393968 | 0.829303130760126 |
| 31896593.7073144 | -1.4106604362336 |
| 32000000 | -3.18731010292392 |
| 32000000 | -4.22652182261954 |
| 32000000 | -4.5712381420709 |
| 32000000 | -4.43894345674322 |
| 32000000 | -4.06514839703244 |
| 32000000 | -3.64503094212676 |
| 32000000 | -3.34381446138945 |
| 32000000 | -3.31358922120446 |
| 31999976.0675888 | -3.67171097147044 |
| 31080915.5102479 | -4.34001713108566 |
| 28517315.7301836 | -4.64250804007677 |
| 26265479.0769573 | -2.49564990527446 |
| 8916445.18666651 | 10.4995661731924 |
| 19635907.1802252 | 170.610904631903 |
| 31997285.7636817 | 175.265731512976 |
| 31997109.1827061 | 177.788145578888 |
| 29483341.2157249 | -179.295184359705 |
| 26507066.4576095 | -174.365734492478 |
| 14094530.7321518 | -160.300980041813 |
| 6043965.61479605 | -79.9984522386838 |
| 12623866.9606 | -30.2850943797791 |
| 14990583.2856948 | -24.0831438721566 |

| | |
|---|---|
| 9682569.01576763 | -34.0158745765792 |
| 7721732.80389043 | -143.598694802397 |
| 28351425.0286731 | -171.89891978116 |
| 32000000 | -174.154360910476 |
| 32000000 | -175.067807234997 |
| 32000000 | -176.707654467601 |
| 32000000 | -178.777483337094 |
| 32000000 | 178.975934814273 |
| 32000000 | 176.874936192752 |
| 32000000 | 175.651008589414 |
| 13320844.37724 | 157.020876900798 |
| 9591327.28131396 | 57.2944558311316 |
| 27390438.3071477 | 21.2265729075205 |
| 30474559.7824228 | 17.3892658274152 |
| 32000000 | 13.670520260203 |
| 32000000 | 10.3576295958149 |
| 32000000 | 7.87708057910993 |
| 32000000 | 6.29129325979959 |
| 32000000 | 5.49944813651935 |
| 32000000 | 5.36451397727553 |
| 32000000 | 5.74833817998815 |
| 32000000 | 6.52316442330981 |
| 32000000 | 7.58745359316841 |
| 32000000 | 8.88153069115382 |
| 32000000 | 10.3391469166621 |
| 32000000 | 11.6435325996847 |
| 16681095.197418 | 31.2380055927452 |
| 7682985.46471666 | 109.71440936781 |
| 6112960.9748938 | 61.7560452565775 |
| 27882585.1591603 | 5.49065227301926 |
| 27865566.6159147 | -5.22440675064164 |
| 29016361.7908813 | -10.4277495232296 |
| 30356398.8469198 | -13.4309089141634 |
| 31394207.2328647 | -13.9323012350889 |
| 31869099.2380239 | -12.2085960373952 |
| 31985240.4614528 | -8.62662122378557 |
| 31300647.346831 | -3.99312489260474 |
| 28787721.7333786 | 1.1922905740895 |
| 26359160.039382 | 5.60326084865314 |
| 10684661.7001155 | 17.9766319513369 |
| 19639953.3648584 | 171.79513750837 |
| 23270160.822579 | 178.321199097767 |
| 17720526.1023088 | -170.992052011447 |
| 9380332.85525362 | -131.029411409327 |
| 13013959.1207051 | -63.4323520325207 |
| 22279628.6285217 | -45.3853238579539 |
| 28673097.4461689 | -41.9217587874373 |
| 23526044.3443909 | -64.6257023341233 |
| 25065603.9548449 | -118.358656796882 |
| 28585682.8056276 | -133.872170931935 |
| 29192607.697189 | -146.056487915761 |
| 29800836.9714484 | -158.437213217169 |
| 31517298.440487 | -169.814298904898 |
| 32000000 | -178.695589591271 |
| 32000000 | 174.703589125888 |
| 26701491.6268694 | 8.02633093444014 |
| 28974370.1439094 | -0.317364363809533 |
| 30224052.4596961 | -7.01027318032428 |
| 31743938.6988574 | -11.8328050696436 |
| 31999755.2416908 | -14.7665486241525 |
| 31999721.7740073 | -15.9105087641067 |
| 31999666.9036368 | -15.5193898296209 |
| 31999614.3890326 | -13.8957197468103 |
| 31999595.9530704 | -11.3297958517338 |
| 31873805.9626479 | -8.20444632329545 |
| 31758105.7493464 | -5.29275743880126 |
| 31469725.8877378 | -4.08165913966364 |
| 29333533.2491393 | -6.50866692180417 |
| 27735616.1589054 | -13.6846412961639 |
| 28014008.5649122 | -23.4722870749543 |
| 29609861.1417055 | -31.5774414731879 |
| 30769973.1710446 | -35.9724309203476 |
| 31672668.3516801 | -36.8798282224853 |
| 31787207.2257248 | -35.370436588147 |
| 31593728.2915859 | -35.9136017114933 |
| 25049625.6393817 | -42.9271760171193 |

| | |
|---|---|
| 13665077.8596367 | -58.3234131076216 |
| 6078813.33838734 | -75.5677929907456 |
| 7176768.82393967 | 4.10839372705331 |
| 26090794.5291236 | 18.411123521558 |
| 30642331.3634315 | 26.3367635379576 |
| 31864264.8007235 | 28.617497078715 |
| 31894115.2672583 | 24.9270183238638 |
| 31965498.6866765 | 19.1535940955971 |
| 32000000 | 13.7450075999466 |
| 32000000 | 9.85367586343217 |
| 32000000 | 7.68472215822087 |
| 32000000 | 7.02923673899054 |
| 31999920.2358327 | 7.59772077222324 |
| 31990257.6323314 | 9.19843620818426 |
| 31920485.1817 | 11.8363307559208 |
| 31848936.8962915 | 15.5558753004332 |
| 31812256.2338263 | 19.5581308596296 |
| 10545163.554475 | 44.7579268555427 |
| 32000000 | 174.536222963583 |
| 31962048.3747042 | 179.026564908764 |
| 31865465.200005 | -176.760374966778 |
| 31697822.5328205 | -171.93120050441 |
| 31585055.0583696 | -165.199073940716 |
| 14414107.7414867 | -132.52899812013 |
| 15745766.0581945 | -51.4001963862096 |
| 27535856.2765201 | -29.0994321132792 |
| 32000000 | -22.8168667886944 |
| 32000000 | -19.9408983884827 |
| 31769581.2207295 | -18.0973866425855 |
| 21329162.0168953 | -18.3761846858004 |
| 5476572.5005761 | -36.307445824024 |
| 11279880.7033238 | 178.958365275213 |
| 17747422.9386167 | 169.517250970715 |
| 27330404.8645527 | 168.713230715921 |
| 29802257.2691646 | 168.746290832778 |
| 30484459.6357003 | 170.066333027449 |
| 30987721.5296991 | 173.16818955508 |
| 31318189.86137 | 177.695376562071 |
| 31520189.8288534 | -176.784288949674 |
| 5063778.01732104 | -113.631314317037 |
| 23035578.6045174 | -15.8805385462954 |
| 31998522.9400131 | -10.7699617666 |
| 31998495.668537 | -9.56515177192135 |
| 31998572.1964841 | -7.72210160065846 |
| 31998709.0126747 | -5.5076602418131 |
| 31998854.9172072 | -3.02568409993224 |
| 31998955.0964149 | -0.438117349875299 |
| 31998972.5940614 | 1.97641059146993 |
| 31998915.6088854 | 3.81198648596055 |
| 31998836.4370833 | 4.62082461581056 |
| 31998818.5529701 | 4.00053031060869 |
| 31998929.4977365 | 1.94411908566648 |
| 31999167.9913954 | -0.933297763052633 |
| 31999468.2504316 | -3.75612624824393 |
| 31999755.1928432 | -5.92457211398546 |
| 31999978.498607 | -7.1340904871819 |
| 32000000 | -7.34374889349892 |
| 32000000 | -6.68209674114327 |
| 32000000 | -5.33785424791469 |
| 31999884.1368775 | -4.406642077214 |
| 29157522.049447 | -10.4380647875832 |
| 11402025.8362507 | -18.1469497366816 |
| 4820956.17181781 | -28.9876063988851 |
| 7447138.13034996 | -10.3763344008256 |
| 17248967.344181 | -1.48823387449173 |
| 30203328.2756753 | 0.855236257077181 |
| 29538446.45446 | 2.75831181291439 |
| 29012146.284714 | 3.8215885651521 |
| 20984193.9051196 | 6.02841081058306 |
| 12979701.5786465 | 10.6079201104689 |
| 3815991.27673281 | 138.79177120636 |
| 22854855.2208849 | 173.762861935397 |
| 31490247.215933 | 176.971638192854 |
| 31398992.9702682 | 176.975701968302 |
| 31355632.5527953 | 176.623597263495 |
| 31382764.2484023 | 176.511700481351 |

| | |
|---|---|
| 31475601.6910368 | 177.245911801552 |
| 31627257.5646609 | 179.177530710625 |
| 24291501.4677251 | -177.794003038556 |
| 17451071.0714988 | -171.586794854815 |
| 12557298.5020421 | -159.791668135737 |
| 10436008.0096581 | -143.617762983351 |
| 13738575.8065195 | -33.6933514686793 |
| 31452327.8126844 | -13.3373490566844 |
| 31685851.3886163 | -11.8105694929037 |
| 31936136.7654985 | -8.87412826600385 |
| 31999754.7758779 | -4.3261920997581 |
| 31999981.332448 | 1.44447800407136 |
| 32000000 | 7.76671765906183 |
| 32000000 | 13.8474920158335 |
| 32000000 | 18.9871497634306 |
| 32000000 | 22.709459180798 |
| 32000000 | 24.7716371680998 |
| 32000000 | 25.1029065302376 |
| 32000000 | 23.7449362534455 |
| 32000000 | 20.8612271848624 |
| 31551318.0281867 | 16.6522411208876 |
| 31084245.0211923 | 11.6490324150921 |
| 31053428.1313189 | 7.05454359559064 |
| 31273012.3094514 | 3.99647831863341 |
| 27055337.6090813 | 2.67623523588946 |
| 26257470.326562 | 2.47510872946733 |
| 27178033.4706491 | 3.38292703309025 |
| 24191634.2762617 | 5.86003837870122 |
| 21984628.5347614 | 9.11092411070952 |
| 20718664.0914006 | 11.6844895417331 |
| 20545521.8551368 | 11.9383807743348 |
| 21922716.9002821 | 8.99110384255432 |
| 25544849.930855 | 3.78381653272668 |
| 28776156.2676429 | -1.64537149998222 |
| 30766251.6598527 | -5.96583657707339 |
| 32000000 | -8.19973602179766 |
| 32000000 | -8.58092864336476 |
| 32000000 | -7.87402496373684 |
| 32000000 | -6.74826380916209 |
| 32000000 | -5.61009712128133 |
| 32000000 | -4.68123916502657 |
| 32000000 | -4.13250745448968 |
| 32000000 | -4.19795836305542 |
| 32000000 | -5.32210067987877 |
| 31999851.5916473 | -8.46022497518271 |
| 31415182.0075474 | -15.7332615851709 |
| 25370379.6151417 | -31.4048239400988 |
| 15524994.7230046 | -80.2007766526758 |
| 32000000 | -150.924072715007 |
| 32000000 | -161.759382717463 |
| 32000000 | -163.36279413465 |
| 32000000 | -163.935315387876 |
| 32000000 | -165.885335498871 |
| 31980561.1617445 | -170.048701779146 |
| 15759723.7473007 | -175.235655657816 |
| 3851556.40687853 | 48.4223415767284 |
| 15764145.711981 | 23.0823711803171 |
| 20575847.7144465 | 24.2502709467666 |
| 18304682.1335421 | 32.0946915481187 |
| 11994299.5714254 | 58.3047309703684 |
| 10794868.6039693 | 111.244905163604 |
| 14411736.0019801 | 140.087734745781 |
| 17177612.9302666 | 153.426550011741 |
| 20182941.8720141 | 164.154722514175 |
| 21843039.2458262 | 171.936399924337 |
| 11898276.5489181 | 1.86725641815407 |
| 25719227.77974 | -5.74589208582619 |
| 25474023.2608107 | -10.8711871357689 |
| 25852544.4528647 | -12.8237913484347 |
| 26202634.2858269 | -11.8904524306298 |
| 26883157.2856942 | -9.07385348372353 |
| 27140980.0439161 | -6.44552872461019 |
| 23289809.9695389 | -3.89863236655632 |
| 20101390.1711842 | -1.96419913851003 |
| 19996424.5318019 | -1.68554968878959 |
| 25376730.0646685 | -2.89540027155594 |

| | |
|---|---|
| 31998978.6615024 | -3.88403344880627 |
| 32000000 | -5.55617656348147 |
| 32000000 | -6.93993209580786 |
| 32000000 | -7.57352525642177 |
| 32000000 | -7.45676065535326 |
| 32000000 | -6.68283162115508 |
| 32000000 | -5.35180386361034 |
| 31942041.9773394 | -3.58320855527151 |
| 31056343.9259721 | -1.52174085722465 |
| 25829615.3461606 | 0.81143024948272 |
| 10038361.5334228 | 5.49838584466697 |
| 2479791.73621284 | 163.348474931191 |
| 10793790.7087906 | -179.152298735836 |
| 12940641.0748702 | -174.193804496023 |
| 9116215.4291104 | -165.247699328629 |
| 2819318.06132853 | -93.0079393826098 |
| 11543750.0389391 | -12.5521463768613 |
| 23495025.9683321 | -3.03908947120092 |
| 31999354.5153445 | 1.36975267150735 |
| 32000000 | 5.58198697108021 |
| 26692722.184809 | 15.4318091395606 |
| 24587924.5464085 | 24.3007852081242 |
| 19015060.1032958 | 42.2322867608184 |
| 14818413.7208691 | 81.8934637837033 |
| 19461993.9235626 | 127.788451355368 |
| 24324617.5070757 | 145.084694090721 |
| 25291704.8750844 | 152.679786457856 |
| 25923280.8105738 | 159.99377763461 |
| 25932125.3597262 | 165.481111057776 |
| 24948310.7173175 | 169.113944453839 |
| 22784836.5545846 | 171.163338624235 |
| 17726534.6846479 | 172.556454881076 |
| 4011947.55929255 | 168.299551218176 |
| 25491578.2572307 | 1.67731839465631 |
| 32000000 | 2.6510105290456 |
| 32000000 | 7.57524114370505 |
| 32000000 | 10.2588563945376 |
| 32000000 | 11.4072216452856 |
| 32000000 | 11.3800521879684 |
| 32000000 | 10.368987731425 |
| 32000000 | 8.49163611222377 |
| 31680654.027477 | 5.8902801614417 |
| 30748996.2567283 | 2.8238230603822 |
| 30209978.9234526 | -0.290359566619977 |
| 30155864.1080654 | -2.85551182118434 |
| 30605289.1311696 | -4.26198361212307 |
| 31492076.6559935 | -4.09471589078142 |
| 31999778.1235954 | -2.26372105978353 |
| 31999971.3833912 | 1.01652414520195 |
| 32000000 | 5.26908930048531 |
| 32000000 | 9.88827633141267 |
| 32000000 | 17.6019072573721 |
| 14813134.9493294 | 53.8057358864077 |
| 12818520.012016 | 114.394489443414 |
| 16316998.1642022 | 138.220156111818 |
| 16969324.0018873 | 144.160274536983 |
| 14790111.6168464 | 141.227432912596 |
| 11051124.947755 | 123.899465518686 |
| 10219321.831777 | 74.0984420013625 |
| 10592475.1420037 | 99.9481797982297 |
| 11388347.9917885 | 116.796848788858 |
| 10107113.5525817 | 115.457995889949 |
| 7494678.99727381 | 97.6325318611396 |
| 8275297.83731342 | 40.1116520204979 |
| 17617885.1584019 | 10.3184042478437 |
| 30748749.6066132 | 2.28471417470028 |
| 31999694.4081901 | -0.0452460234115585 |
| 31999515.8139013 | -1.52037684060058 |
| 31999299.6960043 | -2.35709619583576 |
| 31999089.9070684 | -2.84492202241123 |
| 31998935.4248271 | -2.89256258911246 |
| 31980031.0457073 | -2.1219373675077 |
| 31258339.0853076 | -0.256860286809413 |
| 24997084.5835221 | 2.54389244689479 |
| 1675027.02094489 | 47.719685667406 |
| 25514209.5502747 | 178.682123483396 |

| | |
|---|---|
| 31999599.207035 | -177.395184745872 |
| 31997118.5657908 | -176.222201087145 |
| 30863145.1046998 | -176.202510772933 |
| 28031503.3809938 | -176.708909495246 |
| 25339859.5353028 | -177.922908627731 |
| 23538438.4105135 | 179.492306036386 |
| 7780910.74827648 | 173.955953325912 |
| 6294008.76700734 | 14.6119451045854 |
| 15270926.6851667 | 8.67964905638308 |
| 16285283.4870607 | 9.80433032105625 |
| 6310487.88192393 | 26.6727434788838 |
| 19136035.1374316 | 172.917324671033 |
| 31720686.0249046 | 178.743608387905 |
| 31774574.872384 | -178.451207228847 |
| 31827429.5597019 | -175.77670563011 |
| 31894733.4424703 | -173.874284074966 |
| 31959072.2290771 | -173.27734009981 |
| 31427604.5056893 | -174.275367157652 |
| 29462860.7178968 | -177.054856993134 |
| 27438522.3827547 | 178.323966492664 |
| 25256107.9099836 | 172.402656969285 |
| 23905571.2605898 | 167.290170753962 |
| 19613701.2179837 | 19.0220042440609 |
| 32000000 | 12.1887546220024 |
| 32000000 | 11.2562109898545 |
| 31999677.7923603 | 9.70001919873276 |
| 31999309.5932995 | 6.2657929491393 |
| 31999031.0559142 | 1.53957040905728 |
| 31998875.145379 | -3.67132510805032 |
| 31984157.8005577 | -8.42801534097897 |
| 31934840.5002088 | -13.0133447285105 |
| 31874710.8789511 | -15.0758084006319 |
| 31809906.0014925 | -13.0447542298496 |
| 31765755.5309751 | -8.81558421505961 |
| 31779521.7150916 | -4.68771746768914 |
| 31849016.169881 | -0.570181922506336 |
| 31949983.490768 | 3.05800889843641 |
| 32000000 | 5.83473814097578 |
| 32000000 | 8.02419698655168 |
| 32000000 | 10.5513924712787 |
| 20843373.3383361 | 15.9285121720642 |
| 9975397.32725132 | 26.5918337119234 |
| 3728147.56137983 | 49.6031512169995 |
| 1277151.65050416 | 61.917788966713 |
| 3468950.44226425 | -174.655792524989 |
| 3292266.54454579 | -157.143985822009 |
| 2196106.10520235 | -46.5738356762564 |
| 3847663.8461525 | -162.366931111679 |
| 26633132.6781344 | -179.977975340972 |
| 25999416.7355307 | 177.217371125089 |
| 21892732.3098692 | 173.900547121452 |
| 20213475.9720154 | 170.847062296271 |
| 18748187.2593482 | 168.640455872507 |
| 18914514.3046026 | 169.100943971792 |
| 21168897.5683735 | 172.406530068944 |
| 23651259.4226143 | 176.364421275026 |
| 27621363.3989904 | -179.986731697286 |
| 22694494.9725406 | -176.58151768233 |
| 16746250.1880282 | -172.91910730309 |
| 11989717.2528221 | -171.180949287343 |
| 5449629.4793478 | -174.219430730648 |
| 6738019.57057183 | 15.2693429882558 |
| 25737309.1299687 | 11.05000044194 |
| 32000000 | 11.0411098556547 |
| 32000000 | 10.6453667759525 |
| 32000000 | 9.68470278107132 |
| 32000000 | 8.42836529710901 |
| 32000000 | 7.20494175976322 |
| 32000000 | 6.13053554711818 |
| 32000000 | 5.19751333760354 |
| 32000000 | 4.32742331739951 |
| 32000000 | 3.34945301748871 |
| 32000000 | 1.93254741954704 |
| 32000000 | -0.136361034024851 |
| 24227072.2163551 | -4.98927905669497 |
| 3009232.60581223 | -79.5286650937037 |

| | |
|---|---|
| 12938795.1194785 | -168.0936710615 |
| 14018106.4361115 | -172.241446737923 |
| 4681308.77793017 | -163.892995675825 |
| 9387251.59166406 | -7.83380863232479 |
| 16806299.2228222 | -5.40760831294852 |
| 25532218.7589217 | -3.83672126291822 |
| 30873399.8320648 | -3.31404937047777 |
| 32000000 | -3.12006769564198 |
| 32000000 | -3.23407240939765 |
| 32000000 | -3.35859756725667 |
| 32000000 | -3.42405667883587 |
| 32000000 | -3.49295911897059 |
| 32000000 | -3.87182080165989 |
| 32000000 | -4.56846914628005 |
| 32000000 | -5.33709143103601 |
| 32000000 | -6.44350855415013 |
| 32000000 | -8.09862629392813 |
| 32000000 | -9.83341482007077 |
| 32000000 | -11.2935613186248 |
| 32000000 | -12.2829297943945 |
| 32000000 | -12.7354309834026 |
| 32000000 | -12.6990875427227 |
| 32000000 | -12.2833669822322 |
| 32000000 | -11.6146703075337 |
| 32000000 | -10.7791531043146 |
| 31889415.3857353 | -9.66570959642913 |
| 21937803.2667336 | -16.2733990345445 |
| 27834898.5880394 | -168.662023730373 |
| 29757422.1977245 | -168.149541353121 |
| 30614613.2800988 | -167.014839486678 |
| 30357955.1040711 | -165.506991237854 |
| 29091636.0420726 | -163.808110370151 |
| 27079510.2175457 | -162.08429904929 |
| 19974214.8399748 | -157.13888170384 |
| 6614724.1706507 | -114.076111179646 |
| 26600207.9851267 | -8.20465719093758 |
| 31999052.8971492 | -1.27698558925731 |
| 31998971.7803885 | 3.03844699991982 |
| 31998938.7063426 | 6.38777869639217 |
| 31998950.5247821 | 8.70449733901183 |
| 31798841.7782749 | 12.4893898087031 |
| 15489522.3894562 | 31.0500804099185 |
| 10143353.6296135 | 117.704230519343 |
| 23254895.0186458 | 155.264547497396 |
| 29561100.2053077 | 160.573366311936 |
| 25830658.8288198 | 159.634247367383 |
| 21021424.4035965 | 158.568664976802 |
| 14906317.7165393 | 155.530390329654 |
| 5308804.51011702 | 66.7186420245524 |
| 10519572.105662 | 22.4145171398726 |
| 15538581.5771966 | 12.9955569530933 |
| 20085462.3043813 | 9.18176916034363 |
| 22976161.1487021 | 7.36114153818535 |
| 23178914.6484319 | 6.12273679371947 |
| 20413089.8065337 | 4.5315859091438 |
| 15498542.2579479 | 1.14694423196771 |
| 10399178.4921694 | -7.66144733929165 |
| 7351927.24361501 | -27.2282440312639 |
| 8109116.43380714 | -42.3047931047449 |
| 12340970.7201037 | -37.0842895601845 |
| 14996732.5590803 | -36.9870024265066 |
| 19951923.5920196 | -30.0901078873965 |
| 28713304.5377401 | -20.6584699928173 |
| 31999987.5816124 | -14.89673334559 |
| 31999415.8163575 | -12.8024615428977 |
| 31998716.4826502 | -9.20083449924412 |
| 31998074.0038475 | -4.27284919647169 |
| 31997584.2297481 | 0.94320081471628 |
| 31997306.7622802 | 5.59305554879817 |
| 31997267.8800844 | 8.81327190710388 |
| 31997469.7382581 | 10.1293206373229 |
| 25218822.6796167 | 11.2160647890757 |
| 18601797.3318019 | 8.2178463437696 |
| 18394375.825131 | 0.353989654208687 |
| 24508693.4027082 | -4.77217173985827 |
| 23322124.7153634 | -8.25676142415701 |

| | |
|---|---|
| 14806251.0359332 | -15.0097895318024 |
| 16899718.5433257 | -11.6855773974282 |
| 13954853.9461831 | -8.17801893985039 |
| 4318949.29063054 | 0.846796206498803 |
| 12664858.503436 | 170.152194530718 |
| 27301858.4095455 | 171.882956690217 |
| 32000000 | 171.551023027038 |
| 32000000 | 171.899004205733 |
| 32000000 | 172.120664101427 |
| 32000000 | 172.241231255522 |
| 32000000 | 172.176720666439 |
| 31999920.2217631 | 172.010834439032 |
| 31999331.3722052 | 171.308504284278 |
| 10018139.6214237 | 31.4631102342234 |
| 29248075.8588626 | 14.2495046562966 |
| 32000000 | 15.9160853017491 |
| 32000000 | 16.7858421309994 |
| 32000000 | 16.7548404964641 |
| 32000000 | 15.6521684060182 |
| 32000000 | 13.6899801796608 |
| 32000000 | 11.1009429607121 |
| 32000000 | 8.13268628007555 |
| 32000000 | 5.06351475364091 |
| 32000000 | 2.22988128379853 |
| 31420492.8596771 | 0.0305890962297433 |
| 28779131.1782637 | -1.23651506380686 |
| 26661421.3013299 | -1.59794759825525 |
| 25260128.3135045 | -1.140191228252 |
| 20343272.8825096 | 1.02571517964501 |
| 2425413.02675684 | 172.662276838766 |
| 14981437.3070668 | 178.362674027308 |
| 18373301.096811 | 177.981153943434 |
| 15701677.1687065 | 176.814085895288 |
| 4196642.94933408 | 165.540754785567 |
| 11867128.9899583 | 5.56584121917404 |
| 29928578.9302517 | 2.32073082230218 |
| 31999716.5813672 | 2.04241020312366 |
| 31999412.8164202 | 2.36945377598659 |
| 31999132.8537622 | 2.8581776486453 |
| 31998929.026597 | 3.33403045737106 |
| 31998841.474222 | 3.6339634470793 |
| 31957531.7000251 | 4.3207310017899 |
| 14507067.4265645 | 9.84402106461985 |
| 7159224.81780016 | 158.942422834344 |
| 23003080.0804856 | 173.436075613225 |
| 30277973.6206358 | 175.317584829169 |
| 30016050.4257241 | 176.328141705238 |
| 17585353.3779868 | 176.153798193665 |
| 4600424.04518312 | 174.428896586958 |
| 6084080.82304494 | -0.0459413769671048 |
| 16451876.5855694 | 0.0468469571000285 |
| 26668488.4639183 | 1.25370246188311 |
| 27675346.5941252 | 3.71254617237072 |
| 27726843.2243396 | 5.38908659202304 |
| 26265806.6544138 | 6.77521710970097 |
| 20891808.9564737 | 8.82349618879868 |
| 17936133.6302965 | 171.356742319164 |
| 32000000 | 179.314938443895 |
| 32000000 | -178.152236783899 |
| 32000000 | -175.715306772613 |
| 32000000 | -173.585393709465 |
| 32000000 | -171.851866369153 |
| 32000000 | -170.620825650082 |
| 32000000 | -170.057517341036 |
| 32000000 | -170.37428904789 |
| 32000000 | -172.04296615076 |
| 32000000 | -173.788405023061 |
| 24586457.7664709 | -176.92954967767 |
| 32000000 | 178.230315086598 |
| 32000000 | 175.518624807223 |
| 32000000 | 173.216921987061 |
| 31966831.5515823 | 172.208304989521 |
| 31911558.921924 | 172.70591326424 |
| 30782413.1321307 | 174.573761145715 |
| 29114617.3159958 | 177.741269725553 |
| 27761321.5469939 | -178.180029143228 |

| | |
|---|---|
| 26991024.4786773 | -173.513997272093 |
| 19352027.6720874 | -161.946354940292 |
| 17513931.7025349 | -23.6353601208249 |
| 30847239.1234554 | -14.1499739697289 |
| 30553015.2270629 | -14.2354455489022 |
| 30440258.6291603 | -13.929460488024 |
| 30468253.0709499 | -12.961808644448 |
| 30659336.1576472 | -11.3613548949741 |
| 30993883.7197144 | -9.36108066326237 |
| 31282516.3767023 | -7.2290391457387 |
| 31578223.637458 | -5.21010443660857 |
| 31860960.1914796 | -3.39658702951907 |
| 31975963.4976328 | -1.77094965141926 |
| 31999531.2043288 | -0.222679529250715 |
| 28154514.4658599 | 1.68170506825032 |
| 19648045.1770845 | 5.03226478314341 |
| 10731238.9101216 | 13.3930459420539 |
| 3381714.42496665 | 64.28273767986 |
| 6833890.80682911 | 150.890008222497 |
| 10805044.3583222 | 162.432699689845 |
| 10700891.9040249 | 164.518703396446 |
| 6115523.54016107 | 159.276068978184 |
| 2417651.14006752 | 31.1042997773311 |
| 1235052.88811546 | 2.14183534889358 |
| 1674168.10375726 | -61.9161496893638 |
| 3216620.60064213 | -98.4892427916328 |
| 6234351.09229033 | -127.394040416483 |
| 22033112.2595962 | -161.888650530696 |
| 27109619.01005 | -162.589077241388 |
| 28227246.2239794 | -160.718771154372 |
| 30692217.8100228 | -161.060234052031 |
| 31508814.730368 | -162.125967321294 |
| 31999551.7195839 | -164.025126358433 |
| 31999749.405208 | -166.354483974879 |
| 31999896.0136346 | -168.820703387907 |
| 31999945.4854916 | -171.257160230194 |
| 31999870.002486 | -173.578827685036 |
| 31999661.3627773 | -175.607978334206 |
| 31994006.753394 | -177.184730060871 |
| 19271617.6044337 | -175.407826029489 |
| 5483007.7761387 | -154.275020088233 |
| 4964481.04179239 | -48.4657833593119 |
| 7052661.5008552 | -44.5157897604404 |
| 10955564.2470803 | -32.0692850495989 |
| 11716155.6407409 | -32.214697524014 |
| 10162023.0744113 | -35.9838778914841 |
| 9424731.98510236 | -31.7964187140392 |
| 10346787.9426957 | -18.9059599825106 |
| 12479324.5844831 | -5.76157099108283 |
| 11902971.7475668 | 6.38500753133068 |
| 13366114.6314265 | 18.5885814167885 |
| 16458708.0727466 | 25.9831513104476 |
| 20778815.8141752 | 27.986388198844 |
| 26304921.6904032 | 25.7273861973008 |
| 31999015.2071121 | 20.6886523217334 |
| 31999432.944342 | 16.0365722337714 |
| 31999886.1090811 | 10.9733293034736 |
| 32000000 | 6.28727512200322 |
| 32000000 | 1.17837491254581 |
| 32000000 | -4.25987184534715 |
| 32000000 | -9.41649559193175 |
| 32000000 | -13.7536944051682 |
| 32000000 | -16.768897638753 |
| 32000000 | -18.1131789040386 |
| 32000000 | -17.68757609679 |
| 30837871.3860004 | -15.3439172308967 |
| 28974596.2588418 | -11.2556154186372 |
| 27844115.9873576 | -6.01541996117729 |
| 17820928.7355605 | -0.730822922581663 |
| 9330769.576017 | 11.8237879742473 |
| 25204541.8585736 | 172.594130044885 |
| 30684778.2846055 | 173.042476065658 |
| 28581852.9958105 | 173.599519759291 |
| 26301544.6668568 | 176.198332805424 |
| 23638690.8062674 | -179.222188546554 |
| 20124236.2396073 | -172.358171621328 |

| | |
|---|---|
| 14480910.4227895 | -160.537936779845 |
| 10410450.407147 | -141.472938183665 |
| 8453930.18191207 | -118.748462577389 |
| 7647479.57634897 | -102.670887776755 |
| 6649016.88690623 | -97.4973094895559 |
| 5031433.68886812 | -104.197972731493 |
| 3332715.34428139 | -131.43388221432 |
| 3197228.66998882 | 174.962988501551 |
| 4851138.69612326 | 139.532153153307 |
| 6746688.5455142 | 120.895275459116 |
| 8320980.16603248 | 107.655156455326 |
| 9441160.0144798 | 96.9843950970664 |
| 10018279.2816984 | 88.8519054467397 |
| 9910669.45737496 | 84.2064959450145 |
| 9009492.70192537 | 84.8693295386 |
| 7502288.66340763 | 94.8207843193678 |
| 6410047.20887989 | 120.763416634673 |
| 7535019.80324231 | 154.777515280913 |
| 10704586.7310262 | 176.188792781036 |
| 14304051.3864359 | -172.455408561703 |
| 17234919.9573995 | -165.026511384451 |
| 18920275.3422866 | -158.596639945314 |
| 19226165.6244019 | -151.700107669665 |
| 18439250.8841722 | -143.52722222505 |
| 17143045.8901666 | -134.017125815724 |
| 15922865.1932608 | -124.492785619176 |
| 15033302.4492076 | -117.877849346846 |
| 14440213.8278609 | -117.555488070756 |
| 14363527.4403119 | -125.604780750262 |
| 15608414.7916938 | -140.327646425033 |
| 18769133.8321306 | -155.611123240274 |
| 23247257.4770017 | -167.092426285338 |
| 27649377.7220516 | -174.733469045968 |
| 30541781.8545614 | -179.801755568629 |
| 30848193.5539258 | 176.697290286811 |
| 28072759.9941529 | 174.119580380617 |
| 22395946.9535828 | 172.005740955327 |
| 14605066.0221316 | 169.868770979276 |
| 5885525.59610459 | 166.143321307438 |
| 2511546.36071554 | -3.64152361492612 |
| 9321668.04358634 | -11.9460563989065 |
| 13806244.3528142 | -15.5129569101304 |
| 15612333.8885303 | -19.6194722116934 |
| 14915073.2688158 | -25.3335066678632 |
| 12350136.7785043 | -34.2133124483114 |
| 8924416.8146375 | -49.7719789828198 |
| 6047259.23194594 | -79.7918247529338 |
| 5357962.21173706 | -124.53765231527 |
| 6444349.43102804 | -158.571124104629 |
| 7579861.08754854 | -179.907438719831 |
| 8209925.87271573 | 163.559685455332 |
| 8432264.16478333 | 148.895159010915 |
| 8415649.81964853 | 136.191584547902 |
| 8164312.16206251 | 126.690497733375 |
| 7555371.26777528 | 121.62921067056 |
| 6514673.37846913 | 122.289461697219 |
| 5174871.39346611 | 131.200520724718 |
| 4012307.38702124 | 153.368670547729 |
| 3819587.97367574 | -172.195159430701 |
| 4692399.60110715 | -143.690863485338 |
| 5833403.50767129 | -126.068821034145 |
| 6683898.76154718 | -113.979480941736 |
| 7015934.62237585 | -104.19556517111 |
| 6762468.8302152 | -95.3623995151345 |
| 5935606.78866604 | -86.8603122249616 |
| 4596002.39836001 | -78.084563353817 |
| 2854977.90776312 | -67.0354078789327 |
| 975024.355748348 | -34.4992170893126 |
| 1492024.11429471 | 85.5791543628903 |
| 3350948.454076 | 103.205975024864 |
| 4861604.62141818 | 109.34593552484 |
| 5781390.76224644 | 112.479290945098 |
| 6001435.80124151 | 113.896674888668 |
| 5543351.35423722 | 113.968873429939 |
| 4557860.42619507 | 112.930132836501 |
| 3290156.06493 | 111.429981628357 |

| | |
|---|---|
| 2020478.09335147 | 112.33800992273 |
| 1059376.25847481 | 129.130441074711 |
| 981512.929806543 | 174.676166789734 |
| 1600400.43539063 | -172.189183004888 |
| 2185087.35602741 | -177.887136325828 |
| 2335421.53569121 | 169.211488183382 |
| 2369764.89077231 | 156.963390602569 |
| 2837562.30664598 | 154.048037048054 |
| 3256656.56073906 | 150.779137340282 |
| 3533441.13683247 | 146.977436146875 |
| 3589439.65640159 | 142.087699263363 |
| 3386102.51898886 | 135.029647467067 |
| 2957797.17892784 | 123.66270479281 |
| 2470199.45844713 | 104.019382931606 |
| 2286016.59048546 | 73.6590063835323 |
| 2700384.49805566 | 43.5201989742379 |
| 3489559.38394087 | 23.8320675736895 |
| 4273462.47041654 | 11.7374209982236 |
| 4798801.85274606 | 3.22162546035373 |
| 4922927.45680249 | -4.07187571328659 |
| 4595031.0882795 | -11.8398053174346 |
| 3861478.87196979 | -22.2209392360983 |
| 2901422.76967602 | -39.6694708782814 |
| 2163729.9351859 | -73.3373224683598 |
| 2350527.96000072 | -117.344847151325 |
| 3265788.22161476 | -144.865414334605 |
| 4228893.13138799 | -159.915536581614 |
| 4913213.41141308 | -170.199619489592 |
| 5198515.27620308 | -179.037202398949 |
| 5077519.93307756 | 171.875365232814 |
| 4627442.65077374 | 161.239561746588 |
| 3991204.49566689 | 147.702839654461 |
| 3351959.09168599 | 129.948411954547 |
| 2881011.22619355 | 107.828421175589 |
| 2643027.74330005 | 83.9081413349127 |
| 2546532.09267757 | 61.6811720891133 |
| 2446427.12827688 | 42.0386702827399 |
| 2263014.1319932 | 23.5551929224439 |
| 2002752.08283858 | 4.22838085198648 |
| 1723740.05868327 | -17.5562925634503 |
| 1484994.5052313 | -42.2941569181656 |
| 1303530.97177853 | -69.3640520752679 |
| 1165681.33507381 | -98.9165482165325 |
| 1100936.27516351 | -132.624951323961 |
| 1210970.58400519 | -167.851685810538 |
| 1530561.74609135 | 164.081006064711 |
| 1950778.1399005 | 145.692182850778 |
| 2327944.49652874 | 134.228954466064 |
| 2545875.83208253 | 127.280616105987 |
| 2528973.30239676 | 123.678004235661 |
| 2249660.4229647 | 123.355005395649 |
| 1737428.22803961 | 127.985777577026 |
| 1112855.48426557 | 145.108340389429 |
| 803907.287689042 | -163.55246765115 |
| 1287244.43058028 | -119.859661327619 |
| 1992682.92313064 | -105.016628189231 |
| 2594814.75901792 | -98.6765887464792 |
| 2991818.38639789 | -95.0464701663955 |
| 3151221.66765474 | -92.3969192415268 |
| 3084464.54390279 | -90.0062692497809 |
| 2835786.14254082 | -87.4269083232708 |
| 2470713.65607507 | -84.2203303686416 |
| 2063878.64139949 | -79.8006173229393 |
| 1688271.4871904 | -73.3643854717562 |
| 1407132.72546895 | -64.17749295614 |
| 1265096.88806305 | -52.6571751943111 |
| 1274618.65984796 | -41.1802235052769 |
| 1413305.29154335 | -32.1078905152266 |
| 1643740.52323065 | -25.683675474273 |
| 1929123.18136162 | -20.9145778702098 |
| 2234185.11707761 | -16.8849402671612 |
| 2522929.90821361 | -13.0982041519029 |
| 2758314.75381082 | -9.35976777615062 |
| 2903788.2246533 | -5.60924257477854 |
| 2926442.06720377 | -1.79579700054867 |
| 2801665.71739413 | 2.22195532453474 |

| | |
|---|---|
| 2518875.99578073 | 6.81167832041978 |
| 2088172.49519284 | 12.8893848989141 |
| 1551303.0085135 | 22.9647964016862 |
| 1021113.19263212 | 44.9378792161413 |
| 824653.823560524 | 91.6621561404444 |
| 1190822.70484372 | 128.857800319593 |
| 1729898.89832656 | 143.017264076833 |
| 2205785.92226166 | 148.021137121097 |
| 2534012.87854826 | 149.012001574177 |
| 2680843.44789271 | 147.61677516718 |
| 2643261.07513628 | 144.336687390069 |
| 2443904.81271318 | 139.155936625095 |
| 2127845.75732034 | 131.667587004734 |
| 1758691.16266059 | 121.077026388688 |
| 1411242.34725777 | 106.456605470071 |
| 1150920.03055543 | 88.0944234258926 |
| 990189.645679287 | 69.6571540870342 |
| 867154.354522638 | 56.9372235875226 |
| 709824.076539333 | 55.3892017020227 |
| 550129.412132931 | 75.2942541662511 |
| 652737.796405204 | 115.926671639149 |
| 1105980.54779774 | 137.558773176073 |
| 1696497.24869149 | 144.423332974759 |
| 2280647.24162572 | 146.21130008483 |
| 2754365.66956488 | 146.048045465314 |
| 3033334.92243199 | 144.944929924724 |
| 3058536.70634877 | 143.191560980722 |
| 2805187.12825683 | 140.6864737716 |
| 2289528.90537325 | 136.817463392563 |
| 1574251.08432361 | 129.433445502045 |
| 799836.323054611 | 107.595143865781 |
| 571724.935384139 | 27.2338013529039 |
| 1170936.36844069 | -10.9353235429038 |
| 1709364.90745392 | -21.4592187461269 |
| 1977027.33747176 | -26.915215580958 |
| 1909434.32485825 | -31.4407352871131 |
| 1503143.66379792 | -37.5694122404037 |
| 829434.005492934 | -53.7048290126043 |
| 488705.069557699 | -144.227150921659 |
| 1382369.0219172 | 172.437290687225 |
| 2414259.94159228 | 163.761405431563 |
| 3328402.73101244 | 160.093745969502 |
| 4004556.05661835 | 157.975711318493 |
| 4362992.18477427 | 156.53150221492 |
| 4364928.30211659 | 155.454769135112 |
| 4013579.17620099 | 154.655089883385 |
| 3350582.28403784 | 154.214447436094 |
| 2448237.23921534 | 154.570965335184 |
| 1401041.06336212 | 157.752156775346 |
| 370312.285604451 | -169.829713235575 |
| 855694.748168459 | -53.9267461903113 |
| 1800831.69289595 | -46.2879196757694 |
| 2593243.43293922 | -45.5172234066131 |
| 3184569.48467079 | -46.1392327591006 |
| 3556749.82918722 | -47.1172696464794 |
| 3710217.98750139 | -48.0052861984144 |
| 3659763.90583962 | -48.4810494684076 |
| 3431857.1332906 | -48.2292439343076 |
| 3062870.82169287 | -46.8837625772504 |
| 2597482.61364562 | -43.9646147746721 |
| 2086367.23806388 | -38.7743154518471 |
| 1582657.35914162 | -30.2117328105503 |
| 1137528.78393464 | -16.4599947660501 |
| 796368.403785452 | 5.27961606565246 |
| 595538.879444727 | 37.3683262781623 |
| 548217.611174643 | 75.5905010192613 |
| 625281.292589041 | 109.356641406135 |
| 783045.81422723 | 133.889754999229 |
| 986413.90041051 | 149.986962076082 |
| 1203830.26669918 | 159.442823538332 |
| 1410512.41398382 | 163.708283156871 |
| 1597549.70249897 | 163.81300050695 |
| 1776352.33982887 | 160.679785620641 |
| 1971858.76830571 | 155.493023735556 |
| 2203907.22322192 | 149.743966534724 |
| 2468305.43757214 | 144.799400185153 |

```
2732800.35807316    141.455483829668
2948285.76499724    139.923682467706
3063950.12947148    140.092302096423
3038685.3394663     141.763707630732
2847586.9221246     144.791925185298
2484866.99484974    149.188466984901
1964890.57517241    155.348563256629
1324194.59502208    164.992217356916
643909.963670429    -171.860302962099
431578.651462513    -78.2221870796764
1023098.99316118    -36.3801422296181
1607890.6237913     -22.8115350298508
2033065.56720724    -13.6013405558328
2242233.49726651    -5.18373463553497
2214894.39713101    3.92884663349289
1971996.76993342    15.374644132581
1591811.99856932    32.2239030568788
1245711.44373199    59.9942728126213
1192504.0963227     97.8775916601315
1456344.3187575     127.900898336166
1770057.32669417    145.596176272676
1938199.81732851    156.512439685239
1877667.09015722    163.998034314995
1577879.262364      169.400900266297
1082152.46913867    172.666513261806
477705.82351482     168.677677380709
223011.09057221     49.2015907624186
740474.20638728     28.422397892512
1133064.82958764    32.8049315495323
1346137.37518465    42.4296818104869
1412919.42152713    56.969142005963
1433079.09981215    76.7194466724545
1520340.22361327    99.0548462105081
1694945.11342374    118.917973581815
1861952.54361036    133.976130880967
1901882.61322738    145.108750544525
1736873.79824254    154.009642624325
1349616.14237757    162.591232825634
786536.356569125    175.297054615413
251443.835761755    -123.285283983017
656523.856344497    -35.5226940406503
1190731.20846891    -20.7976654944177
1532041.24691341    -12.172261531556
1628094.70507741    -3.09463604828416
1508869.65480654    9.92141473950373
1311918.5163645     31.3373204730259
1283654.99105322    61.481635675682
1538608.88222997    87.2855806832295
1886680.79602152    101.881549002555
2110578.67045048    108.881323239139
2087653.47490888    111.52359201388
1776637.71391095    111.366594308378
1200750.30862176    109.087975691591
429828.386762025    105.110699688313
```

We assume a response function digitised with 0.5 ns time resolution which is defined in the `Rsp.dat` file (main text Figure 6A):

```
2.6577900e-01  0.0000000e+00
2.3063150e-01  2.4570450e-03
1.9548400e-01  4.9140900e-03
1.6958700e-01  6.0714200e-03
1.4369000e-01  7.2287500e-03
1.2462150e-01  7.6011700e-03
1.0555300e-01  7.9735900e-03
9.1520400e-02  7.8949350e-03
7.7487800e-02  7.8162800e-03
6.7168300e-02  7.4989800e-03
5.6848800e-02  7.1816800e-03
4.9264550e-02  6.7575000e-03
4.1680300e-02  6.3333200e-03
3.6109800e-02  5.8811000e-03
3.0539300e-02  5.4288800e-03
2.6450500e-02  4.9932750e-03
```

```
2.2361700e-02  4.5576700e-03
1.9362400e-02  4.1616750e-03
1.6363100e-02  3.7656800e-03
1.4164350e-02  3.4189650e-03
1.1965600e-02  3.0722500e-03
1.0354835e-02  2.7765850e-03
8.7440700e-03  2.4809200e-03
7.5647900e-03  2.2336700e-03
6.3855100e-03  1.9864200e-03
5.5227050e-03  1.7827600e-03
4.6599000e-03  1.5791000e-03
4.0290600e-03  1.4133550e-03
3.3982200e-03  1.2476100e-03
2.9372950e-03  1.1140370e-03
2.4763700e-03  9.8046400e-04
2.1398200e-03  8.7369750e-04
1.8032700e-03  7.6693100e-04
1.5577100e-03  6.8218000e-04
1.3121500e-03  5.9742900e-04
1.1331045e-03  5.3055350e-04
9.5405900e-04  4.6367800e-04
8.2360450e-04  4.1117950e-04
6.9315000e-04  3.5868100e-04
5.9816950e-04  3.1765600e-04
```

# 7 Quadrupolar second-order cross-terms

Residual dipolar splitting spectra in the main text Figure 8 are simulated using the input file

```
spinsys {
    channels            1H 14N
    nuclei              1H 14N
    dipole              1 2 -7000 0 0.0 0
    quadrupole          2 2 3.0e6 0.8 0 0 0
    quadrupole_x_dipole 2 1
}

par {
    spin_rate         50000
    method            direct
    sw                20000
    variable tsw      1e6/sw
    proton_frequency  800e6
    np                4096
    crystal_file      zcw986
    gamma_angles      16
    start_operator    I1x
    detect_operator   I1p
}

proc pulseq {} {
    global par

    maxdt [expr 1.0e6/$par(spin_rate)/24.0]
    acq_block {
        delay $par(tsw)
    }
}

proc main {} {
    global par

    set f [fsimpson]
    faddlb $f 15 0
    fzerofill $f 8192
    fft $f
    fsave $f $par(name).spe
    funload $f
}
```

A two-dimensional shifted-echo STMAS experiment with realistic RF pulses is presented in the main text Figure 9

and is calculated using the input file

```
# ideal excitations, shifted echo sequence
# pathway ST+(k*t1) -> CT+(kk*t1+tau) -> CT- (acq)
spinsys {
     nuclei     87Rb
     channels   87Rb
     quadrupole 1 2 4.0e6 0.0  0 0 0
     shift      1 4700 500p 0 0 0 0
}

par {
    proton_frequency  304.47e6
    spin_rate         50000.0
    method            direct
    gamma_angles      16
    crystal_file      zcw376
    start_operator    I1z
    detect_operator   I1c

    sw                spin_rate
    np                512
    ni                256
    variable dt1      1.0e6/spin_rate
    variable k        9.0/17.0
    variable kk       8.0/17.0
    variable tau      np/2.0*1.0e6/sw
    variable tsw      1.0e6/sw
    sw1               spin_rate*17.0/9.0

    variable p1       1.6
    variable p2       1.6
    variable p3       25.0
    verbose           01
}

proc pulseq {} {
    global par

    # this is ST+
    matrix set 1 operator I1p-I1c
    # this is CT+
    matrix set 2 operator I1c
    # CT- is not needed

    maxdt 0.05
    # excite ST+
    reset
    pulse $par(p1) 100000 x
    store 1

    # ST to CT
    reset [expr $par(dt1)+$par(p1)*0.5-$par(p2)*0.5]
    pulse $par(p2) 100000 x
    store 2

    # CT inversion occures at different rotor pases for each t1 increment
    for {set dim1 1} {$dim1 <= $par(ni)} {incr dim1} {
        # first t1 delay (ST+ evolution)  k*t1 = n*dt1 = 1/spin_rate
        set t1a [expr $dim1*$par(dt1)-$par(p1)*0.5-$par(p2)*0.5]
        # second t1 delay (CT+ evolution)
        set t1b [expr $t1a/$par(k)*$par(kk)+$par(tau)]

        reset
        # excitation ST+
        prop 1
        filter 1
        # evolution k*t1
        delay $t1a
        # conversion to CT+
        prop 2
        filter 2
        # second part of evolution kk*t1
        delay $t1b
        # CT inversion
        pulse $par(p3) 10000 x
        # acquire full echo
```

```
        acq_block -np $par(np) {delay $par(tsw)}
    }
}

proc main {} {
    global par

    set f [fsimpson]
    puts "      Calc. time = [expr $par(tcalc)*1e-6] s"

    # save as binary without headers, read in matlab as floats
    fsave $f $par(name)_raw_bin.fid -raw_bin
    funload $f
}
```

Second-order cross-term between the nuclear quadrupole and chemical shift anisotropy interactions can be triggered using the `spinsys` section as follows

```
spinsys {
     nuclei               87Rb
     channels             87Rb
     quadrupole           1 2 4.0e6 0.0 0 0 0
     shift                1 4700 500p 0 0 0 0
     quadrupole_x_shift   1
}
```

while the cross-term between the nuclear quadrupole and its dipole-dipole interaction with another nucleus is triggered in the following `spinsys` definitions, for a spin-1/2 (proton, $^{1}$H) and a spin-3/2 (sodium, $^{23}$Na).

```
spinsys {
     nuclei               87Rb 1H
     channels             87Rb
     quadrupole           1 2 4.0e6 0.0 0 0 0
     dipole               1 2 -10000 0 0 0
     quadrupole_x_dipole 1 2
}

spinsys {
     nuclei               87Rb 23Na
     channels             87Rb
     quadrupole           1 2 4.0e6 0.0 0 0 0
     dipole               1 2 -10000 0 0 0
     quadrupole_x_dipole 1 2
}
```

# 8 Calculation of tm-SPICE pulses

Here, we reproduce the input files and other data used to produce tm-SPICE pulses for magnetization transfer from amide nitrogen to the neighbouring alpha carbon. The original publication is available at `https://doi.org/10.1002/anie.201805002`. For robustness, a minimal set of four nuclei is needed to reflect spin dynamics in fully labelled proteins. It is defined as

```
spinsys {
    # 1: 0 N N 2 A {} 19
    # 2: 0 C CA 2 A {} 20
    # 3: 0 C C 2 A {} 21
    # 4: 0 C CB 2 A {} 23

    channels  15N 13C
    nuclei    15N 13C 13C 13C

    shift 1   0p      99p   0.19    103.01350343140321   -141.5746631993705   65.13327882351086
    shift 2   0p      -20p  0.43    -81.06377248255257    37.80482478676182   37.44093809450101
    shift 3   118.4p  -76p  0.90    -150.38505792335727  89.66822674355326   -24.463624969871375
    shift 4   -16.1p  -20p  0.43    -81.06377248255257    37.80482478676182   37.44093809450101

    dipole    1 2   1019.177373191048   0 63.761085493672105  113.83213979076521
```

```
    dipole    1 3   224.75204646817454  0 92.27944718252601   88.65551357209294
    dipole    1 4   207.87002195441818  0 75.88146104801265   149.7140672262098
    dipole    2 3   -2153.960746084526  0 61.21562695898275   -115.71997661790925
    dipole    2 4   -2119.03836757051   0 88.5024983502745    -0.5617060154408939
    dipole    3 4   -476.3048614125925  0 105.97921978418117  29.371944568430724

    jcoupling 1 2 -11 0 0 0 0 0
    jcoupling 2 3 55  0 0 0 0 0
    jcoupling 2 4 35  0 0 0 0 0
}
```

The optimisation procedure progresses in three levels of increasing complexity. Initially, the optimisation assumes ideal RF homogeneity and on-resonance conditions for the $^{15}$N and $^{13}$C nuclei involved in the transfer. This provides a good starting shapes for optimisations in the next level where time-modulated RF inhomogeneity is assumed. The input file is as follows.

```
# spinsys defined in an external file
source NCACOcCB.spinsys

par {
    spin_rate 16500
    # parallelization using MPI (mpi_exec)
    num_cores 1

    method              direct dsyev
    crystal_file        rep3_112.cry
    gamma_angles        1
    variable Nspins     4
    variable recalc     pow(2,2-Nspins)

    start_operator      I1x
    detect_operator     I2x
    proton_frequency    850e6
    sw                  1e6

    # Parameters for optimization - L-BFGS
    oc_grad_level       2
    oc_var_save_proc    rfstore
    # this MUST be used when working with optimal control!!!
    conjugate_fid       false
}

# procedure to store rf shape(s) during oc_optimize
proc rfstore {} {
    global par rfshN rfshC optname itercount fout tfcomponents

    incr itercount $par(oc_var_save_iter)
    save_shape $rfshN $optname\_N_temp_$itercount.dat
    save_shape $rfshC $optname\_C_temp_$itercount.dat
    puts $fout "Iter $itercount : $tfcomponents"
    flush $fout
}

# generates list of cp numbers distributed over +/-SW/2 range
proc get_lims {SWH cp} {
    if {$cp <= 1} {
        set Res 0
    } else {
        set step [expr double($SWH)/($cp-1)]
        set Res {}
        for {set i 0} {$i < $cp} {incr i} {
            set shft [expr double($SWH)/2.0-$i*$step]
            lappend Res $shft
        }
    }
    return $Res
}

proc pulseq_OC {} {
    global par rfshN rfshC

    maxdt $par(dt)
    reset
```

```
    pulse_shaped $par(duration) $rfshN $rfshC
    oc_acq_hermit
}

proc pulseq_OC_rotmod {} {
    global par rfshN rfshC

    maxdt $par(dt)
    reset
    pulse_shaped_rotormodulated $par(duration) $rfshN $rfshC
    oc_acq_hermit
}

proc gradient {} {
    global par rfshN rfshC tfcomponents

    set par(np) [expr [shape_len $rfshN] + [shape_len $rfshC] ]
    # looping over offset profiles is done in averaging_file
    set f [fsimpson]
    fscale $f -scale $par(recalc)
    oc_grad_add_energy_penalty $f $rfshN -$par(lamN) $rfshC -$par(lamC)
    set pen1 [expr $par(lamN)*[shape_energy $rfshN $par(duration)]]
    set pen2 [expr $par(lamC)*[shape_energy $rfshC $par(duration)]]
    set tfcomponents [list [expr $par(_phivals_)*$par(recalc)] $pen1 $pen2 ]
    return $f
}

proc target_function {} {
    global par rfshN rfshC

    set par(np) 1
    set f [fsimpson]
    set Res [expr [findex $f 1 -re]*$par(recalc) ]
    funload $f
    set pen1 [expr $par(lamN)*[shape_energy $rfshN $par(duration)]]
    set pen2 [expr $par(lamC)*[shape_energy $rfshC $par(duration)]]
    set Res [expr $Res - $pen1 - $pen2]
    return [format "%.20f" $Res]
}

proc prepare_ave {vals1 vals2 filename} {
    set fd [open $filename w]
    puts $fd "shift_1_iso shift_2_iso weight"
    set w [expr 1.0 / ([llength $vals1] * [llength $vals2]) ]
    foreach a $vals1 {
        foreach b $vals2 {
            puts $fd "[format "%8.2f" $a]p [format "%8.2f" $b]p [format "%12.8f" $w]"
        }
    }
    close $fd
}

proc main {} {
    global par rfshN rfshC optname itercount fout tfcomponents

    set number_of_rotor_periods 60
    set pulses_per_period  25
    set rfmax13C  40000
    set rfmax15N  30000
    set par(lamN) 3e-11
    set par(lamC) 1e-11
    set taur [expr 1.0e6/$par(spin_rate)]
    set par(duration) [expr $number_of_rotor_periods*$taur]
    set par(dt) [expr $taur/$pulses_per_period]
    set par(Nelem) [expr $number_of_rotor_periods*$pulses_per_period]

    puts "MAS frequency: $par(spin_rate) Hz"
    puts "pulses in one rotor period: $pulses_per_period"
    puts "duration: $par(duration)"
    puts "number of pulses: $par(Nelem)"
    puts "element length: $par(dt) us"
    puts "number of rotor periods: [expr $par(duration)/(1.0e6/$par(spin_rate))]"

    # level 1 (no rf inhomogeneity)
    set rfshN [rand_shape 5000 $par(Nelem) [expr int($number_of_rotor_periods/2)] ]
    set rfshC [rand_shape 5000 $par(Nelem) [expr int($number_of_rotor_periods/2)] ]
```

```
    set optname shp_lev1
    set tfcomponents {}
    set fout [open $optname\_output.txt w]
    set par(oc_var_save_iter) 20
    set par(pulse_sequence) pulseq_OC
    set itercount 0
    set par(oc_method) CG
    set par(oc_max_iter) 150
    set tfopt [oc_optimize $rfshN -max $rfmax15N $rfshC -max $rfmax13C]
    save_shape $rfshN $optname\_N_final.dat
    save_shape $rfshC $optname\_C_final.dat
    close $fout

    # level 2 (include spatial rf inhomogeneity)
    set optname shp_lev2
    set par(rfmap) coil_3p2_800MHz_N_C_detweights.dat
    set par(oc_var_save_iter) 10
    set fout [open $optname\_output.txt a]
    set par(pulse_sequence) pulseq_OC_rotmod
    set itercount 0
    set par(oc_method) CG
    set par(oc_max_iter) 1000
    set tfopt [oc_optimize $rfshN -max $rfmax15N $rfshC -max $rfmax13C]
    save_shape $rfshN $optname\_N_final.dat
    save_shape $rfshC $optname\_C_final.dat
    close $fout
    free_all_shapes
}
```

Finally, the resulting shapes are optimised for robustness over a range of chemical shifts, typical for amide and C$\alpha$ resonances in proteins. The full input file reads

```
# Broadband transfer, little RF energy penalty and hard RF limits
# Reads initial shapes from results of previous runs using
#  simpson nca_lev3.in 225
#                      225 is number of previous iteration

# spinsys defined in an external file
source NCACOcCB.spinsys

par {
    spin_rate 16500
    # parallelization using MPI (mpi_exec)
    num_cores 1

    method              direct dsyev
    crystal_file        rep3_112.cry
    gamma_angles        1
    variable Nspins     4
    variable recalc     pow(2,2-Nspins)

    start_operator      I1x
    detect_operator     I2x
    proton_frequency    850e6
    sw                  1e6

    # Parameters for optimization - L-BFGS
    oc_grad_level       2
    oc_var_save_proc    rfstore
    # this MUST be used when working with optimal control!!!
    conjugate_fid       false
}

# procedure to store rf shape(s) during oc_optimize
proc rfstore {} {
    global par rfshN rfshC optname itercount fout tfcomponents

    incr itercount $par(oc_var_save_iter)
    save_shape $rfshN $optname\_N_temp_$itercount.dat
    save_shape $rfshC $optname\_C_temp_$itercount.dat
    puts $fout "Iter $itercount : $tfcomponents"
    flush $fout
}
```

```
# generates list of cp numbers distributed over +/-SW/2 range
proc get_lims {SWH cp} {
    if {$cp <= 1} {
        set Res 0
    } else {
        set step [expr double($SWH)/($cp-1)]
        set Res {}
        for {set i 0} {$i < $cp} {incr i} {
            set shft [expr double($SWH)/2.0-$i*$step]
            lappend Res $shft
        }
    }
    return $Res
}

proc pulseq_OC_rotmod {} {
    global par rfshN rfshC

    maxdt $par(dt)
    reset
    pulse_shaped_rotormodulated $par(duration) $rfshN $rfshC
    oc_acq_hermit
}

proc gradient {} {
    global par rfshN rfshC tfcomponents

    set par(np) [expr [shape_len $rfshN] + [shape_len $rfshC] ]
    # looping over offset profiles is done in averaging_file
    set f [fsimpson]
    fscale $f -scale $par(recalc)
    oc_grad_add_energy_penalty $f $rfshN -$par(lamN) $rfshC -$par(lamC)
    set pen1 [expr $par(lamN)*[shape_energy $rfshN $par(duration)]]
    set pen2 [expr $par(lamC)*[shape_energy $rfshC $par(duration)]]
    set tfcomponents [list [expr $par(_phivals_)*$par(recalc)] $pen1 $pen2 ]
    return $f
}

proc target_function {} {
    global par rfshN rfshC

    set par(np) 1
    set f [fsimpson]
    set Res [expr [findex $f 1 -re]*$par(recalc) ]
    funload $f
    set pen1 [expr $par(lamN)*[shape_energy $rfshN $par(duration)]]
    set pen2 [expr $par(lamC)*[shape_energy $rfshC $par(duration)]]
    set Res [expr $Res - $pen1 - $pen2]
    return [format "%.20f" $Res]
}

proc prepare_ave {vals1 vals2 filename} {
    set fd [open $filename w]
    puts $fd "shift_1_iso shift_2_iso weight"
    set w [expr 1.0 / ([llength $vals1] * [llength $vals2]) ]
    foreach a $vals1 {
        foreach b $vals2 {
            puts $fd "[format "%8.2f" $a]p [format "%8.2f" $b]p [format "%12.8f" $w]"
        }
    }
    close $fd
}

proc main {} {
    global par rfshN rfshC optname itercount fout tfcomponents

    set number_of_rotor_periods 60
    set pulses_per_period  25
    set rfmax13C  40000
    set rfmax15N  30000
    set par(lamN) 3e-11
    set par(lamC) 1e-11
    set taur [expr 1.0e6/$par(spin_rate)]
    set par(duration) [expr $number_of_rotor_periods*$taur]
    set par(dt) [expr $taur/$pulses_per_period]
    set par(Nelem) [expr $number_of_rotor_periods*$pulses_per_period]
```

```
    # range of chemical shifts with control points
    set limsN [get_lims 26.8 3]
    set limsC [get_lims 25 5]

    set optname shp_lev3

    if {[llength $::argv] < 2} {
        set Nini 0
    } else {
        set Nini [lindex $::argv 1]
    }
    if {$Nini == 0} {
        set shapeininameN shp_lev2_N_final.dat
        set shapeininameC shp_lev2_C_final.dat
    } else {
        set shapeininameN $optname\_N_temp_${Nini}.dat
        set shapeininameC $optname\_C_temp_${Nini}.dat
    }
    set rfshN [load_shape $shapeininameN]
    set rfshC [load_shape $shapeininameC]
    set par(Nelem) [shape_len $rfshN]
    set taur [expr 1.0e6/$par(spin_rate)]
    set par(duration) [expr $number_of_rotor_periods*$taur]

    set tfcomponents {}
    set itercount $Nini
    set par(rfmap) coil_3p2_800MHz_N_C_detweights.dat
    set par(pulse_sequence) pulseq_OC_rotmod
    set par(averaging_file) $par(name).ave
    prepare_ave $limsN $limsC $par(averaging_file)
    set par(oc_var_save_iter) 5
    set fout [open $optname\_output.txt a]
    set par(oc_method) CG
    set par(oc_max_iter) 2000
    set tfopt [oc_optimize $rfshN -max $rfmax15N $rfshC -max $rfmax13C]
    save_shape $rfshN $optname\_N_final.dat
    save_shape $rfshC $optname\_C_final.dat
    close $fout
    free_all_shapes
}
```

For time-modulated RF inhomogeneity, a dataset defining $B_1$ field parameters ($x$- and $y$-components at different volume elements) is contained in the file `coil_3p2_800MHz_N_C_detweights.dat` which is listed below (line breaks in the listing are indicated by indentation):

```
21 2 91
0.0580128 6 0.442773 -0.00319435 0.564436 -0.196016 0.648825 -0.201133 0.655091 0.000655143 0.536485 0
    .189028 0.393987 0.178788 0.44231 -0.0031699 0.56383 -0.195844 0.648218 -0.200969 0.654553 0
    .000649118 0.536091 0.188894 0.393699 0.178681
0.0720874 6 0.560875 0.0224739 0.705408 -0.128776 0.792774 -0.143677 0.813989 0.0206696 0.697284 0
    .215611 0.525179 0.213355 0.560318 0.0224477 0.704678 -0.128774 0.79207 -0.143651 0.81335 0.0206307
     0.696781 0.215473 0.5248 0.213234
0.0815388 6 0.675095 0.0307884 0.775025 -0.0927908 0.84888 -0.0864887 0.880675 0.0297255 0.821033 0
    .175042 0.687936 0.191913 0.67452 0.0307366 0.774351 -0.0929049 0.848261 -0.0866036 0.880099 0
    .0296697 0.820496 0.174987 0.68746 0.191844
0.0917012 6 0.833612 0.02688 0.888282 -0.0538891 0.93413 -0.0597056 0.94159 0.0304462 0.88951 0.120328
    0.827099 0.115112 0.833052 0.0268278 0.887723 -0.0540657 0.933674 -0.0598789 0.941202 0.0303953 0
    .889105 0.120391 0.826626 0.115169
0.0978093 6 0.913159 0.0226382 0.932991 -0.0258517 0.960771 -0.0128396 0.973953 0.0298403 0.966919 0
    .0709986 0.93389 0.0781765 0.912795 0.0225851 0.93266 -0.0260572 0.96054 -0.0130422 0.973773 0
    .0297962 0.966695 0.0710926 0.933584 0.0782623
0.102345 6 0.966506 0.0209472 0.989198 0.0107604 1.00912 0.0115005 1.01842 0.0294779 0.998005 0.0601725
     0.9661 0.0525037 0.966343 0.0208989 0.989072 0.010603 1.00907 0.0113534 1.01841 0.0294462 0.997963
     0.0602491 0.96598 0.0525733
0.0520608 6 0.99698 0.0187711 1.00953 0.0295482 1.01514 0.0340338 1.02028 0.0275747 1.01353 0.0340338 0
    .99585 0.0295482 0.997024 0.0187246 1.00958 0.0295095 1.01519 0.0340062 1.02033 0.0275503 1.01358 0
    .0340062 0.995894 0.0295095
0.0345679 6 0.477677 -4.03363e-05 0.544296 -0.101943 0.597246 -0.102586 0.601766 0.00177668 0.539511 0
    .103743 0.466133 0.101182 0.477258 -2.81693e-05 0.543798 -0.101866 0.596739 -0.102515 0.601298 0
    .00177319 0.539117 0.103677 0.465784 0.101126
0.0420092 6 0.592014 0.0172509 0.662254 -0.074904 0.715159 -0.077048 0.72275 0.0166856 0.662347 0
    .117065 0.583126 0.117023 0.591522 0.0172288 0.661682 -0.0749014 0.714594 -0.0770443 0.722228 0
    .016656 0.66189 0.116996 0.58271 0.11696
```

```
0.0482525 6 0.699735 0.0269408 0.755659 -0.0492387 0.801856 -0.049077 0.812139 0.0261272 0.767186 0
    .109032 0.700513 0.111736 0.699219 0.0268957 0.755091 -0.0493033 0.801313 -0.0491413 0.811634 0
    .0260804 0.766715 0.108988 0.700058 0.111691
0.05467 6 0.821854 0.0290026 0.855984 -0.022449 0.888429 -0.0221185 0.895745 0.0303388 0.86614 0
    .0855935 0.824625 0.0855095 0.821378 0.0289489 0.8555 -0.0225653 0.887993 -0.0222338 0.895348 0
    .030287 0.865742 0.0855972 0.824197 0.0855105
0.0595607 6 0.915986 0.0256278 0.931986 -0.00273688 0.950767 8.87235e-05 0.956416 0.0294203 0.942872 0
    .0584874 0.92121 0.057798 0.915661 0.0255755 0.931677 -0.00286991 0.950513 -4.1618e-05 0.956194 0
    .0293737 0.94263 0.0585171 0.92092 0.0578242
0.0623889 6 0.970535 0.0220326 0.979677 0.0100301 0.989569 0.0122064 0.992047 0.0268898 0.983529 0
    .04111 0.971905 0.0385002 0.970388 0.0219854 0.97955 0.00992151 0.989485 0.0121029 0.991985 0
    .0268522 0.983447 0.0411327 0.971781 0.0385181
0.0318841 6 1.00172 0.0195352 1.005 0.0216645 1.00553 0.0242309 1.00412 0.0246853 1.00152 0.0242309 0
    .999653 0.0216645 1.00174 0.019491 1.00502 0.0216235 1.00555 0.0241962 1.00414 0.0246538 1.00154 0
    .0241962 0.999669 0.0216235
0.0115161 1 0.537098 0.00142532 0.536679 0.00142818
0.013867 1 0.646523 0.0153703 0.646053 0.0153469
0.0159487 1 0.74331 0.0249274 0.742832 0.0248847
0.0181601 1 0.84621 0.0295437 0.845793 0.0294913
0.0199373 1 0.928979 0.0280287 0.928707 0.0279786
0.0209529 1 0.976261 0.0247415 0.976146 0.024698
0.010729 1 0.999751 0.0222979 0.999752 0.022259
```
